# Supplementary material for: POPQORN: Quantifying Robustness of Recurrent Neural Networks
Source: arXiv:1905.07387 source file (2019-05-17)
Supplement: Supplementary file 1 [file appendix.pdf]

# Appendix[1]

# Contents


A. Theorems and Algorithms . . . 2
- A.1 Vanilla Recurrent Neural Network . . . 2
- A.2 Algorithms for Recurrent Neural Networks . . . 11
- A.3 Long Short-term Memory Network . . . 12
- A.4 Bounding Planes for 2D Nonlinear Activation Functions . . . 24
- A.5 Algorithms for Long Short-term Memory Networks . . . 26
- A.6 Long Short-term Memory Network (1D bounding lines) . . . 29
- A.7 Gated Recurrent Unit Network . . . 34

B. Experiments . . . 43
- B.1 Significance of plane (2D)-bounding POPQORN certificates . . . 43
- B.2 CLEVER-RNN Score . . . 44
- B.3 Adapted C&W Attack . . . 45
- B.4 Experimental Details . . . 46


[1] Supplementary materials of *POPQORN: Quantifying Robustness of Recurrent Neural Networks*. Copyright 2019 by the authors.

## A. Theorems and Algorithms

### A.1 Vanilla Recurrent Neural Network

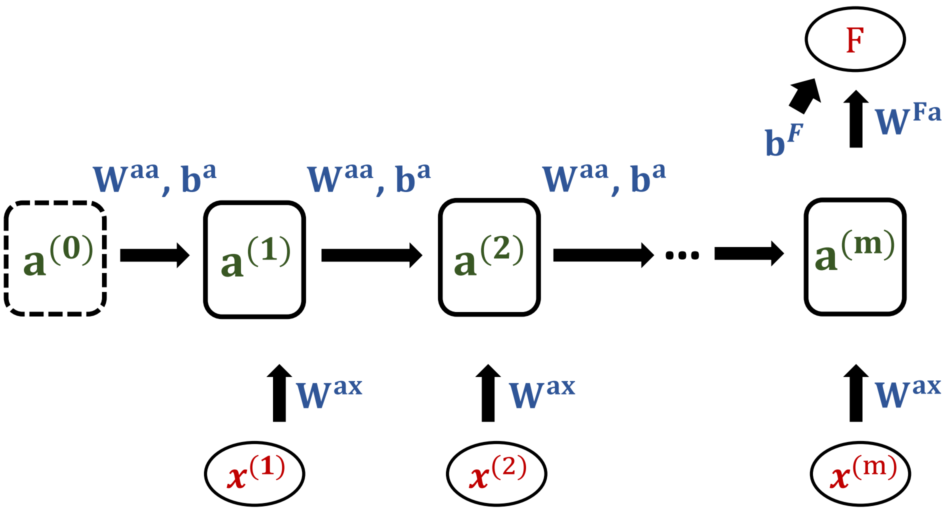


Figure 1: Graphical depiction of an $m$-th layer many-to-one recurrent neural network

**Theorem A. 1 (Explicit output bound of recurrent neural network F)** *Given an $m$-layer recurrent neural network $F : \mathbb{R}^{n\times m} \to \mathbb{R}^t$, there exists two explicit functions $F_j^L : \mathbb{R}^{n\times m} \to \mathbb{R}$ and $F_j^U : \mathbb{R}^{n\times m} \to \mathbb{R}$ such that $\forall\, j \in [t]$ and $\forall\, \mathbf{X} \in \mathbb{R}^{n\times m}$ where $\mathbf{x}^{(k)} \in \mathbb{B}_p(\mathbf{x}_0^{(k)}, \epsilon)$, the inequity $F_j^L(\mathbf{X}) \leq F_j(\mathbf{X}) \leq F_j^U(\mathbf{X})$ holds true, where*

$$F_j^U(\mathbf{X}) = \mathbf{\Lambda}_{j,:}^{(0)}\mathbf{a}^{(0)} + \sum_{k=1}^{m} \mathbf{\Lambda}_{j,:}^{(k)}\mathbf{W}^{ax}\mathbf{x}^{(k)} + \sum_{k=1}^{m} \mathbf{\Lambda}_{j,:}^{(k)}(\mathbf{b}^a + \mathbf{\Delta}_{:,j}^{(k)}) + \mathbf{b}_j^F,$$
$$F_j^L(\mathbf{X}) = \mathbf{\Omega}_{j,:}^{(0)}\mathbf{a}^{(0)} + \sum_{k=1}^{m} \mathbf{\Omega}_{j,:}^{(k)}\mathbf{W}^{ax}\mathbf{x}^{(k)} + \sum_{k=1}^{m} \mathbf{\Omega}_{j,:}^{(k)}(\mathbf{b}^a + \mathbf{\Theta}_{:,j}^{(k)}) + \mathbf{b}_j^F,$$

$$\mathbf{\Lambda}_{j,:}^{(k-1)} = \begin{cases} \mathbf{W}_{j,:}^{Fa} \odot \lambda_{j,:}^{(k-1)} & \text{if} \quad k = m+1; \\ (\mathbf{\Lambda}_{j,:}^{(k)}\mathbf{W}^{aa}) \odot \lambda_{j,:}^{(k-1)} & \text{if} \quad k \in [m]; \end{cases} \quad \mathbf{\Omega}_{j,:}^{(k-1)} = \begin{cases} \mathbf{W}_{j,:}^{Fa} \odot \omega_{j,:}^{(k-1)} & \text{if} \quad k = m+1; \\ (\mathbf{\Omega}_{j,:}^{(k)}\mathbf{W}^{aa}) \odot \omega_{j,:}^{(k-1)} & \text{if} \quad k \in [m]; \end{cases}$$

*and* $\forall r \in s$,

$$\lambda_{j,i}^{(m)} = \begin{cases} \alpha_{U,i}^{(m)} & \text{if} \;\; \mathbf{W}_{j,i}^{Fa} \geq 0; \\ \alpha_{L,i}^{(m)} & \text{if} \;\; \mathbf{W}_{j,i}^{Fa} < 0; \end{cases} \qquad \mathbf{\Delta}_{i,j}^{(m)} = \begin{cases} \beta_{U,i}^{(m)} & \text{if} \;\; \mathbf{W}_{j,i}^{Fa} \geq 0; \\ \beta_{L,i}^{(m)} & \text{if} \;\; \mathbf{W}_{j,i}^{Fa} < 0; \end{cases}$$
$$\omega_{j,r}^{(m)} = \begin{cases} \alpha_{L,i}^{(m)} & \text{if} \;\; \mathbf{W}_{j,i}^{Fa} \geq 0; \\ \alpha_{U,i}^{(m)} & \text{if} \;\; \mathbf{W}_{j,i}^{Fa} < 0; \end{cases} \qquad \mathbf{\Theta}_{r,j}^{(m)} = \begin{cases} \beta_{L,i}^{(m)} & \text{if} \;\; \mathbf{W}_{j,i}^{Fa} \geq 0; \\ \beta_{U,i}^{(m)} & \text{if} \;\; \mathbf{W}_{j,i}^{Fa} < 0; \end{cases}$$

*and* $\forall r \in s, k \in [m-1]$,

$$\lambda_{j,r}^{(k)} = \begin{cases} \alpha_{U,r}^{(k)} & \text{if} \quad \tilde{\mathbf{W}}_{j,r}^{aa(k+1)} \geq 0 \quad (\Longleftrightarrow \mathbf{\Lambda}_{j,:}^{(k+1)}\mathbf{W}_{:,r}^{aa} \geq 0); \\ \alpha_{L,r}^{(k)} & \text{if} \quad \tilde{\mathbf{W}}_{j,r}^{aa(k+1)} < 0 \quad (\Longleftrightarrow \mathbf{\Lambda}_{j,:}^{(k+1)}\mathbf{W}_{:,r}^{aa} < 0); \end{cases}$$
$$\omega_{j,r}^{(k)} = \begin{cases} \alpha_{L,r}^{(k)} & \text{if} \quad \tilde{\mathbf{W}}_{j,r}^{aa(k+1)} \geq 0 \quad (\Longleftrightarrow \mathbf{\Omega}_{j,:}^{(k+1)}\mathbf{W}_{:,r}^{aa} \geq 0); \\ \alpha_{U,r}^{(k)} & \text{if} \quad \tilde{\mathbf{W}}_{j,r}^{aa(k+1)} < 0 \quad (\Longleftrightarrow \mathbf{\Omega}_{j,:}^{(k+1)}\mathbf{W}_{:,r}^{aa} < 0); \end{cases}$$

$$\mathbf{\Delta}_{r,j}^{(k)} = \begin{cases} \beta_{U,r}^{(k)} & \textit{if} \quad \tilde{\mathbf{W}}_{j,r}^{aa(k+1)} \geq 0 \quad (\Longleftrightarrow \mathbf{\Lambda}_{j,:}^{(k+1)} \mathbf{W}_{:,r}^{aa} \geq 0); \\ \beta_{L,r}^{(k)} & \textit{if} \quad \tilde{\mathbf{W}}_{j,r}^{aa(k+1)} < 0 \quad (\Longleftrightarrow \mathbf{\Lambda}_{j,:}^{(k+1)} \mathbf{W}_{:,r}^{aa} < 0); \end{cases}$$

$$\mathbf{\Theta}_{r,j}^{(k)} = \begin{cases} \beta_{L,r}^{(k)} & \textit{if} \quad \tilde{\mathbf{W}}_{j,r}^{aa(k+1)} \geq 0 \quad (\Longleftrightarrow \mathbf{\Omega}_{j,:}^{(k+1)} \mathbf{W}_{:,r}^{aa} \geq 0); \\ \beta_{U,r}^{(k)} & \textit{if} \quad \tilde{\mathbf{W}}_{j,r}^{aa(k+1)} < 0 \quad (\Longleftrightarrow \mathbf{\Omega}_{j,:}^{(k+1)} \mathbf{W}_{:,r}^{aa} < 0); \end{cases}$$

*and* $\forall r \in s, \lambda_{j,r}^{(0)} = \omega_{j,r}^{(0)} = 1$, *where* $\odot$ *is the Hadamard product.*

***Proof 1*** *Given an* $m$*-layer recurrent neural network* $F : \mathbb{R}^{n \times m} \rightarrow \mathbb{R}^t$ *with pre-activation bounds* $\mathbf{l}^{(k)}$ *and* $\mathbf{u}^{(k)}$ *for* $\mathbf{X} \in \mathbb{R}^{n \times m}$*, where* $\mathbf{x}^{(k)} \in \mathbb{B}_p(\mathbf{x}_0^{(k)}, \epsilon)$*, let the pre-activation inputs for the* $j$*-th neuron at the output layer be* $F_j(\mathbf{X}) = \mathbf{W}_{j,:}^{Fa} \mathbf{a}^{(m)} + \mathbf{b}_j^F$*. The* $j$*-th output of the recurrent neural network is the following:*

$$\begin{aligned} F_j(\mathbf{X}) &= \mathbf{W}_{j,:}^{Fa} \mathbf{a}^{(m)} + \mathbf{b}_j^F, \quad (1) \\ &= \sum_{i=1}^{s} \mathbf{W}_{j,i}^{Fa} \mathbf{a}_i^{(m)} + \mathbf{b}_j^F, \\ &= \sum_{i=1}^{s} \mathbf{W}_{j,i}^{Fa} \sigma(\mathbf{y}_i^{(m)}) + \mathbf{b}_j^F, \\ &= \sum_{\mathbf{W}_{j,i}^{Fa} \geq 0} \mathbf{W}_{j,i}^{Fa} \sigma(\mathbf{y}_i^{(m)}) + \sum_{\mathbf{W}_{j,i}^{Fa} < 0} \mathbf{W}_{j,i}^{Fa} \sigma(\mathbf{y}_i^{(m)}) + \mathbf{b}_j^F. \quad (2) \end{aligned}$$

*Assume the activation function* $\sigma(\mathbf{y})$ *is bounded by two linear functions* $h_{L,i}^{(m)}(\mathbf{y})$ *and* $h_{U,i}^{(m)}(\mathbf{y})$*, we have*

$$h_{L,i}^{(m)}(\mathbf{y}_i^{(m)}) \leq \sigma(\mathbf{y}_i^{(m)}) \leq h_{U,i}^{(m)}(\mathbf{y}_i^{(m)}).$$

*Thus, if the associated weight* $\mathbf{W}_{j,i}^{Fa}$ *to the* $i$*-th neuron is non-negative, we have*

$$\mathbf{W}_{j,i}^{Fa} \cdot h_{L,i}^{(m)}(\mathbf{y}_i^{(m)}) \leq \mathbf{W}_{j,i}^{Fa} \sigma(\mathbf{y}_i^{(m)}) \leq \mathbf{W}_{j,i}^{Fa} \cdot h_{U,i}^{(m)}(\mathbf{y}_i^{(m)}); \quad (3)$$

*otherwise, we have*

$$\mathbf{W}_{j,i}^{Fa} \cdot h_{U,i}^{(m)}(\mathbf{y}_i^{(m)}) \leq \mathbf{W}_{j,i}^{Fa} \sigma(\mathbf{y}_i^{(m)}) \leq \mathbf{W}_{j,i}^{Fa} \cdot h_{L,i}^{(m)}(\mathbf{y}_i^{(m)}). \quad (4)$$

***Upper bound.*** *By using the right-hand side of Inequity* (3) *and Inequity* (4) *in Equation* (2)*, we obtain an upper bound*

$$\begin{aligned} F_j^{U,m}(\mathbf{X}) = &\sum_{\mathbf{W}_{j,i}^{Fa} \geq 0} \mathbf{W}_{j,i}^{Fa} \ \alpha_{U,i}^{(m)}(\mathbf{y}_i^{(m)} + \beta_{U,i}^{(m)}) \\ &+ \sum_{\mathbf{W}_{j,i}^{Fa} < 0} \mathbf{W}_{j,i}^{Fa} \ \alpha_{L,i}^{(m)}(\mathbf{y}_i^{(m)} + \beta_{L,i}^{(m)}) + \mathbf{b}_j^F. \end{aligned}$$

*We use variables* $\lambda_{j,i}^{(m)}$ *and* $\mathbf{\Delta}_{i,j}^{(m)}$ *to denote the slops in front of* $\mathbf{y}_i^{(m)}$ *and intercepts in the parentheses:*

$$\lambda_{j,i}^{(m)} = \begin{cases} \alpha_{U,i}^{(m)} & \textit{if} \ \mathbf{W}_{j,i}^{Fa} \geq 0; \\ \alpha_{L,i}^{(m)} & \textit{if} \ \mathbf{W}_{j,i}^{Fa} < 0; \end{cases}$$

$$\mathbf{\Delta}_{i,j}^{(m)} = \begin{cases} \beta_{U,i}^{(m)} & \textit{if} \ \mathbf{W}_{j,i}^{Fa} \geq 0; \\ \beta_{L,i}^{(m)} & \textit{if} \ \mathbf{W}_{j,i}^{Fa} < 0; \end{cases}$$

*and obtain*

$$F_j^{U,m}(\mathbf{X}) = \sum_{i=1}^{s} \mathbf{W}_{j,i}^{Fa} \ \lambda_{j,i}^{(m)}(\mathbf{y}_i^{(m)} + \mathbf{\Delta}_{i,j}^{(m)}) + \mathbf{b}_j^F.$$

*We further let* $\mathbf{\Lambda}_{j,i}^{(m)} := \mathbf{W}_{j,i}^{Fa}\ \lambda_{j,i}^{(m)}$ *and we have*

$$\begin{aligned}
F_j^{U,m}(\mathbf{X}) &= \sum_{i=1}^{s} \mathbf{\Lambda}_{j,i}^{(m)}(\mathbf{y}_i^{(m)} + \mathbf{\Delta}_{i,j}^{(m)}) + \mathbf{b}_j^F, \\
&= \sum_{i=1}^{s} \mathbf{\Lambda}_{j,i}^{(m)}(\mathbf{W}_{i,:}^{aa}\mathbf{a}^{(m-1)} + \mathbf{W}_{i,:}^{ax}\mathbf{x}^{(m)} + \mathbf{b}_i^a + \mathbf{\Delta}_{i,j}^{(m)}) + \mathbf{b}_j^F, \\
&= \sum_{i=1}^{s} \mathbf{\Lambda}_{j,i}^{(m)}(\sum_{r=1}^{s}\mathbf{W}_{i,r}^{aa}\mathbf{a}_r^{(m-1)} + \sum_{q_m=1}^{n}\mathbf{W}_{i,q_m}^{ax}\mathbf{x}_{q_m}^{(m)} + \mathbf{b}_i^a + \mathbf{\Delta}_{i,j}^{(m)}) + \mathbf{b}_j^F, \\
&= \sum_{r=1}^{s}(\sum_{i=1}^{s}\mathbf{\Lambda}_{j,i}^{(m)}\mathbf{W}_{i,r}^{aa})\mathbf{a}_r^{(m-1)} + \sum_{q_m=1}^{n}(\sum_{i=1}^{s}\mathbf{\Lambda}_{j,i}^{(m)}\mathbf{W}_{i,q_m}^{ax})\mathbf{x}_{q_m}^{(m)} \\
&+ \sum_{i=1}^{s}\mathbf{\Lambda}_{j,i}^{(m)}(\mathbf{b}_i^a + \mathbf{\Delta}_{i,j}^{(m)}) + \mathbf{b}_j^F. \qquad (5)
\end{aligned}$$

*We combine coefficients in Equation* (5) *into equivalent weights* $\tilde{\mathbf{W}}_{j,r}^{aa(m)}$, $\tilde{\mathbf{W}}_{j,q_m}^{ax(m)}$ *and bias* $\tilde{b}_j^{(m)}$ *as defined by*

$$\begin{aligned}
\tilde{\mathbf{W}}_{j,r}^{aa(m)} &= \sum_{i=1}^{s}\mathbf{\Lambda}_{j,i}^{(m)}\mathbf{W}_{i,r}^{aa} = \mathbf{\Lambda}_{j,:}^{(m)}\mathbf{W}_{:,r}^{aa}, \\
\tilde{\mathbf{W}}_{j,q_m}^{ax(m)} &= \sum_{i=1}^{s}\mathbf{\Lambda}_{j,i}^{(m)}\mathbf{W}_{i,q_m}^{ax} = \mathbf{\Lambda}_{j,:}^{(m)}\mathbf{W}_{:,q_m}^{ax}, \\
\tilde{\mathbf{b}}_j^{(m)} &= \sum_{i=1}^{s}\mathbf{\Lambda}_{j,i}^{(m)}(\mathbf{b}_i^a + \mathbf{\Delta}_{i,j}^{(m)}) + \mathbf{b}_j^F = \mathbf{\Lambda}_{j,:}^{(m)}(\mathbf{b}^a + \mathbf{\Delta}_{:,j}^{(m)}) + \mathbf{b}_j^F,
\end{aligned}$$

*and obtain*

$$\begin{aligned}
F_j^{U,m}(\mathbf{X}) &= \sum_{r=1}^{s}\tilde{\mathbf{W}}_{j,r}^{aa(m)}\mathbf{a}_r^{(m-1)} + \sum_{q_m=1}^{n}\tilde{\mathbf{W}}_{j,q_m}^{ax(m)}\mathbf{x}_{q_m}^{(m)} + \tilde{\mathbf{b}}_j^{(m)}, \qquad (6) \\
&= \sum_{r=1}^{s}\tilde{\mathbf{W}}_{j,r}^{aa(m)}\sigma(\mathbf{y}_r^{(m-1)}) + \sum_{q_m=1}^{n}\tilde{\mathbf{W}}_{j,q_m}^{ax(m)}\mathbf{x}_{q_m}^{(m)} + \tilde{\mathbf{b}}_j^{(m)}, \\
&= \sum_{\tilde{\mathbf{W}}_{j,r}^{aa(m)}\geq 0}\tilde{\mathbf{W}}_{j,r}^{aa(m)}\sigma(\mathbf{y}_r^{(m-1)}) + \sum_{\tilde{\mathbf{W}}_{j,r}^{aa(m)}<0}\tilde{\mathbf{W}}_{j,r}^{aa(m)}\sigma(\mathbf{y}_r^{(m-1)}) + \sum_{q_m=1}^{n}\tilde{\mathbf{W}}_{j,q_m}^{ax(m)}\mathbf{x}_{q_m}^{(m)} + \tilde{\mathbf{b}}_j^{(m)}. \qquad (7)
\end{aligned}$$

*Assume the activation unction* $\sigma(\mathbf{y})$ *is bounded by two linear functions* $h_{L,r}^{(m-1)}(\mathbf{y})$ *and* $h_{U,r}^{(m-1)}(\mathbf{y})$, *we have*

$$h_{L,r}^{(m-1)}(\mathbf{y}_r^{(m-1)}) \leq \sigma(\mathbf{y}_r^{(m-1)}) \leq h_{U,r}^{(m-1)}(\mathbf{y}_r^{(m-1)}).$$

*Thus, if the associated weight* $\tilde{\mathbf{W}}_{j,r}^{aa(m)}$ *to the* $r$*-th neuron is non-negative, we have*

$$\tilde{\mathbf{W}}_{j,r}^{aa(m)} \cdot h_{L,r}^{(m-1)}(\mathbf{y}_r^{(m-1)}) \leq \tilde{\mathbf{W}}_{j,r}^{aa(m)}\sigma(\mathbf{y}_r^{(m-1)}) \leq \tilde{\mathbf{W}}_{j,r}^{aa(m)} \cdot h_{U,r}^{(m-1)}(\mathbf{y}_r^{(m-1)}); \qquad (8)$$

*otherwise, we have*

$$\tilde{\mathbf{W}}_{j,r}^{aa(m)} \cdot h_{U,r}^{(m-1)}(\mathbf{y}_r^{(m-1)}) \leq \tilde{\mathbf{W}}_{j,r}^{aa(m)}\sigma(\mathbf{y}_r^{(m-1)}) \leq \tilde{\mathbf{W}}_{j,r}^{aa(m)} \cdot h_{L,r}^{(m-1)}(\mathbf{y}_r^{(m-1)}). \qquad (9)$$

*By using the right-hand side of Inequity* (8) *and Inequity* (9) *in Equation* (7), *an upper bound can be obtained similarly as*

$$\begin{aligned}
F_j^{U,m-1}(\mathbf{X}) = &\sum_{\tilde{\mathbf{W}}_{j,r}^{aa(m)}\geq 0}\tilde{\mathbf{W}}_{j,r}^{aa(m)}\ \alpha_{U,r}^{(m-1)}(\mathbf{y}_r^{(m-1)} + \beta_{U,r}^{(m-1)}) \\
&+ \sum_{\tilde{\mathbf{W}}_{j,r}^{aa(m)}<0}\tilde{\mathbf{W}}_{j,r}^{aa(m)}\ \alpha_{L,r}^{(m-1)}(\mathbf{y}_r^{(m-1)} + \beta_{L,r}^{(m-1)}) + \sum_{q_m=1}^{n}\tilde{\mathbf{W}}_{j,q_m}^{ax(m)}\mathbf{x}_{q_m}^{(m)} + \tilde{\mathbf{b}}_j^{(m)}.
\end{aligned}$$

*We use variables $\lambda_{j,r}^{(m-1)}$ and $\mathbf{\Delta}_{r,j}^{(m-1)}$ to denote the slops in front of $\mathbf{y}_r^{(m-1)}$ and intercepts in the parentheses:*

$$\lambda_{j,r}^{(m-1)} = \begin{cases} \alpha_{U,r}^{(m-1)} & \text{if} \quad \tilde{\mathbf{W}}_{j,r}^{aa(m)} \geq 0 \quad (\Longleftrightarrow \mathbf{\Lambda}_{j,:}^{(m)}\mathbf{W}_{:,r}^{aa} \geq 0); \\ \alpha_{L,r}^{(m-1)} & \text{if} \quad \tilde{\mathbf{W}}_{j,r}^{aa(m)} < 0 \quad (\Longleftrightarrow \mathbf{\Lambda}_{j,:}^{(m)}\mathbf{W}_{:,r}^{aa} < 0); \end{cases}$$

$$\mathbf{\Delta}_{r,j}^{(m-1)} = \begin{cases} \beta_{U,r}^{(m-1)} & \text{if} \quad \tilde{\mathbf{W}}_{j,r}^{aa(m)} \geq 0 \quad (\Longleftrightarrow \mathbf{\Lambda}_{j,:}^{(m)}\mathbf{W}_{:,r}^{aa} \geq 0); \\ \beta_{L,r}^{(m-1)} & \text{if} \quad \tilde{\mathbf{W}}_{j,r}^{aa(m)} < 0 \quad (\Longleftrightarrow \mathbf{\Lambda}_{j,:}^{(m)}\mathbf{W}_{:,r}^{aa} < 0); \end{cases}$$

*and obtain*

$$F_j^{U,m-1}(\mathbf{X}) = \sum_{r=1}^{s} \tilde{\mathbf{W}}_{j,r}^{aa(m)} \, \lambda_{j,r}^{(m-1)}(\mathbf{y}_r^{(m-1)} + \mathbf{\Delta}_{r,j}^{(m-1)}) + \sum_{q_m=1}^{n} \tilde{\mathbf{W}}_{j,q_m}^{ax(m)} \mathbf{x}_{q_m}^{(m)} + \tilde{\mathbf{b}}_j^{(m)}.$$

*We further let $\mathbf{\Lambda}_{j,r}^{(m-1)} := \tilde{\mathbf{W}}_{j,r}^{aa(m)} \, \lambda_{j,r}^{(m-1)}$ and we have*

$$\begin{aligned} F_j^{U,m-1}(\mathbf{X}) &= \sum_{r=1}^{s} \mathbf{\Lambda}_{j,r}^{(m-1)}(\mathbf{y}_r^{(m-1)} + \mathbf{\Delta}_{r,j}^{(m-1)}) + \sum_{q_m=1}^{n} \tilde{\mathbf{W}}_{j,q_m}^{ax(m)} \mathbf{x}_{q_m}^{(m)} + \tilde{\mathbf{b}}_j^{(m)}, \\ &= \sum_{r=1}^{s} \mathbf{\Lambda}_{j,r}^{(m-1)}(\mathbf{W}_{r,:}^{aa}\mathbf{a}^{(m-2)} + \mathbf{W}_{r,:}^{ax}\mathbf{x}^{(m-1)} + \mathbf{b}_r^{a} + \mathbf{\Delta}_{r,j}^{(m-1)}) + \sum_{q_m=1}^{n} \tilde{\mathbf{W}}_{j,q_m}^{ax(m)} \mathbf{x}_{q_m}^{(m)} + \tilde{\mathbf{b}}_j^{(m)}, \\ &= \sum_{r=1}^{s} \mathbf{\Lambda}_{j,r}^{(m-1)}(\sum_{i=1}^{s} \mathbf{W}_{r,i}^{aa}\mathbf{a}_i^{(m-2)} + \sum_{q_{m-1}=1}^{n} \mathbf{W}_{r,q_{m-1}}^{ax}\mathbf{x}_{q_{m-1}}^{(m-1)} + \mathbf{b}_r^{a} + \mathbf{\Delta}_{r,j}^{(m-1)}) \\ &+ \sum_{q_m=1}^{n} \tilde{\mathbf{W}}_{j,q_m}^{ax(m)} \mathbf{x}_{q_m}^{(m)} + \tilde{\mathbf{b}}_j^{(m)}, \\ &= \sum_{i=1}^{s}(\sum_{r=1}^{s} \mathbf{\Lambda}_{j,r}^{(m-1)}\mathbf{W}_{r,i}^{aa})\mathbf{a}_i^{(m-2)} + \sum_{q_{m-1}=1}^{n}(\sum_{r=1}^{s} \mathbf{\Lambda}_{j,r}^{(m-1)}\mathbf{W}_{r,q_{m-1}}^{ax})\mathbf{x}_{q_{m-1}}^{(m-1)} \\ &+ \sum_{r=1}^{s} \mathbf{\Lambda}_{j,r}^{(m-1)}(\mathbf{b}_r^{a} + \mathbf{\Delta}_{r,j}^{(m-1)}) + \sum_{q_m=1}^{n} \tilde{\mathbf{W}}_{j,q_m}^{ax(m)} \mathbf{x}_{q_m}^{(m)} + \tilde{\mathbf{b}}_j^{(m)}. \end{aligned} \tag{10}$$

*We combine coefficients in Equation* (10) *into equivalent weights $\tilde{\mathbf{W}}_{j,i}^{aa(m-1)}$, $\tilde{\mathbf{W}}_{j,q_{m-1}}^{ax(m-1)}$ and bias $\tilde{\mathbf{b}}_j^{(m-1)}$ as defined by*

$$\begin{aligned} \tilde{\mathbf{W}}_{j,i}^{aa(m-1)} &= \sum_{r=1}^{s} \mathbf{\Lambda}_{j,r}^{(m-1)}\mathbf{W}_{r,i}^{aa} = \mathbf{\Lambda}_{j,:}^{(m-1)}\mathbf{W}_{:,i}^{aa}, \\ \tilde{\mathbf{W}}_{j,q_{m-1}}^{ax(m-1)} &= \sum_{r=1}^{s} \mathbf{\Lambda}_{j,r}^{(m-1)}\mathbf{W}_{r,q_{m-1}}^{ax} = \mathbf{\Lambda}_{j,:}^{(m-1)}\mathbf{W}_{:,q_{m-1}}^{ax}, \\ \tilde{\mathbf{b}}_j^{(m-1)} &= \sum_{r=1}^{s} \mathbf{\Lambda}_{j,r}^{(m-1)}(\mathbf{b}_r^{a} + \mathbf{\Delta}_{r,j}^{(m-1)}) + \tilde{\mathbf{b}}_j^{(m)} = \mathbf{\Lambda}_{j,:}^{(m-1)}(\mathbf{b}^{a} + \mathbf{\Delta}_{:,j}^{(m-1)}) + \tilde{\mathbf{b}}_j^{(m)}, \end{aligned}$$

*and obtain*

$$F_j^{U,m-1}(\mathbf{X}) = \sum_{i=1}^{s} \tilde{\mathbf{W}}_{j,i}^{aa(m-1)}\mathbf{a}_i^{(m-2)} + \sum_{q_{m-1}=1}^{n} \tilde{\mathbf{W}}_{j,q_{m-1}}^{ax(m-1)}\mathbf{x}_{q_{m-1}}^{(m-1)} + \sum_{q_m=1}^{n} \tilde{\mathbf{W}}_{j,q_m}^{ax(m)} \mathbf{x}_{q_m}^{(m)} + \tilde{\mathbf{b}}_j^{(m-1)}. \tag{11}$$

*Notice that Equation* (6) *and Equation* (11) *are in similar forms. Thus, we can repeat the above procedure iteratively until we obtain the final upper bound $F_j^{U,1}(\mathbf{X})$, where $F_j(\mathbf{X}) \leq F_j^{U,F}(\mathbf{X}) \leq F_j^{U,m}(\mathbf{X}) \leq \cdots \leq F_j^{U,1}(\mathbf{X})$. We let $F_j^{U}(\mathbf{X})$ denote the final upper bound $F_j^{U,1}(\mathbf{X})$, and we have*

$$F_j^{U}(\mathbf{X}) = \mathbf{\Lambda}_{j,:}^{(0)}\mathbf{a}^{(0)} + \sum_{k=1}^{m} \mathbf{\Lambda}_{j,:}^{(k)}\mathbf{W}^{ax}\mathbf{x}^{(k)} + \sum_{k=1}^{m} \mathbf{\Lambda}_{j,:}^{(k)}(\mathbf{b}^{a} + \mathbf{\Delta}_{:,j}^{(k)}) + \mathbf{b}_j^{F},$$

*and ($\odot$ is the Hadamard product)*

$$\mathbf{\Lambda}^{(k-1)}_{j,:} = \begin{cases} \mathbf{W}^{Fa}_{j,:} \odot \lambda^{(k-1)}_{j,:} & \textit{if} \quad k = m+1; \\ (\mathbf{\Lambda}^{(k)}_{j,:}\mathbf{W}^{aa}) \odot \lambda^{(k-1)}_{j,:} & \textit{if} \quad k \in [m]; \end{cases}$$

*and* $\forall r \in s$,

$$\lambda^{(m)}_{j,i} = \begin{cases} \alpha^{(m)}_{U,i} & \textit{if} \;\; \mathbf{W}^{Fa}_{j,i} \geq 0; \\ \alpha^{(m)}_{L,i} & \textit{if} \;\; \mathbf{W}^{Fa}_{j,i} < 0; \end{cases}$$

$$\mathbf{\Delta}^{(m)}_{i,j} = \begin{cases} \beta^{(m)}_{U,i} & \textit{if} \;\; \mathbf{W}^{Fa}_{j,i} \geq 0; \\ \beta^{(m)}_{L,i} & \textit{if} \;\; \mathbf{W}^{Fa}_{j,i} < 0; \end{cases}$$

*and* $\forall r \in s, k \in [m-1]$,

$$\lambda^{(k)}_{j,r} = \begin{cases} \alpha^{(k)}_{U,r} & \textit{if} \;\; \tilde{\mathbf{W}}^{aa(k+1)}_{j,r} \geq 0 \quad (\Longleftrightarrow \mathbf{\Lambda}^{(k+1)}_{j,:}\mathbf{W}^{aa}_{:,r} \geq 0); \\ \alpha^{(k)}_{L,r} & \textit{if} \;\; \tilde{\mathbf{W}}^{aa(k+1)}_{j,r} < 0 \quad (\Longleftrightarrow \mathbf{\Lambda}^{(k+1)}_{j,:}\mathbf{W}^{aa}_{:,r} < 0); \end{cases}$$

$$\mathbf{\Delta}^{(k)}_{r,j} = \begin{cases} \beta^{(k)}_{U,r} & \textit{if} \;\; \tilde{\mathbf{W}}^{aa(k+1)}_{j,r} \geq 0 \quad (\Longleftrightarrow \mathbf{\Lambda}^{(k+1)}_{j,:}\mathbf{W}^{aa}_{:,r} \geq 0); \\ \beta^{(k)}_{L,r} & \textit{if} \;\; \tilde{\mathbf{W}}^{aa(k+1)}_{j,r} < 0 \quad (\Longleftrightarrow \mathbf{\Lambda}^{(k+1)}_{j,:}\mathbf{W}^{aa}_{:,r} < 0); \end{cases}$$

*and* $\forall r \in s, \lambda^{(0)}_{j,r} = 1$.

***Lower bound.*** *The above derivations of upper bound can be applied similarly to derive lower bounds of $F_j(\mathbf{X})$, and the only difference is now we need to use the left-hand side of Inequity* (3), (4), (8), (9) *(rather than right-hand side when deriving upper bound) to bound the terms in* (2) *and* (7). *Thus, following the same procedure in deriving the upper bounds, we can iteratively unwrap the activation functions and obtain a final lower bound $F^{L,1}_j(\mathbf{X})$, where $F_j(\mathbf{X}) \geq F^{L,F}_j(\mathbf{X}) \geq F^{L,m}_j(\mathbf{X}) \geq \cdots \geq F^{L,1}_j(\mathbf{X})$. We let $F^L_j(\mathbf{X})$ denote the final lower bound $F^{L,1}_j(\mathbf{X})$, and we have*

$$F^L_j(\mathbf{X}) = \mathbf{\Omega}^{(0)}_{j,:}\mathbf{a}^{(0)} + \sum_{k=1}^{m} \mathbf{\Omega}^{(k)}_{j,:}\mathbf{W}^{ax}\mathbf{x}^{(k)} + \sum_{k=1}^{m} \mathbf{\Omega}^{(k)}_{j,:}(\mathbf{b}^a + \mathbf{\Theta}^{(k)}_{:,j}) + \mathbf{b}^F_j,$$

*and ($\odot$ is the Hadamard product)*

$$\mathbf{\Omega}^{(k-1)}_{j,:} = \begin{cases} \mathbf{W}^{Fa}_{j,:} \odot \omega^{(k-1)}_{j,:} & \textit{if} \quad k = m+1; \\ (\mathbf{\Omega}^{(k)}_{j,:}\mathbf{W}^{aa}) \odot \omega^{(k-1)}_{j,:} & \textit{if} \quad k \in [m]; \end{cases}$$

*and* $\forall r \in s$,

$$\omega^{(m)}_{j,r} = \begin{cases} \alpha^{(m)}_{L,i} & \textit{if} \;\; \mathbf{W}^{Fa}_{j,i} \geq 0; \\ \alpha^{(m)}_{U,i} & \textit{if} \;\; \mathbf{W}^{Fa}_{j,i} < 0; \end{cases}$$

$$\mathbf{\Theta}^{(m)}_{r,j} = \begin{cases} \beta^{(m)}_{L,i} & \textit{if} \;\; \mathbf{W}^{Fa}_{j,i} \geq 0; \\ \beta^{(m)}_{U,i} & \textit{if} \;\; \mathbf{W}^{Fa}_{j,i} < 0; \end{cases}$$

*and* $\forall r \in s, k \in [m-1]$,

$$\omega^{(k)}_{j,r} = \begin{cases} \alpha^{(k)}_{L,r} & \textit{if} \;\; \tilde{\mathbf{W}}^{aa(k+1)}_{j,r} \geq 0 \quad (\Longleftrightarrow \mathbf{\Omega}^{(k+1)}_{j,:}\mathbf{W}^{aa}_{:,r} \geq 0); \\ \alpha^{(k)}_{U,r} & \textit{if} \;\; \tilde{\mathbf{W}}^{aa(k+1)}_{j,r} < 0 \quad (\Longleftrightarrow \mathbf{\Omega}^{(k+1)}_{j,:}\mathbf{W}^{aa}_{:,r} < 0); \end{cases}$$

$$\mathbf{\Theta}^{(k)}_{r,j} = \begin{cases} \beta^{(k)}_{L,r} & \textit{if} \;\; \tilde{\mathbf{W}}^{aa(k+1)}_{j,r} \geq 0 \quad (\Longleftrightarrow \mathbf{\Omega}^{(k+1)}_{j,:}\mathbf{W}^{aa}_{:,r} \geq 0); \\ \beta^{(k)}_{U,r} & \textit{if} \;\; \tilde{\mathbf{W}}^{aa(k+1)}_{j,r} < 0 \quad (\Longleftrightarrow \mathbf{\Omega}^{(k+1)}_{j,:}\mathbf{W}^{aa}_{:,r} < 0); \end{cases}$$

*and* $\forall r \in s, \omega^{(0)}_{j,r} = 1$.

**Corollary A. 1 (Closed-form global bounds)** *Given data $\mathbf{X} \in \mathbb{R}^{n\times m}$, $l_p$ ball parameters $p \geq 1$ and $\epsilon \geq 0$. For an $m$-layer recurrent neural network $F : \mathbb{R}^{n\times m} \to \mathbb{R}^t$, there exists two fixed values $\gamma_j^L$ and $\gamma_j^U$ such that $\forall\ \mathbf{X} \in \mathbb{R}^{n\times m}$ where $\mathbf{x}^{(k)} \in \mathbb{B}_p(\mathbf{x}_0^{(k)}, \epsilon)$, and $\forall\ j \in [t]$, $1/q = 1 - 1/p$, the inequity $\gamma_j^L \leq F_j(\mathbf{X}) \leq \gamma_j^U$ holds true, where*

$$\gamma_j^U = \mathbf{\Lambda}_{j,:}^{(0)}\mathbf{a}^{(0)} + \sum_{k=1}^{m} \epsilon\|\mathbf{\Lambda}_{j,:}^{(k)}\mathbf{W}^{ax}\|_q + \sum_{k=1}^{m} \mathbf{\Lambda}_{j,:}^{(k)}\mathbf{W}^{ax}\mathbf{x}_0^{(k)} + \sum_{k=1}^{m} \mathbf{\Lambda}_{j,:}^{(k)}(\mathbf{b}^a + \mathbf{\Delta}_{:,j}^{(k)}) + \mathbf{b}_j^F,$$
$$\gamma_j^L = \mathbf{\Omega}_{j,:}^{(0)}\mathbf{a}^{(0)} - \sum_{k=1}^{m} \epsilon\|\mathbf{\Omega}_{j,:}^{(k)}\mathbf{W}^{ax}\|_q + \sum_{k=1}^{m} \mathbf{\Omega}_{j,:}^{(k)}\mathbf{W}^{ax}\mathbf{x}_0^{(k)} + \sum_{k=1}^{m} \mathbf{\Omega}_{j,:}^{(k)}(\mathbf{b}^a + \mathbf{\Theta}_{:,j}^{(k)}) + \mathbf{b}_j^F.$$

**Theorem A. 2 (Closed-form pre-activation bounds of recurrent neural network F)** *For the pre-activation input $\mathbf{y}_j^{(v)}$ of the $v$-th layer in a given $m$-layer ($v \leq m$) recurrent neural network, there exists two explicit functions $g_j^{L,v} : \mathbb{R}^{n\times v} \to \mathbb{R}^s$ and $g_j^{U,v} : \mathbb{R}^{n\times v} \to \mathbb{R}^s$ and two fixed values $\mathbf{l}_j^{(v)}$ and $\mathbf{u}_j^{(v)}$ such that $\forall\ j \in [s]$ and $\forall\ \mathbf{X}^{(1:v)} \in \mathbb{R}^{n\times v}$ where $\mathbf{x}^{(k)} \in \mathbb{B}_p(\mathbf{x}_0^{(k)}, \epsilon)$ and $1/q = 1 - 1/p$, the inequity $\mathbf{l}_j^{(v)} \leq g_j^{L,v}(\mathbf{X}^{(1:v)}) \leq \mathbf{y}_j^{(v)} \leq g_j^{U,v}(\mathbf{X}^{(1:v)}) \leq \mathbf{u}_j^{(v)}$ holds true, where*

$$\mathbf{u}_j^{(v)} = \mathbf{\Lambda}_{j,:}^{(0)}\mathbf{a}^{(0)} + \sum_{k=1}^{v} \epsilon\|\mathbf{\Lambda}_{j,:}^{(k)}\mathbf{W}^{ax}\|_q + \sum_{k=1}^{v} \mathbf{\Lambda}_{j,:}^{(k)}\mathbf{W}^{ax}\mathbf{x}_0^{(k)} + \sum_{k=1}^{v} \mathbf{\Lambda}_{j,:}^{(k)}(\mathbf{b}^a + \mathbf{\Delta}_{:,j}^{(k)}),$$
$$\mathbf{l}_j^{(v)} = \mathbf{\Omega}_{j,:}^{(0)}\mathbf{a}^{(0)} - \sum_{k=1}^{v} \epsilon\|\mathbf{\Omega}_{j,:}^{(k)}\mathbf{W}^{ax}\|_q + \sum_{k=1}^{v} \mathbf{\Omega}_{j,:}^{(k)}\mathbf{W}^{ax}\mathbf{x}_0^{(k)} + \sum_{k=1}^{v} \mathbf{\Omega}_{j,:}^{(k)}(\mathbf{b}^a + \mathbf{\Theta}_{:,j}^{(k)}), \tag{12}$$

$$\mathbf{\Lambda}_{j,:}^{(k-1)} = \begin{cases} \mathbf{e}_j^\top & \text{if } k = v+1; \\ \mathbf{W}_{j,:}^{aa} \odot \lambda_{j,:}^{(k-1)} & \text{if } \ k = v; \\ (\mathbf{\Lambda}_{j,:}^{(k)}\mathbf{W}^{aa}) \odot \lambda_{j,:}^{(k-1)} & \text{if } \ k \in [v-1]; \end{cases} \quad \mathbf{\Omega}_{j,:}^{(k-1)} = \begin{cases} \mathbf{e}_j^\top & \text{if } k = v+1; \\ \mathbf{W}_{j,:}^{aa} \odot \omega_{j,:}^{(k-1)} & \text{if } \ k = v; \\ (\mathbf{\Omega}_{j,:}^{(k)}\mathbf{W}^{aa}) \odot \omega_{j,:}^{(k-1)} & \text{if } \ k \in [v-1]; \end{cases} \tag{13}$$

*and* $\forall r \in s, k \in [v-1]$,

$$\lambda_{j,r}^{(k)} = \begin{cases} \alpha_{U,r}^{(k)} & \text{if } \ \mathbf{\Lambda}_{j,:}^{(k+1)}\mathbf{W}_{:,r}^{aa} \geq 0; \\ \alpha_{L,r}^{(k)} & \text{if } \ \mathbf{\Lambda}_{j,:}^{(k+1)}\mathbf{W}_{:,r}^{aa} < 0; \end{cases}$$
$$\omega_{j,r}^{(k)} = \begin{cases} \alpha_{L,r}^{(k)} & \text{if } \ \mathbf{\Omega}_{j,:}^{(k+1)}\mathbf{W}_{:,r}^{aa} \geq 0); \\ \alpha_{U,r}^{(k)} & \text{if } \ \mathbf{\Omega}_{j,:}^{(k+1)}\mathbf{W}_{:,r}^{aa} < 0); \end{cases}$$
$$\mathbf{\Delta}_{r,j}^{(k)} = \begin{cases} \beta_{U,r}^{(k)} & \text{if } \ \mathbf{\Lambda}_{j,:}^{(k+1)}\mathbf{W}_{:,r}^{aa} \geq 0); \\ \beta_{L,r}^{(k)} & \text{if } \ \mathbf{\Lambda}_{j,:}^{(k+1)}\mathbf{W}_{:,r}^{aa} < 0). \end{cases}$$
$$\mathbf{\Theta}_{r,j}^{(k)} = \begin{cases} \beta_{L,r}^{(k)} & \text{if } \ \mathbf{\Omega}_{j,:}^{(k+1)}\mathbf{W}_{:,r}^{aa} \geq 0); \\ \beta_{U,r}^{(k)} & \text{if } \ \mathbf{\Omega}_{j,:}^{(k+1)}\mathbf{W}_{:,r}^{aa} < 0); \end{cases} \tag{14}$$

*and* $\forall r \in s, \lambda_{j,r}^{(0)} = \omega_{j,r}^{(0)} = 1, \mathbf{\Delta}_{r,j}^{(v)} = \mathbf{\Theta}_{r,j}^{(v)} = 0$, *where $\odot$ is the Hadamard product.*

***Proof 2*** *For a given $m$-layer ($v \leq m$) recurrent neural network, let the pre-activation input for the $j$-th neuron at the $k$-th layer be $\mathbf{y}_j^{(v)}$, where $\mathbf{x}^{(k)} \in \mathbb{B}_p(\mathbf{x}_0^{(k)}, \epsilon), \forall\ k \in [v]$. Then we have the following:*

$$\begin{aligned} \mathbf{y}_j^{(v)} &= \mathbf{W}_{j,:}^{aa}\mathbf{a}^{(v-1)} + \mathbf{W}_{j,:}^{ax}\mathbf{x}^{(v)} + \mathbf{b}_j^a, \\ &= \sum_{r=1}^{s} \mathbf{W}_{j,r}^{aa}\mathbf{a}_r^{(v-1)} + \sum_{q_v=1}^{n} \mathbf{W}_{j,q_v}^{ax}\mathbf{x}_{q_v}^{(v)} + \mathbf{b}_j^a, \end{aligned} \tag{15}$$
$$\begin{aligned} &= \sum_{r=1}^{s} \mathbf{W}_{j,r}^{aa}\sigma(\mathbf{y}_r^{(v-1)}) + \sum_{q_v=1}^{n} \mathbf{W}_{j,q_v}^{ax}\mathbf{x}_{q_v}^{(v)} + \mathbf{b}_j^a, \\ &= \sum_{\mathbf{W}_{j,r}^{aa}\geq 0} \mathbf{W}_{j,r}^{aa}\sigma(\mathbf{y}_r^{(v-1)}) + \sum_{\mathbf{W}_{j,r}^{aa}<0} \mathbf{W}_{j,r}^{aa}\sigma(\mathbf{y}_r^{(v-1)}) + \sum_{q_v=1}^{n} \mathbf{W}_{j,q_v}^{ax}\mathbf{x}_{q_v}^{(v)} + \mathbf{b}_j^a. \end{aligned} \tag{16}$$

*Assume the activation unction $\sigma(\mathbf{y}_r^{(v-1)})$ is bounded by two linear functions $h_{L,r}^{(v-1)}(\mathbf{y})$ and $h_{U,r}^{(v-1)}(\mathbf{y})$, we have*

$$h_{L,r}^{(v-1)}(\mathbf{y}_r^{(v-1)}) \leq \sigma(\mathbf{y}_r^{(v-1)}) \leq h_{U,r}^{(v-1)}(\mathbf{y}_r^{(v-1)}).$$

*Thus, if the associated weight $\mathbf{W}_{j,r}^{aa}$ to the $r$-th neuron is non-negative, we have*

$$\mathbf{W}_{j,r}^{aa} \cdot h_{L,r}^{(v-1)}(\mathbf{y}_r^{(v-1)}) \leq \mathbf{W}_{j,r}^{aa}\sigma(\mathbf{y}_r^{(v-1)}) \leq \mathbf{W}_{j,r}^{aa} \cdot h_{U,r}^{(v-1)}(\mathbf{y}_r^{(v-1)}); \tag{17}$$

*otherwise, we have*

$$\mathbf{W}_{j,r}^{aa} \cdot h_{U,r}^{(v-1)}(\mathbf{y}_r^{(v-1)}) \leq \mathbf{W}_{j,r}^{aa}\sigma(\mathbf{y}_r^{(v-1)}) \leq \mathbf{W}_{j,r}^{aa} \cdot h_{L,r}^{(v-1)}(\mathbf{y}_r^{(v-1)}). \tag{18}$$

*By using the right-hand side of Inequity* (17) *and Inequity* (18) *in Equation* (16)*, an upper bound can be obtained similarly as*

$$\begin{aligned} g_j^{U,v,v}(\mathbf{X}^{(1:v)}) = &\sum_{\mathbf{W}_{j,r}^{aa}\geq 0} \mathbf{W}_{j,r}^{aa}\ \alpha_{U,r}^{(v-1)}(\mathbf{y}_r^{(v-1)} + \beta_{U,r}^{(v-1)}) \\ &+ \sum_{\mathbf{W}_{j,r}^{aa}<0} \mathbf{W}_{j,r}^{aa}\ \alpha_{L,r}^{(v-1)}(\mathbf{y}_r^{(v-1)} + \beta_{L,r}^{(v-1)}) + \sum_{q_v=1}^{n} \mathbf{W}_{j,q_v}^{ax}\mathbf{x}_{q_v}^{(v)} + \mathbf{b}_j^a. \end{aligned}$$

*We use variables $\lambda_{j,r}^{(v-1)}$ and $\mathbf{\Delta}_{r,j}^{(v-1)}$ to denote the slops in front of $\mathbf{y}_r^{(v-1)}$ and intercepts in the parentheses:*

$$\lambda_{j,r}^{(v-1)} = \begin{cases} \alpha_{U,r}^{(v-1)} & \textit{if} \quad \mathbf{W}_{j,r}^{aa} \geq 0; \\ \alpha_{L,r}^{(v-1)} & \textit{if} \quad \mathbf{W}_{j,r}^{aa} < 0; \end{cases}$$

$$\mathbf{\Delta}_{r,j}^{(v-1)} = \begin{cases} \beta_{U,r}^{(v-1)} & \textit{if} \quad \mathbf{W}_{j,r}^{aa} \geq 0; \\ \beta_{L,r}^{(v-1)} & \textit{if} \quad \mathbf{W}_{j,r}^{aa} < 0; \end{cases}$$

*and obtain*

$$g_j^{U,v,v}(\mathbf{X}^{(1:v)}) = \sum_{r=1}^{s} \mathbf{W}_{j,r}^{aa}\ \lambda_{j,r}^{(v-1)}(\mathbf{y}_r^{(v-1)} + \mathbf{\Delta}_{r,j}^{(v-1)}) + \sum_{q_v=1}^{n} \mathbf{W}_{j,q_v}^{ax}\mathbf{x}_{q_v}^{(v)} + \mathbf{b}_j^a.$$

*We further let $\mathbf{\Lambda}_{j,r}^{(v-1)} := \mathbf{W}_{j,r}^{aa}\ \lambda_{j,r}^{(v-1)}$ and we have*

$$\begin{aligned} g_j^{U,v,v}(\mathbf{X}^{(1:v)}) &= \sum_{r=1}^{s} \mathbf{\Lambda}_{j,r}^{(v-1)}(\mathbf{y}_r^{(v-1)} + \mathbf{\Delta}_{r,j}^{(v-1)}) + \sum_{q_v=1}^{n} \mathbf{W}_{j,q_v}^{ax}\mathbf{x}_{q_v}^{(v)} + \mathbf{b}_j^a, \\ &= \sum_{r=1}^{s} \mathbf{\Lambda}_{j,r}^{(v-1)}(\mathbf{W}_{r,:}^{aa}\mathbf{a}^{(v-2)} + \mathbf{W}_{r,:}^{ax}\mathbf{x}^{(v-1)} + \mathbf{b}_r^a + \mathbf{\Delta}_{r,j}^{(v-1)}) + \sum_{q_v=1}^{n} \mathbf{W}_{j,q_v}^{ax}\mathbf{x}_{q_v}^{(v)} + \mathbf{b}_j^a, \\ &= \sum_{r=1}^{s} \mathbf{\Lambda}_{j,r}^{(v-1)}(\sum_{i=1}^{s} \mathbf{W}_{r,i}^{aa}\mathbf{a}_i^{(v-2)} + \sum_{q_{v-1}=1}^{n} \mathbf{W}_{r,q_{v-1}}^{ax}\mathbf{x}_{q_{v-1}}^{(v-1)} + \mathbf{b}_r^a + \mathbf{\Delta}_{r,j}^{(v-1)}) \\ &+ \sum_{q_v=1}^{n} \mathbf{W}_{j,q_v}^{ax}\mathbf{x}_{q_v}^{(v)} + \mathbf{b}_j^a, \\ &= \sum_{i=1}^{s}(\sum_{r=1}^{s} \mathbf{\Lambda}_{j,r}^{(v-1)}\mathbf{W}_{r,i}^{aa})\mathbf{a}_i^{(v-2)} + \sum_{q_{v-1}=1}^{n}(\sum_{r=1}^{s} \mathbf{\Lambda}_{j,r}^{(v-1)}\mathbf{W}_{r,q_{v-1}}^{ax})\mathbf{x}_{q_{v-1}}^{(v-1)} \\ &+ \sum_{r=1}^{s} \mathbf{\Lambda}_{j,r}^{(v-1)}(\mathbf{b}_r^a + \mathbf{\Delta}_{r,j}^{(v-1)}) + \sum_{q_v=1}^{n} \mathbf{W}_{j,q_v}^{ax}\mathbf{x}_{q_v}^{(v)} + \mathbf{b}_j^a. \end{aligned} \tag{19}$$

*We combine coefficients in Equation* (19) *into equivalent weights* $\tilde{\mathbf{W}}^{aa(v-1)}_{j,i}$, $\tilde{\mathbf{W}}^{ax(v-1)}_{j,q_2}$ *and bias* $\tilde{\mathbf{b}}^{(v-1)}_j$ *as defined by*

$$\begin{aligned}
\tilde{\mathbf{W}}^{aa(v-1)}_{j,i} &= \sum_{r=1}^{s} \mathbf{\Lambda}^{(v-1)}_{j,r}\mathbf{W}^{aa}_{r,i} = \mathbf{\Lambda}^{(v-1)}_{j,:}\mathbf{W}^{aa}_{:,i}, \\
\tilde{\mathbf{W}}^{ax(v-1)}_{j,q_{v-1}} &= \sum_{r=1}^{s} \mathbf{\Lambda}^{(v-1)}_{j,r}\mathbf{W}^{ax}_{r,q_{v-1}} = \mathbf{\Lambda}^{(v-1)}_{j,:}\mathbf{W}^{ax}_{:,q_{v-1}}, \\
\tilde{\mathbf{b}}^{(v-1)}_{j} &= \sum_{r=1}^{s} \mathbf{\Lambda}^{(v-1)}_{j,r}(\mathbf{b}^a_r + \mathbf{\Delta}^{(v-1)}_{r,j}) + \mathbf{b}^a_j = \mathbf{\Lambda}^{(v-1)}_{j,:}(\mathbf{b}^a + \mathbf{\Delta}^{(v-1)}_{:,j}) + \mathbf{b}^a_j,
\end{aligned}$$

*and obtain*

$$g^{U,v,v}_j(\mathbf{X}^{(1:v)}) = \sum_{i=1}^{s} \tilde{\mathbf{W}}^{aa(v-1)}_{j,i}\mathbf{a}^{(v-2)}_i + \sum_{q_{v-1}=1}^{n} \tilde{\mathbf{W}}^{ax(v-1)}_{j,q_{v-1}}\mathbf{x}^{(v-1)}_{q_{v-1}} + \sum_{q_v=1}^{n} \mathbf{W}^{ax}_{j,q_v}\mathbf{x}^{(v)}_{q_v} + \tilde{\mathbf{b}}^{(v-1)}_j. \tag{20}$$

*Notice that Equation* (15) *and Equation* (20) *are in similar forms. Thus, we can repeat the above procedure iteratively until we obtain the final upper bound* $g^{U,v,1}_j(\mathbf{X}^{(1:v)})$*, where* $\mathbf{y}^{(v)}_j \le g^{U,v,v}_j(\mathbf{X}^{(1:v)}) \le \cdots \le g^{U,v,1}_j(\mathbf{X}^{(1:v)})$*. We let* $\mathbf{u}^{(v)}_j = g^{U,v}_j(\mathbf{X}^{(1:v)})$ *denote the final upper bound* $g^{U,v,1}_j(\mathbf{X}^{(1:v)})$*, and we have*

$$\mathbf{u}^{(v)}_j = g^{U,v}_j(\mathbf{X}^{(1:v)}) = \mathbf{\Lambda}^{(0)}_{j,:}\mathbf{a}^{(0)} + \sum_{k=1}^{v} \mathbf{\Lambda}^{(k)}_{j,:}\mathbf{W}^{ax}\mathbf{x}^{(k)} + \sum_{k=1}^{v} \mathbf{\Lambda}^{(k)}_{j,:}(\mathbf{b}^a + \mathbf{\Delta}^{(k)}_{:,j})$$

*and* ($\odot$ *is the Hadamard product)*

$$\mathbf{\Lambda}^{(k-1)}_{j,:} = \begin{cases} \mathbf{e}^\top_j & \text{if } k = v+1; \\ \mathbf{W}^{aa}_{j,:} \odot \lambda^{(k-1)}_{j,:} & \text{if } k = v; \\ (\mathbf{\Lambda}^{(k)}_{j,:}\mathbf{W}^{aa}) \odot \lambda^{(k-1)}_{j,:} & \text{if } k \in [v-1]; \end{cases}$$

*and* $\forall r \in s, k \in [v-1]$,

$$\lambda^{(k)}_{j,r} = \begin{cases} \alpha^{(k)}_{U,r} & \text{if } \mathbf{\Lambda}^{(k+1)}_{j,:}\mathbf{W}^{aa}_{:,r} \ge 0; \\ \alpha^{(k)}_{L,r} & \text{if } \mathbf{\Lambda}^{(k+1)}_{j,:}\mathbf{W}^{aa}_{:,r} < 0; \end{cases}$$

$$\mathbf{\Delta}^{(k)}_{r,j} = \begin{cases} \beta^{(k)}_{U,r} & \text{if } \mathbf{\Lambda}^{(k+1)}_{j,:}\mathbf{W}^{aa}_{:,r} \ge 0); \\ \beta^{(k)}_{L,r} & \text{if } \mathbf{\Lambda}^{(k+1)}_{j,:}\mathbf{W}^{aa}_{:,r} < 0); \end{cases}$$

*and* $\forall r \in s, \lambda^{(0)}_{j,r} = 1, \mathbf{\Delta}^{(v)}_{r,j} = 0$.

***Lower bound.*** *The above derivations of upper bound can be applied similarly to derive lower bounds of* $f_j(\mathbf{X})$*, and the only difference is now we need to use the left-hand side of Inequity* (17), (18) *(rather than right-hand side when deriving upper bound) to bound the terms in* (16)*. Thus, following the same procedure in deriving the upper bounds, we can iteratively unwrap the activation functions and obtain a final lower bound* $g^{L,v,1}_j(\mathbf{X}^{(1:v)})$*, where* $\mathbf{y}^{(v)}_j \ge g^{L,v,v}_j(\mathbf{X}^{(1:v)}) \ge \cdots \ge g^{L,v,1}_j(\mathbf{X}^{(1:v)})$*. We let* $\mathbf{l}^{(v)}_j = g^{L,v}_j(\mathbf{X}^{(1:v)})$ *denote the final upper bound* $g^{L,v,1}_j(\mathbf{X}^{(1:v)})$*, and we have*

$$\mathbf{l}^{(v)}_j = g^{L,v}_j(\mathbf{X}^{(1:v)}) = \mathbf{\Omega}^{(0)}_{j,:}\mathbf{a}^{(0)} + \sum_{k=1}^{v} \mathbf{\Omega}^{(k)}_{j,:}\mathbf{W}^{ax}\mathbf{x}^{(k)} + \sum_{k=1}^{v} \mathbf{\Omega}^{(k)}_{j,:}(\mathbf{b}^a + \mathbf{\Theta}^{(k)}_{:,j})$$

*and* ($\odot$ *is the Hadamard product)*

$$\mathbf{\Omega}^{(k-1)}_{j,:} = \begin{cases} \mathbf{e}^\top_j & \text{if } k = v+1; \\ \mathbf{W}^{aa}_{j,:} \odot \omega^{(k-1)}_{j,:} & \text{if } k = v; \\ (\mathbf{\Omega}^{(k)}_{j,:}\mathbf{W}^{aa}) \odot \omega^{(k-1)}_{j,:} & \text{if } k \in [v-1]; \end{cases}$$

*and* $\forall r \in s, k \in [v-1]$,

$$\omega_{j,r}^{(k)} = \begin{cases} \alpha_{L,r}^{(k)} & \textit{if} \quad \mathbf{\Omega}_{j,:}^{(k+1)} \mathbf{W}_{:,r}^{aa} \geq 0); \\ \alpha_{U,r}^{(k)} & \textit{if} \quad \mathbf{\Omega}_{j,:}^{(k+1)} \mathbf{W}_{:,r}^{aa} < 0); \end{cases}$$

$$\mathbf{\Theta}_{r,j}^{(k)} = \begin{cases} \beta_{L,r}^{(k)} & \textit{if} \quad \mathbf{\Omega}_{j,:}^{(k+1)} \mathbf{W}_{:,r}^{aa} \geq 0); \\ \beta_{U,r}^{(k)} & \textit{if} \quad \mathbf{\Omega}_{j,:}^{(k+1)} \mathbf{W}_{:,r}^{aa} < 0). \end{cases}$$

*and* $\forall r \in s, \omega_{j,r}^{(0)} = 1, \mathbf{\Theta}_{r,j}^{(v)} = 0$.

### A.2 Algorithms for Recurrent Neural Networks

**Algorithm 1** *Compute POPQORN robustness bound of recurrent neural network (true label: c, target label: i)*

***Input***: *weight matrices* $\mathbf{W}^{aa}$, $\mathbf{W}^{Fa}$, $\mathbf{W}^{ax}$ *and bias vectors* $\mathbf{b}^{a}$, $\mathbf{b}^{f}$ *of an* $m$*-layer recurrent neural network* $f$*, input sequence* $[\mathbf{x}^{(1)}, \ldots, \mathbf{x}^{(m)}]$*, p-norm,* $\epsilon_0$.

***Output***: *a robustness bound* $\tilde{\epsilon}$.

*Replace the last layer weights* $\overline{\mathbf{w}} \leftarrow \mathbf{W}^{Fa}_{c,:} - \mathbf{W}^{Fa}_{i,:}$

*Initialize* $\epsilon \leftarrow \epsilon_0$

***while*** $\epsilon$ *has not achieved a desired accuracy and iteration limit has not reached* ***do***

    ***for*** *v=1,...,m* ***do***

        ***for*** *j=1,...,s* ***do***

            $\mathbf{l}^{(v)}_j$, $\mathbf{u}^{(v)}_j$ $\leftarrow$ *compute the pre-activation bound for the* $j$*-th neuron of the* $v$*-th layer according to Equation* (12)*,* (13) *and* (14).

            $\alpha^{(v)}_{L,j}$, $\alpha^{(v)}_{U,j}$, $\beta^{(v)}_{L,j}$, $\beta^{(v)}_{U,j}$ $\leftarrow$ *compute the two bounding linear function* $h^{(v)}_{L,j}$, $h^{(v)}_{U,j}$

        ***end for***

    ***end for***

    $\gamma^U, \gamma^L \leftarrow$ *Corollary A.1*

    ***if*** $\gamma^L \geq 0$ ***then***

        $\epsilon$ *is a lower bound; increase* $\epsilon$ *using a binary search procedure*

    ***else***

        $\epsilon$ *is not a lower bound; decrease* $\epsilon$ *using a binary search procedure*

    ***end if***

    $\tilde{\epsilon} \leftarrow \epsilon$

***end while***

### A.3 Long Short-term Memory Network

**Notations** In the derivation of long short-term memory network (LSTM), we define the equations as follows:

$$
\begin{aligned}
\text{Input gate:} \quad & \mathbf{i}^{(k)} = \sigma(\mathbf{y}^{i(k)}) = \sigma(\mathbf{W}^{ix}\mathbf{x}^{(k)} + \mathbf{W}^{ia}\mathbf{a}^{(k-1)} + \mathbf{b}^{i}); \\
\text{Forget gate:} \quad & \mathbf{f}^{(k)} = \sigma(\mathbf{y}^{f(k)}) = \sigma(\mathbf{W}^{fx}\mathbf{x}^{(k)} + \mathbf{W}^{fa}\mathbf{a}^{(k-1)} + \mathbf{b}^{f}); \\
\text{Cell gate:} \quad & \mathbf{g}^{(k)} = \tanh(\mathbf{y}^{g(k)}) = \tanh(\mathbf{W}^{gx}\mathbf{x}^{(k)} + \mathbf{W}^{ga}\mathbf{a}^{(k-1)} + \mathbf{b}^{g}); \\
\text{Output gate:} \quad & \mathbf{o}^{(k)} = \sigma(\mathbf{y}^{o(k)}) = \sigma(\mathbf{W}^{ox}\mathbf{x}^{(k)} + \mathbf{W}^{oa}\mathbf{a}^{(k-1)} + \mathbf{b}^{o}); \\
\text{Cell state:} \quad & \mathbf{c}^{(k)} = \mathbf{f}^{(k)} \odot \mathbf{c}^{(k-1)} + \mathbf{i}^{(k)} \odot \mathbf{g}^{(k)}; \\
\text{Hidden state:} \quad & \mathbf{a}^{(k)} = \mathbf{o}^{(k)} \odot \tanh(\mathbf{c}^{(k)}).
\end{aligned}
$$

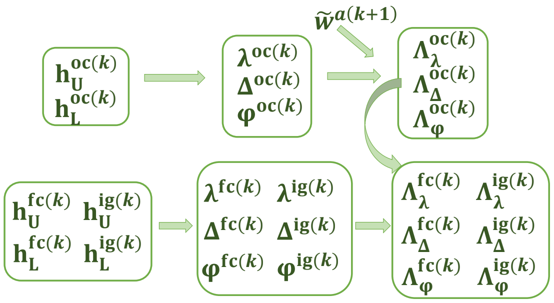


Figure 2: Steps in computing bounds for a long short-term memory network.

**Definition 1 (Linear bounds on 2D activation function)** *For the r-th neuron in k-th layer with pre-activation bounds of $\mathbf{y}_r^{o(k)}, \mathbf{c}_r^{(k)}$: $\mathbf{l}_r^{o(k)}$, $\mathbf{u}_r^{o(k)}$, $\mathbf{l}_r^{c(k)}$, $\mathbf{u}_r^{c(k)}$ and the activation functions, define two linear functions $h_{L,r}^{oc(k)}$, $h_{U,r}^{oc(k)} : \mathbb{R}^2 \to \mathbb{R}$,*

$$
\begin{aligned}
h_{L,r}^{oc(k)}(\mathbf{y}_r^{o(k)}, \mathbf{c}_r^{(k)}) = \alpha_{L,r}^{oc(k)} \mathbf{y}_r^{o(k)} + \beta_{L,r}^{oc(k)} \mathbf{c}_r^{(k)} + \gamma_{L,r}^{oc(k)}, \\
h_{U,r}^{oc(k)}(\mathbf{y}_r^{o(k)}, \mathbf{c}_r^{(k)}) = \alpha_{U,r}^{oc(k)} \mathbf{y}_r^{o(k)} + \beta_{U,r}^{oc(k)} \mathbf{c}_r^{(k)} + \gamma_{U,r}^{oc(k)},
\end{aligned}
$$

*such that for $\mathbf{y}_r^{o(k)} \in [\mathbf{l}_r^{o(k)}, \mathbf{u}_r^{o(k)}]$, $\mathbf{c}_r^{(k)} \in [\mathbf{l}_r^{c(k)}, \mathbf{u}_r^{c(k)}]$,*

$$
h_{L,r}^{oc(k)}(\mathbf{y}_r^{o(k)}, \mathbf{c}_r^{(k)}) \le \sigma(\mathbf{y}_r^{o(k)}) \tanh(\mathbf{c}_r^{(k)}) \le h_{U,r}^{oc(k)}(\mathbf{y}_r^{o(k)}, \mathbf{c}_r^{(k)}).
$$

*Similarly, we can define linear functions $h_{L,r}^{fc(k)}$, $h_{U,r}^{fc(k)}$, $h_{L,r}^{ig(k)}$, and $h_{U,r}^{ig(k)}$ such that for $\mathbf{y}_r^{f(k)} \in [\mathbf{l}_r^{f(k)}, \mathbf{u}_r^{f(k)}]$, $\mathbf{c}_r^{(k-1)} \in [\mathbf{l}_r^{c(k-1)}, \mathbf{u}_r^{c(k-1)}]$,*

$$
h_{L,r}^{fc(k)}(\mathbf{y}_r^{f(k)}, \mathbf{c}_r^{(k-1)}) \le \sigma(\mathbf{y}_r^{f(k)}) \mathbf{c}_r^{(k-1)} \le h_{U,r}^{fc(k)}(\mathbf{y}_r^{f(k)}, \mathbf{c}_r^{(k-1)});
$$

*and for $\mathbf{y}_r^{i(k)} \in [\mathbf{l}_r^{i(k)}, \mathbf{u}_r^{i(k)}]$, $\mathbf{y}_r^{g(k)} \in [\mathbf{l}_r^{g(k)}, \mathbf{u}_r^{g(k)}]$,*

$$
h_{L,r}^{ig(k)}(\mathbf{y}_r^{i(k)}, \mathbf{y}_r^{g(k)}) \le \sigma(\mathbf{y}_r^{i(k)}) \tanh(\mathbf{y}_r^{g(k)}) \le h_{U,r}^{ig(k)}(\mathbf{y}_r^{i(k)}, \mathbf{y}_r^{g(k)}).
$$

**Theorem A. 3 (Explicit output bound of long short-term memory network F)** *Given an $m$-layer long short-term memory network $F : \mathbb{R}^{n \times m} \to \mathbb{R}^t$, we can derive two explicit functions $F_j^L : \mathbb{R}^{n \times m} \to \mathbb{R}$ and $F_j^U : \mathbb{R}^{n \times m} \to \mathbb{R}$ such that $\forall\ j \in [t]$ and $\forall\ \mathbf{X} \in \mathbb{R}^{n \times m}$ where $\mathbf{x}^{(k)} \in \mathbb{B}_p(\mathbf{x}_0^{(k)}, \epsilon)$, the inequity $F_j^L(\mathbf{X}) \le F_j(\mathbf{X}) \le F_j^U(\mathbf{X})$ holds true. We can obtain them through following steps: Starting from $k = m$, $\forall r \in s$ we*

**1. define unified slopes and intercepts of cross terms of the cell state and the output gate;**

$$\lambda_{j,r}^{oc(k)} = \begin{cases} \alpha_{U,r}^{oc(k)} & \textit{if} \;\; \tilde{\mathbf{W}}_{U,j,r}^{a(k+1)} \geq 0; \\ \alpha_{L,r}^{oc(k)} & \textit{if} \;\; \tilde{\mathbf{W}}_{U,j,r}^{a(k+1)} < 0; \end{cases} \quad \omega_{j,r}^{oc(k)} = \begin{cases} \alpha_{L,r}^{oc(k)} & \textit{if} \;\; \tilde{\mathbf{W}}_{L,j,r}^{a(k+1)} \geq 0; \\ \alpha_{U,r}^{oc(k)} & \textit{if} \;\; \tilde{\mathbf{W}}_{L,j,r}^{a(k+1)} < 0; \end{cases}$$

$$\mathbf{\Delta}_{j,r}^{oc(k)} = \begin{cases} \beta_{U,r}^{oc(k)} & \textit{if} \;\; \tilde{\mathbf{W}}_{U,j,r}^{a(k+1)} \geq 0; \\ \beta_{L,r}^{oc(k)} & \textit{if} \;\; \tilde{\mathbf{W}}_{U,j,r}^{a(k+1)} < 0; \end{cases} \quad \mathbf{\Theta}_{j,r}^{oc(k)} = \begin{cases} \beta_{L,r}^{oc(k)} & \textit{if} \;\; \tilde{\mathbf{W}}_{L,j,r}^{a(k+1)} \geq 0; \\ \beta_{U,r}^{oc(k)} & \textit{if} \;\; \tilde{\mathbf{W}}_{L,j,r}^{a(k+1)} < 0; \end{cases}$$

$$\varphi_{j,r}^{oc(k)} = \begin{cases} \gamma_{U,r}^{oc(k)} & \textit{if} \;\; \tilde{\mathbf{W}}_{U,j,r}^{a(k+1)} \geq 0; \\ \gamma_{L,r}^{oc(k)} & \textit{if} \;\; \tilde{\mathbf{W}}_{U,j,r}^{a(k+1)} < 0; \end{cases} \quad \psi_{j,r}^{oc(k)} = \begin{cases} \gamma_{L,r}^{oc(k)} & \textit{if} \;\; \tilde{\mathbf{W}}_{L,j,r}^{a(k+1)} \geq 0; \\ \gamma_{U,r}^{oc(k)} & \textit{if} \;\; \tilde{\mathbf{W}}_{L,j,r}^{a(k+1)} < 0; \end{cases}$$

*where* $\tilde{\mathbf{W}}_{U,j,r}^{a(m+1)} = \tilde{\mathbf{W}}_{L,j,r}^{a(m+1)} = \mathbf{W}_{j,r}^{Fa}$;

**2. collect coefficients in front of the cell state and the output gate *pre-activation*, and constants;**

$$\mathbf{\Lambda}_{\lambda,j,:}^{oc(k)} = \begin{cases} \mathbf{W}_{j,:}^{Fa} \odot \lambda_{j,:}^{oc(k)} & \textit{if} \;\; k = m; \\ \tilde{\mathbf{W}}_{U,j,:}^{a(k+1)} \odot \lambda_{j,:}^{oc(k)} & \textit{if} \;\; k \in [m-1]; \end{cases} \quad \mathbf{\Omega}_{\omega,j,:}^{oc(k)} = \begin{cases} \mathbf{W}_{j,:}^{Fa} \odot \omega_{j,:}^{oc(k)} & \textit{if} \;\; k = m; \\ \tilde{\mathbf{W}}_{L,j,:}^{a(k+1)} \odot \omega_{j,:}^{oc(k)} & \textit{if} \;\; k \in [m-1]; \end{cases}$$

$$\mathbf{\Lambda}_{\Delta,j,:}^{oc(k)} = \begin{cases} \mathbf{W}_{j,:}^{Fa} \odot \mathbf{\Delta}_{j,:}^{oc(k)} & \textit{if} \;\; k = m; \\ \tilde{\mathbf{W}}_{U,j,:}^{a(k+1)} \odot \mathbf{\Delta}_{j,:}^{oc(k)} & +\mathbf{\Lambda}_{\Delta,j,:}^{fc(k+1)} \\ & \textit{if} \;\; k \in [m-1]; \end{cases} \quad \mathbf{\Omega}_{\Theta,j,:}^{oc(k)} = \begin{cases} \mathbf{W}_{j,:}^{Fa} \odot \mathbf{\Theta}_{j,:}^{oc(k)} & \textit{if} \;\; k = m; \\ \tilde{\mathbf{W}}_{L,j,:}^{a(k+1)} \odot \mathbf{\Theta}_{j,:}^{oc(k)} & +\mathbf{\Omega}_{\Theta,j,:}^{fc(k+1)} \\ & \textit{if} \;\; k \in [m-1]; \end{cases}$$

$$\mathbf{\Lambda}_{\varphi,j,:}^{oc(k)} = \begin{cases} \mathbf{W}_{j,:}^{Fa} \odot \varphi_{j,:}^{oc(k)} & \textit{if} \;\; k = m; \\ \tilde{\mathbf{W}}_{U,j,:}^{a(k+1)} \odot \varphi_{j,:}^{oc(k)} & \textit{if} \;\; k \in [m-1]; \end{cases} \quad \mathbf{\Omega}_{\psi,j,:}^{oc(k)} = \begin{cases} \mathbf{W}_{j,:}^{Fa} \odot \psi_{j,:}^{oc(k)} & \textit{if} \;\; k = m; \\ \tilde{\mathbf{W}}_{L,j,:}^{a(k+1)} \odot \psi_{j,:}^{oc(k)} & \textit{if} \;\; k \in [m-1]; \end{cases}$$

**3. define unified slopes and intercepts of cross terms of the cell state and the forget gate, the input gate and the cell gate;**

$$\lambda_{j,r}^{fc(k)} = \begin{cases} \alpha_{U,r}^{fc(k)} & \textit{if} \;\; \mathbf{\Lambda}_{\Delta,j,r}^{oc(k)} \geq 0; \\ \alpha_{L,r}^{fc(k)} & \textit{if} \;\; \mathbf{\Lambda}_{\Delta,j,r}^{oc(k)} < 0; \end{cases} \quad \omega_{j,r}^{fc(k)} = \begin{cases} \alpha_{L,r}^{fc(k)} & \textit{if} \;\; \mathbf{\Omega}_{\Theta,j,r}^{oc(k)} \geq 0; \\ \alpha_{U,r}^{fc(k)} & \textit{if} \;\; \mathbf{\Omega}_{\Theta,j,r}^{oc(k)} < 0; \end{cases}$$

$$\mathbf{\Delta}_{j,r}^{fc(k)} = \begin{cases} \beta_{U,r}^{fc(k)} & \textit{if} \;\; \mathbf{\Lambda}_{\Delta,j,r}^{oc(k)} \geq 0; \\ \beta_{L,r}^{fc(k)} & \textit{if} \;\; \mathbf{\Lambda}_{\Delta,j,r}^{oc(k)} < 0; \end{cases} \quad \mathbf{\Theta}_{j,r}^{fc(k)} = \begin{cases} \beta_{L,r}^{fc(k)} & \textit{if} \;\; \mathbf{\Omega}_{\Theta,j,r}^{oc(k)} \geq 0; \\ \beta_{U,r}^{fc(k)} & \textit{if} \;\; \mathbf{\Omega}_{\Theta,j,r}^{oc(k)} < 0; \end{cases}$$

$$\varphi_{j,r}^{fc(k)} = \begin{cases} \gamma_{U,r}^{fc(k)} & \textit{if} \;\; \mathbf{\Lambda}_{\Delta,j,r}^{oc(k)} \geq 0; \\ \gamma_{L,r}^{fc(k)} & \textit{if} \;\; \mathbf{\Lambda}_{\Delta,j,r}^{oc(k)} < 0; \end{cases} \quad \psi_{j,r}^{fc(k)} = \begin{cases} \gamma_{L,r}^{fc(k)} & \textit{if} \;\; \mathbf{\Omega}_{\Theta,j,r}^{oc(k)} \geq 0; \\ \gamma_{U,r}^{fc(k)} & \textit{if} \;\; \mathbf{\Omega}_{\Theta,j,r}^{oc(k)} < 0; \end{cases}$$

$$\lambda_{j,r}^{ig(k)} = \begin{cases} \alpha_{U,r}^{ig(k)} & \textit{if} \;\; \mathbf{\Lambda}_{\Delta,j,r}^{oc(k)} \geq 0; \\ \alpha_{L,r}^{ig(k)} & \textit{if} \;\; \mathbf{\Lambda}_{\Delta,j,r}^{oc(k)} < 0; \end{cases} \quad \omega_{j,r}^{ig(k)} = \begin{cases} \alpha_{L,r}^{ig(k)} & \textit{if} \;\; \mathbf{\Omega}_{\Theta,j,r}^{oc(k)} \geq 0; \\ \alpha_{U,r}^{ig(k)} & \textit{if} \;\; \mathbf{\Omega}_{\Theta,j,r}^{oc(k)} < 0; \end{cases}$$

$$\mathbf{\Delta}_{j,r}^{ig(k)} = \begin{cases} \beta_{U,r}^{ig(k)} & \textit{if} \;\; \mathbf{\Lambda}_{\Delta,j,r}^{oc(k)} \geq 0; \\ \beta_{L,r}^{ig(k)} & \textit{if} \;\; \mathbf{\Lambda}_{\Delta,j,r}^{oc(k)} < 0; \end{cases} \quad \mathbf{\Theta}_{j,r}^{ig(k)} = \begin{cases} \beta_{L,r}^{ig(k)} & \textit{if} \;\; \mathbf{\Omega}_{\Theta,j,r}^{oc(k)} \geq 0; \\ \beta_{U,r}^{ig(k)} & \textit{if} \;\; \mathbf{\Omega}_{\Theta,j,r}^{oc(k)} < 0; \end{cases}$$

$$\varphi_{j,r}^{ig(k)} = \begin{cases} \gamma_{U,r}^{ig(k)} & \textit{if} \;\; \mathbf{\Lambda}_{\Delta,j,r}^{oc(k)} \geq 0; \\ \gamma_{L,r}^{ig(k)} & \textit{if} \;\; \mathbf{\Lambda}_{\Delta,j,r}^{oc(k)} < 0; \end{cases} \quad \psi_{j,r}^{ig(k)} = \begin{cases} \gamma_{L,r}^{ig(k)} & \textit{if} \;\; \mathbf{\Omega}_{\Theta,j,r}^{oc(k)} \geq 0; \\ \gamma_{U,r}^{ig(k)} & \textit{if} \;\; \mathbf{\Omega}_{\Theta,j,r}^{oc(k)} < 0; \end{cases}$$

**4. collect coefficients in front of the cell state, the forget gate *pre-activation*, the input gate *pre-activation*, the cell gate *pre-activation*, and constants of the two couplings;**

$$\mathbf{\Lambda}_{\lambda,j,:}^{fc(k)} = \mathbf{\Lambda}_{\Delta,j,:}^{oc(k)} \odot \lambda_{j,:}^{fc(k)}; \quad \mathbf{\Omega}_{\omega,j,:}^{fc(k)} = \mathbf{\Omega}_{\Theta,j,:}^{oc(k)} \odot \omega_{j,:}^{fc(k)};$$

$$\mathbf{\Lambda}_{\Delta,j,:}^{fc(k)} = \mathbf{\Lambda}_{\Delta,j,:}^{oc(k)} \odot \mathbf{\Delta}_{j,:}^{fc(k)}; \quad \mathbf{\Omega}_{\Theta,j,:}^{fc(k)} = \mathbf{\Omega}_{\Theta,j,:}^{oc(k)} \odot \mathbf{\Theta}_{j,:}^{fc(k)};$$

$$\mathbf{\Lambda}_{\varphi,j,:}^{fc(k)} = \mathbf{\Lambda}_{\Delta,j,:}^{oc(k)} \odot \varphi_{j,:}^{fc(k)}; \quad \mathbf{\Omega}_{\psi,j,:}^{fc(k)} = \mathbf{\Omega}_{\Theta,j,:}^{oc(k)} \odot \psi_{j,:}^{fc(k)};$$

$$\mathbf{\Lambda}_{\lambda,j,:}^{ig(k)} = \mathbf{\Lambda}_{\Delta,j,:}^{oc(k)} \odot \lambda_{j,:}^{ig(k)}; \quad \mathbf{\Omega}_{\omega,j,:}^{ig(k)} = \mathbf{\Omega}_{\Theta,j,:}^{oc(k)} \odot \omega_{j,:}^{ig(k)};$$

$$\mathbf{\Lambda}^{ig(k)}_{\Delta,j,:} = \mathbf{\Lambda}^{oc(k)}_{\Delta,j,:} \odot \mathbf{\Delta}^{ig(k)}_{j,:}; \qquad \mathbf{\Omega}^{ig(k)}_{\Theta,j,:} = \mathbf{\Omega}^{oc(k)}_{\Theta,j,:} \odot \mathbf{\Theta}^{ig(k)}_{j,:};$$

$$\mathbf{\Lambda}^{ig(k)}_{\varphi,j,:} = \mathbf{\Lambda}^{oc(k)}_{\Delta,j,:} \odot \varphi^{ig(k)}_{j,:}; \qquad \mathbf{\Omega}^{ig(k)}_{\psi,j,:} = \mathbf{\Omega}^{oc(k)}_{\Theta,j,:} \odot \psi^{ig(k)}_{j,:};$$

**5. define equivalent weight matrices and biases;**

$$\begin{aligned}
\tilde{\mathbf{W}}^{x(k)}_{U,j,q_k} &= \mathbf{\Lambda}^{oc(k)}_{\lambda,j,:}\mathbf{W}^{ox}_{:,q_k} + \mathbf{\Lambda}^{fc(k)}_{\lambda,j,:}\mathbf{W}^{fx}_{:,q_k} + \mathbf{\Lambda}^{ig(k)}_{\lambda,j,:}\mathbf{W}^{ix}_{:,q_k} + \mathbf{\Lambda}^{ig(k)}_{\Delta,j,:}\mathbf{W}^{gx}_{:,q_k};\\
\tilde{\mathbf{W}}^{a(k)}_{U,j,r} &= \mathbf{\Lambda}^{oc(k)}_{\lambda,j,:}\mathbf{W}^{oa}_{:,r} + \mathbf{\Lambda}^{fc(k)}_{\lambda,j,:}\mathbf{W}^{fa}_{:,r} + \mathbf{\Lambda}^{ig(k)}_{\lambda,j,:}\mathbf{W}^{ia}_{:,r} + \mathbf{\Lambda}^{ig(k)}_{\Delta,j,:}\mathbf{W}^{ga}_{:,r};\\
\tilde{\mathbf{b}}^{(k)}_{U,j} &= \mathbf{\Lambda}^{oc(k)}_{\lambda,j,:}\mathbf{b}^{o} + \mathbf{\Lambda}^{fc(k)}_{\lambda,j,:}\mathbf{b}^{f} + \mathbf{\Lambda}^{ig(k)}_{\lambda,j,:}\mathbf{b}^{i} + \mathbf{\Lambda}^{ig(k)}_{\Delta,j,:}\mathbf{b}^{g} + \sum_{i=1}^{s}(\mathbf{\Lambda}^{oc(k)}_{\varphi,j,i} + \mathbf{\Lambda}^{fc(k)}_{\varphi,j,i} + \mathbf{\Lambda}^{ig(k)}_{\varphi,j,i});\\
\tilde{\mathbf{W}}^{x(k)}_{L,j,q_k} &= \mathbf{\Omega}^{oc(k)}_{\omega,j,:}\mathbf{W}^{ox}_{:,q_k} + \mathbf{\Omega}^{fc(k)}_{\omega,j,:}\mathbf{W}^{fx}_{:,q_k} + \mathbf{\Omega}^{ig(k)}_{\omega,j,:}\mathbf{W}^{ix}_{:,q_k} + \mathbf{\Omega}^{ig(k)}_{\Theta,j,:}\mathbf{W}^{gx}_{:,q_k};\\
\tilde{\mathbf{W}}^{a(k)}_{L,j,r} &= \mathbf{\Omega}^{oc(k)}_{\omega,j,:}\mathbf{W}^{oa}_{:,r} + \mathbf{\Omega}^{fc(k)}_{\omega,j,:}\mathbf{W}^{fa}_{:,r} + \mathbf{\Omega}^{ig(k)}_{\omega,j,:}\mathbf{W}^{ia}_{:,r} + \mathbf{\Omega}^{ig(k)}_{\Theta,j,:}\mathbf{W}^{ga}_{:,r};\\
\tilde{\mathbf{b}}^{(k)}_{L,j} &= \mathbf{\Omega}^{oc(k)}_{\omega,j,:}\mathbf{b}^{o} + \mathbf{\Omega}^{fc(k)}_{\omega,j,:}\mathbf{b}^{f} + \mathbf{\Omega}^{ig(k)}_{\omega,j,:}\mathbf{b}^{i} + \mathbf{\Omega}^{ig(k)}_{\Theta,j,:}\mathbf{b}^{g} + \sum_{i=1}^{s}(\mathbf{\Omega}^{oc(k)}_{\psi,j,i} + \mathbf{\Omega}^{fc(k)}_{\psi,j,i} + \mathbf{\Omega}^{ig(k)}_{\psi,j,i});
\end{aligned}$$

**6. After looping steps 1 to 5 from $k = m$ to $k = 1$, the bounds are given by**

$$\begin{aligned}
F^{U}_{j}(\mathbf{X}) &= \tilde{\mathbf{W}}^{a(1)}_{U,j,:}\mathbf{a}^{(0)} + \mathbf{\Lambda}^{fc(1)}_{\Delta,j,:}\mathbf{c}^{(0)} + \sum_{k=1}^{m}\tilde{\mathbf{W}}^{x(k)}_{U,j,:}\mathbf{x}^{(k)} + \sum_{k=1}^{m}\tilde{\mathbf{b}}^{(k)}_{U,j} + \mathbf{b}^{F}_{j},\\
F^{L}_{j}(\mathbf{X}) &= \tilde{\mathbf{W}}^{a(1)}_{L,j,:}\mathbf{a}^{(0)} + \mathbf{\Omega}^{fc(1)}_{\Theta,j,:}\mathbf{c}^{(0)} + \sum_{k=1}^{m}\tilde{\mathbf{W}}^{x(k)}_{L,j,:}\mathbf{x}^{(k)} + \sum_{k=1}^{m}\tilde{\mathbf{b}}^{(k)}_{L,j} + \mathbf{b}^{F}_{j}.
\end{aligned}$$

*Though we exemplify by an $m$-layer many-to-one long short-term memory network, the above steps can also be used to derive bounds for the $k$-th output $\mathbf{W}^{Fa}\mathbf{a}^{(k)} + \mathbf{b}^{F}$ in a many-to-many long short-term memory network.*

***Proof 3*** *Given an $m$-layer long short-term memory network $F : \mathbb{R}^{n\times m} \to \mathbb{R}^{t}$ with pre-activation bounds $\mathbf{l}^{o(k)}$,$\mathbf{u}^{o(k)}$, $\mathbf{l}^{c(k)}$,$\mathbf{u}^{c(k)}$, $\mathbf{l}^{f(k)}$,$\mathbf{u}^{f(k)}$, $\mathbf{l}^{i(k)}$,$\mathbf{u}^{i(k)}$, $\mathbf{l}^{g(k)}$ and $\mathbf{u}^{g(k)}$ for $\mathbf{X} \in \mathbb{R}^{n\times m}$, where $\mathbf{x}^{(k)} \in \mathbb{B}_{p}(\mathbf{x}^{(k)}_{0}, \epsilon)$, let the pre-activation inputs for the $j$-th neuron at the output layer be $F_j(\mathbf{X}) = \mathbf{W}^{Fa}_{j,:}\mathbf{a}^{(m)} + \mathbf{b}^{F}_{j}$. The $j$-th output of the recurrent neural network is the following:*

$$\begin{aligned}
F_j(\mathbf{X}) &= \mathbf{W}^{Fa}_{j,:}\mathbf{a}^{(m)} + \mathbf{b}^{F}_{j},\\
&= \sum_{i=1}^{s}\mathbf{W}^{Fa}_{j,i}\mathbf{a}^{(m)}_{i} + \mathbf{b}^{F}_{j},\\
&= \sum_{i=1}^{s}\mathbf{W}^{Fa}_{j,i}[\mathbf{o}^{(m)}_{i}\tanh(\mathbf{c}^{(m)}_{i})] + \mathbf{b}^{F}_{j},\\
&= \sum_{i=1}^{s}\mathbf{W}^{Fa}_{j,i}[\sigma(\mathbf{y}^{o(m)}_{i})\tanh(\mathbf{c}^{(m)}_{i})] + \mathbf{b}^{F}_{j},\\
&= \sum_{\mathbf{W}^{Fa}_{j,i}\geq 0}\mathbf{W}^{Fa}_{j,i}[\sigma(\mathbf{y}^{o(m)}_{i})\tanh(\mathbf{c}^{(m)}_{i})] + \sum_{\mathbf{W}^{Fa}_{j,i}< 0}\mathbf{W}^{Fa}_{j,i}[\sigma(\mathbf{y}^{o(m)}_{i})\tanh(\mathbf{c}^{(m)}_{i})] + \mathbf{b}^{F}_{j}.
\end{aligned}$$

*Assume the activation function $\sigma(\mathbf{y})\tanh(\mathbf{x})$ is bounded by two linear functions $h^{oc(m)}_{L,i}(\mathbf{y},\mathbf{x})$, $h^{oc(m)}_{U,i}(\mathbf{y},\mathbf{x})$, we have*

$$h^{oc(m)}_{L,i}(\mathbf{y}^{o(m)}_{i},\mathbf{c}^{(m)}_{i}) \leq \sigma(\mathbf{y}^{o(m)}_{i})\tanh(\mathbf{c}^{(m)}_{i}) \leq h^{oc(m)}_{U,i}(\mathbf{y}^{o(m)}_{i},\mathbf{c}^{(m)}_{i}).$$

***Upper bound.*** *We can then obtain*

$$
\begin{aligned}
F_j(\mathbf{X}) \le & \sum_{\mathbf{W}^{Fa}_{j,i} \ge 0} \mathbf{W}^{Fa}_{j,i} \; (\alpha^{oc(m)}_{U,i} \mathbf{y}^{o(m)}_i + \beta^{oc(m)}_{U,i} \mathbf{c}^{(m)}_i + \gamma^{oc(m)}_{U,i}) \\
& + \sum_{\mathbf{W}^{Fa}_{j,i} < 0} \mathbf{W}^{fa}_{j,i} \; (\alpha^{oc(m)}_{L,i} \mathbf{y}^{o(m)}_i + \beta^{oc(m)}_{L,i} \mathbf{c}^{(m)}_i + \gamma^{oc(m)}_{L,i}) + \mathbf{b}^F_j.
\end{aligned}
$$

*We then define $\lambda^{oc(m)}_{j,i}$, $\mathbf{\Delta}^{oc(m)}_{j,i}$ and $\varphi^{oc(m)}_{j,i}$ in the parentheses:*

$$
\lambda^{oc(m)}_{j,i} = \begin{cases} \alpha^{oc(m)}_{U,i} & \textit{if } \mathbf{W}^{Fa}_{j,i} \ge 0; \\ \alpha^{oc(m)}_{L,i} & \textit{if } \mathbf{W}^{Fa}_{j,i} < 0; \end{cases}
$$

$$
\mathbf{\Delta}^{oc(m)}_{j,i} = \begin{cases} \beta^{oc(m)}_{U,i} & \textit{if } \mathbf{W}^{Fa}_{j,i} \ge 0; \\ \beta^{oc(m)}_{L,i} & \textit{if } \mathbf{W}^{Fa}_{j,i} < 0; \end{cases}
$$

$$
\varphi^{oc(m)}_{j,i} = \begin{cases} \gamma^{oc(m)}_{U,i} & \textit{if } \mathbf{W}^{Fa}_{j,i} \ge 0; \\ \gamma^{oc(m)}_{L,i} & \textit{if } \mathbf{W}^{Fa}_{j,i} < 0; \end{cases}
$$

*and obtain*

$$
F_j(\mathbf{X}) \le \sum_{i=1}^{s} \mathbf{W}^{Fa}_{j,i} \; (\lambda^{oc(m)}_{j,i} \mathbf{y}^{o(m)}_i + \mathbf{\Delta}^{oc(m)}_{j,i} \mathbf{c}^{(m)}_i + \varphi^{oc(m)}_{j,i}) + \mathbf{b}^F_j.
$$

*We further let*

$$
\mathbf{\Lambda}^{oc(m)}_{\lambda,j,i} := \mathbf{W}^{Fa}_{j,i} \; \lambda^{oc(m)}_{j,i}, \; \mathbf{\Lambda}^{oc(m)}_{\Delta,j,i} := \mathbf{W}^{Fa}_{j,i} \; \mathbf{\Delta}^{oc(m)}_{j,i}, \; \mathbf{\Lambda}^{oc(m)}_{\varphi,j,i} := \mathbf{W}^{Fa}_{j,i} \; \varphi^{oc(m)}_{j,i},
$$

*and we have*

$$
\begin{aligned}
F_j(\mathbf{X}) \le & \sum_{i=1}^{s} (\mathbf{\Lambda}^{oc(m)}_{\lambda,j,i} \mathbf{y}^{o(m)}_i + \mathbf{\Lambda}^{oc(m)}_{\Delta,j,i} \mathbf{c}^{(m)}_i + \mathbf{\Lambda}^{oc(m)}_{\varphi,j,i}) + \mathbf{b}^F_j, \qquad (21) \\
= & \sum_{i=1}^{s} [\mathbf{\Lambda}^{oc(m)}_{\lambda,j,i} (\mathbf{W}^{ox}_{i,:} \mathbf{x}^{(m)} + \mathbf{W}^{oa}_{i,:} \mathbf{a}^{(m-1)} + \mathbf{b}^o_i) + \mathbf{\Lambda}^{oc(m)}_{\Delta,j,i} (\mathbf{f}^{(m)}_i \mathbf{c}^{(m-1)}_i + \mathbf{i}^{(m)}_i \mathbf{g}^{(m)}_i) + \mathbf{\Lambda}^{oc(m)}_{\varphi,j,i}] + \mathbf{b}^F_j, \\
= & \sum_{q_m=1}^{n} (\sum_{i=1}^{s} \mathbf{\Lambda}^{oc(m)}_{\lambda,j,i} \mathbf{W}^{ox}_{i,q_m}) \mathbf{x}^{(m)}_{q_m} + \sum_{r=1}^{s} (\sum_{i=1}^{s} \mathbf{\Lambda}^{oc(m)}_{\lambda,j,i} \mathbf{W}^{oa}_{i,r}) \mathbf{a}^{(m-1)}_r + \sum_{i=1}^{s} (\mathbf{\Lambda}^{oc(m)}_{\lambda,j,i} \mathbf{b}^o_i + \mathbf{\Lambda}^{oc(m)}_{\varphi,j,i}) \\
& + \sum_{\mathbf{\Lambda}^{oc(m)}_{\Delta,j,i} \ge 0} \mathbf{\Lambda}^{oc(m)}_{\Delta,j,i} (\sigma(\mathbf{y}^{f(m)}_i) \mathbf{c}^{(m-1)}_i + \sigma(\mathbf{y}^{i(m)}_i) \tanh(\mathbf{y}^{g(m)}_i)) \\
& + \sum_{\mathbf{\Lambda}^{oc(m)}_{\Delta,j,i} < 0} \mathbf{\Lambda}^{oc(m)}_{\Delta,j,i} (\sigma(\mathbf{y}^{f(m)}_i) \mathbf{c}^{(m-1)}_i + \sigma(\mathbf{y}^{i(m)}_i) \tanh(\mathbf{y}^{g(m)}_i)) + \mathbf{b}^F_j.
\end{aligned}
$$

*Assume the activation function $\sigma(\mathbf{y})\mathbf{x}$ is bounded by two linear functions $h^{fc(m)}_{L,i}(\mathbf{y}, \mathbf{x})$, $h^{fc(m)}_{U,i}(\mathbf{y}, \mathbf{x})$ and $\sigma(\mathbf{y}) \tanh(\mathbf{x})$ is bounded by two linear functions $h^{ig(m)}_{L,i}(\mathbf{y}, \mathbf{x})$, $h^{ig(m)}_{U,i}(\mathbf{y}, \mathbf{x})$, we have*

$$
\begin{aligned}
h^{fc(m)}_{L,i}(\mathbf{y}^{f(m)}_i, \mathbf{c}^{(m-1)}_i) \le \sigma(\mathbf{y}^{f(m)}_i) \mathbf{c}^{(m-1)}_i \le h^{fc(m)}_{U,i}(\mathbf{y}^{f(m)}_i, \mathbf{c}^{(m-1)}_i), \\
h^{ig(m)}_{L,i}(\mathbf{y}^{i(m)}_i, \mathbf{y}^{g(m)}_i) \le \sigma(\mathbf{y}^{i(m)}_i) \tanh(\mathbf{y}^{g(m)}_i) \le h^{ig(m)}_{U,i}(\mathbf{y}^{i(m)}_i, \mathbf{y}^{g(m)}_i)
\end{aligned}
$$

*We then have*

$$F_j(\mathbf{X}) \leq \sum_{q_m=1}^{n}(\sum_{i=1}^{s}\mathbf{\Lambda}^{oc(m)}_{\lambda,j,i}\mathbf{W}^{ox}_{i,q_m})\mathbf{x}^{(m)}_{q_m} + \sum_{r=1}^{s}(\sum_{i=1}^{s}\mathbf{\Lambda}^{oc(m)}_{\lambda,j,i}\mathbf{W}^{oa}_{i,r})\mathbf{a}^{(m-1)}_{r} + \sum_{i=1}^{s}(\mathbf{\Lambda}^{oc(m)}_{\lambda,j,i}\mathbf{b}^{o}_{i} + \mathbf{\Lambda}^{oc(m)}_{\varphi,j,i}) + \mathbf{b}^{F}_{j}$$
$$+ \sum_{\mathbf{\Lambda}^{oc(m)}_{\Delta,j,i}\geq 0}\mathbf{\Lambda}^{oc(m)}_{\Delta,j,i}(\alpha^{fc(m)}_{U,i}\mathbf{y}^{f(m)}_{i} + \beta^{fc(m)}_{U,i}\mathbf{c}^{(m-1)}_{i} + \gamma^{fc(m)}_{U,i} + \alpha^{ig(m)}_{U,i}\mathbf{y}^{i(m)}_{i} + \beta^{ig(m)}_{U,i}\mathbf{y}^{g(m)}_{i} + \gamma^{ig(m)}_{U,i})$$
$$+ \sum_{\mathbf{\Lambda}^{oc(m)}_{\Delta,j,i}< 0}\mathbf{\Lambda}^{oc(m)}_{\Delta,j,i}(\alpha^{fc(m)}_{L,i}\mathbf{y}^{f(m)}_{i} + \beta^{fc(m)}_{L,i}\mathbf{c}^{(m-1)}_{i} + \gamma^{fc(m)}_{L,i} + \alpha^{ig(m)}_{L,i}\mathbf{y}^{i(m)}_{i} + \beta^{ig(m)}_{L,i}\mathbf{y}^{g(m)}_{i} + \gamma^{ig(m)}_{L,i}).$$

*We then define* $\lambda^{fc(m)}_{j,i}$, $\mathbf{\Delta}^{fc(m)}_{j,i}$, $\varphi^{fc(m)}_{j,i}$,$\mathbf{\Lambda}^{ig(m)}_{\lambda,j,i}$, $\mathbf{\Lambda}^{ig(m)}_{\Delta,j,i}$ *and* $\mathbf{\Lambda}^{ig(m)}_{\varphi,j,i}$ *in the parentheses:*

$$\lambda^{fc(m)}_{j,i} = \begin{cases}\alpha^{fc(m)}_{U,i} & \textit{if } \mathbf{\Lambda}^{oc(m)}_{\Delta,j,i} \geq 0;\\ \alpha^{fc(m)}_{L,i} & \textit{if } \mathbf{\Lambda}^{oc(m)}_{\Delta,j,i} < 0;\end{cases} \quad \lambda^{ig(m)}_{j,i} = \begin{cases}\alpha^{ig(m)}_{U,i} & \textit{if } \mathbf{\Lambda}^{oc(m)}_{\Delta,j,i} \geq 0;\\ \alpha^{ig(m)}_{L,i} & \textit{if } \mathbf{\Lambda}^{oc(m)}_{\Delta,j,i} < 0;\end{cases}$$
$$\mathbf{\Delta}^{fc(m)}_{j,i} = \begin{cases}\beta^{fc(m)}_{U,i} & \textit{if } \mathbf{\Lambda}^{oc(m)}_{\Delta,j,i} \geq 0;\\ \beta^{fc(m)}_{L,i} & \textit{if } \mathbf{\Lambda}^{oc(m)}_{\Delta,j,i} < 0;\end{cases} \quad \mathbf{\Delta}^{ig(m)}_{j,i} = \begin{cases}\beta^{ig(m)}_{U,i} & \textit{if } \mathbf{\Lambda}^{oc(m)}_{\Delta,j,i} \geq 0;\\ \beta^{ig(m)}_{L,i} & \textit{if } \mathbf{\Lambda}^{oc(m)}_{\Delta,j,i} < 0;\end{cases}$$
$$\varphi^{fc(m)}_{j,i} = \begin{cases}\gamma^{fc(m)}_{U,i} & \textit{if } \mathbf{\Lambda}^{oc(m)}_{\Delta,j,i} \geq 0;\\ \gamma^{fc(m)}_{L,i} & \textit{if } \mathbf{\Lambda}^{oc(m)}_{\Delta,j,i} < 0;\end{cases} \quad \varphi^{ig(m)}_{j,i} = \begin{cases}\gamma^{ig(m)}_{U,i} & \textit{if } \mathbf{\Lambda}^{oc(m)}_{\Delta,j,i} \geq 0;\\ \gamma^{ig(m)}_{L,i} & \textit{if } \mathbf{\Lambda}^{oc(m)}_{\Delta,j,i} < 0;\end{cases}$$

*and obtain*

$$F_j(\mathbf{X}) \leq \sum_{q_m=1}^{n}(\sum_{i=1}^{s}\mathbf{\Lambda}^{oc(m)}_{\lambda,j,i}\mathbf{W}^{ox}_{i,q_m})\mathbf{x}^{(m)}_{q_m} + \sum_{r=1}^{s}(\sum_{i=1}^{s}\mathbf{\Lambda}^{oc(m)}_{\lambda,j,i}\mathbf{W}^{oa}_{i,r})\mathbf{a}^{(m-1)}_{r} + \sum_{i=1}^{s}(\mathbf{\Lambda}^{oc(m)}_{\lambda,j,i}\mathbf{b}^{o}_{i} + \mathbf{\Lambda}^{oc(m)}_{\varphi,j,i}) + \mathbf{b}^{F}_{j}$$
$$+ \sum_{i=1}^{s}\mathbf{\Lambda}^{oc(m)}_{\Delta,j,i}(\lambda^{fc(m)}_{j,i}\mathbf{y}^{f(m)}_{i} + \mathbf{\Delta}^{fc(m)}_{j,i}\mathbf{c}^{(m-1)}_{i} + \varphi^{fc(m)}_{j,i} + \lambda^{ig(m)}_{j,i}\mathbf{y}^{i(m)}_{i} + \mathbf{\Delta}^{ig(m)}_{j,i}\mathbf{y}^{g(m)}_{i} + \varphi^{ig(m)}_{j,i}).$$

*We further define*

$$\mathbf{\Lambda}^{fc(m)}_{\lambda,j,i} := \mathbf{\Lambda}^{oc(m)}_{\Delta,j,i}\ \lambda^{fc(m)}_{j,i}; \mathbf{\Lambda}^{fc(m)}_{\Delta,j,i} := \mathbf{\Lambda}^{oc(m)}_{\Delta,j,i}\ \mathbf{\Delta}^{fc(m)}_{j,i}; \mathbf{\Lambda}^{fc(m)}_{\varphi,j,i} := \mathbf{\Lambda}^{oc(m)}_{\Delta,j,i}\ \varphi^{fc(m)}_{j,i};$$
$$\mathbf{\Lambda}^{ig(m)}_{\lambda,j,i} := \mathbf{\Lambda}^{oc(m)}_{\Delta,j,i}\ \lambda^{ig(m)}_{j,i}; \mathbf{\Lambda}^{ig(m)}_{\Delta,j,i} := \mathbf{\Lambda}^{oc(m)}_{\Delta,j,i}\ \mathbf{\Delta}^{ig(m)}_{j,i}; \mathbf{\Lambda}^{ig(m)}_{\varphi,j,i} := \mathbf{\Lambda}^{oc(m)}_{\Delta,j,i}\ \varphi^{ig(m)}_{j,i};$$

*and obtain*

$$F_j(\mathbf{X}) \leq \sum_{q_m=1}^{n}(\sum_{i=1}^{s}\mathbf{\Lambda}^{oc(m)}_{\lambda,j,i}\mathbf{W}^{ox}_{i,q_m})\mathbf{x}^{(m)}_{q_m} + \sum_{r=1}^{s}(\sum_{i=1}^{s}\mathbf{\Lambda}^{oc(m)}_{\lambda,j,i}\mathbf{W}^{oa}_{i,r})\mathbf{a}^{(m-1)}_{r} + \sum_{i=1}^{s}(\mathbf{\Lambda}^{oc(m)}_{\lambda,j,i}\mathbf{b}^{o}_{i} + \mathbf{\Lambda}^{oc(m)}_{\varphi,j,i}) + \mathbf{b}^{F}_{j}$$
$$+ \sum_{i=1}^{s}(\mathbf{\Lambda}^{fc(m)}_{\lambda,j,i}\mathbf{y}^{f(m)}_{i} + \mathbf{\Lambda}^{fc(m)}_{\Delta,j,i}\mathbf{c}^{(m-1)}_{i} + \mathbf{\Lambda}^{fc(m)}_{\varphi,j,i} + \mathbf{\Lambda}^{ig(m)}_{\lambda,j,i}\mathbf{y}^{i(m)}_{i} + \mathbf{\Lambda}^{ig(m)}_{\Delta,j,i}\mathbf{y}^{g(m)}_{i} + \mathbf{\Lambda}^{ig(m)}_{\varphi,j,i})$$
$$= \sum_{q_m=1}^{n}(\sum_{i=1}^{s}\mathbf{\Lambda}^{oc(m)}_{\lambda,j,i}\mathbf{W}^{ox}_{i,q_m})\mathbf{x}^{(m)}_{q_m} + \sum_{r=1}^{s}(\sum_{i=1}^{s}\mathbf{\Lambda}^{oc(m)}_{\lambda,j,i}\mathbf{W}^{oa}_{i,r})\mathbf{a}^{(m-1)}_{r} + \sum_{i=1}^{s}(\mathbf{\Lambda}^{oc(m)}_{\lambda,j,i}\mathbf{b}^{o}_{i} + \mathbf{\Lambda}^{oc(m)}_{\varphi,j,i}) + \mathbf{b}^{F}_{j}$$
$$+ \sum_{i=1}^{s}[\mathbf{\Lambda}^{fc(m)}_{\lambda,j,i}(\mathbf{W}^{fx}_{i,:}\mathbf{x}^{(m)} + \mathbf{W}^{fa}_{i,:}\mathbf{a}^{(m-1)} + \mathbf{b}^{f}_{i}) + \mathbf{\Lambda}^{fc(m)}_{\Delta,j,i}\mathbf{c}^{(m-1)}_{i} + \mathbf{\Lambda}^{fc(m)}_{\varphi,j,i}$$
$$+ \mathbf{\Lambda}^{ig(m)}_{\lambda,j,i}(\mathbf{W}^{ix}_{i,:}\mathbf{x}^{(m)} + \mathbf{W}^{ia}_{i,:}\mathbf{a}^{(m-1)} + \mathbf{b}^{i}_{i}) + \mathbf{\Lambda}^{ig(m)}_{\Delta,j,i}(\mathbf{W}^{gx}_{i,:}\mathbf{x}^{(m)} + \mathbf{W}^{ga}_{i,:}\mathbf{a}^{(m-1)} + \mathbf{b}^{g}_{i}) + \mathbf{\Lambda}^{ig(m)}_{\varphi,j,i}]$$
$$= \sum_{q_m=1}^{n}(\mathbf{\Lambda}^{oc(m)}_{\lambda,j,:}\mathbf{W}^{ox}_{:,q_m} + \mathbf{\Lambda}^{fc(m)}_{\lambda,j,:}\mathbf{W}^{fx}_{:,q_m} + \mathbf{\Lambda}^{ig(m)}_{\lambda,j,:}\mathbf{W}^{ix}_{:,q_m} + \mathbf{\Lambda}^{ig(m)}_{\Delta,j,:}\mathbf{W}^{gx}_{:,q_m})\mathbf{x}^{(m)}_{q_m}$$
$$+ \sum_{r=1}^{s}(\mathbf{\Lambda}^{oc(m)}_{\lambda,j,:}\mathbf{W}^{oa}_{:,r} + \mathbf{\Lambda}^{fc(m)}_{\lambda,j,:}\mathbf{W}^{fa}_{:,r} + \mathbf{\Lambda}^{ig(m)}_{\lambda,j,:}\mathbf{W}^{ia}_{:,r} + \mathbf{\Lambda}^{ig(m)}_{\Delta,j,:}\mathbf{W}^{ga}_{:,r})\mathbf{a}^{(m-1)}_{r}$$

$$+ \mathbf{\Lambda}^{oc(m)}_{\lambda,j,:}\mathbf{b}^o + \mathbf{\Lambda}^{fc(m)}_{\lambda,j,:}\mathbf{b}^f + \mathbf{\Lambda}^{ig(m)}_{\lambda,j,:}\mathbf{b}^i + \mathbf{\Lambda}^{ig(m)}_{\Delta,j,:}\mathbf{b}^g + \sum_{i=1}^{s}(\mathbf{\Lambda}^{oc(m)}_{\varphi,j,i} + \mathbf{\Lambda}^{fc(m)}_{\varphi,j,i} + \mathbf{\Lambda}^{ig(m)}_{\varphi,j,i}) + \mathbf{b}^F_j$$
$$+ \mathbf{\Lambda}^{fc(m)}_{\Delta,j,:}\mathbf{c}^{(m-1)}. \tag{22}$$

*We combine coefficients in Equation* (22) *into equivalent weights* $\tilde{\mathbf{W}}^{x(m)}_{U,j,q_m}$, $\tilde{\mathbf{W}}^{a(m)}_{U,j,r}$ *and bias* $\tilde{\mathbf{b}}^{(m)}_{U,j}$ *as defined by*

$$\begin{aligned}
\tilde{\mathbf{W}}^{x(m)}_{U,j,q_m} &= \mathbf{\Lambda}^{oc(m)}_{\lambda,j,:}\mathbf{W}^{ox}_{:,q_m} + \mathbf{\Lambda}^{fc(m)}_{\lambda,j,:}\mathbf{W}^{fx}_{:,q_m} + \mathbf{\Lambda}^{ig(m)}_{\lambda,j,:}\mathbf{W}^{ix}_{:,q_m} + \mathbf{\Lambda}^{ig(m)}_{\Delta,j,:}\mathbf{W}^{gx}_{:,q_m},\\
\tilde{\mathbf{W}}^{a(m)}_{U,j,r} &= \mathbf{\Lambda}^{oc(m)}_{\lambda,j,:}\mathbf{W}^{oa}_{:,r} + \mathbf{\Lambda}^{fc(m)}_{\lambda,j,:}\mathbf{W}^{fa}_{:,r} + \mathbf{\Lambda}^{ig(m)}_{\lambda,j,:}\mathbf{W}^{ia}_{:,r} + \mathbf{\Lambda}^{ig(m)}_{\Delta,j,:}\mathbf{W}^{ga}_{:,r},\\
\tilde{\mathbf{b}}^{(m)}_{U,j} &= \mathbf{\Lambda}^{oc(m)}_{\lambda,j,:}\mathbf{b}^o + \mathbf{\Lambda}^{fc(m)}_{\lambda,j,:}\mathbf{b}^f + \mathbf{\Lambda}^{ig(m)}_{\lambda,j,:}\mathbf{b}^i + \mathbf{\Lambda}^{ig(m)}_{\Delta,j,:}\mathbf{b}^g + \sum_{i=1}^{s}(\mathbf{\Lambda}^{oc(m)}_{\varphi,j,i} + \mathbf{\Lambda}^{fc(m)}_{\varphi,j,i} + \mathbf{\Lambda}^{ig(m)}_{\varphi,j,i}),
\end{aligned}$$

*and obtain*

$$\begin{aligned}
F_j(\mathbf{X}) \le F^{U,m}_j(\mathbf{X}) &= \tilde{\mathbf{W}}^{x(m)}_{U,j,:}\mathbf{x}^{(m)} + \tilde{\mathbf{W}}^{a(m)}_{U,j,:}\mathbf{a}^{(m-1)} + \mathbf{\Lambda}^{fc(m)}_{\Delta,j,:}\mathbf{c}^{(m-1)} + \tilde{\mathbf{b}}^{(m)}_{U,j} + \mathbf{b}^F_j, \qquad (23)\\
&= \tilde{\mathbf{W}}^{x(m)}_{U,j,:}\mathbf{x}^{(m)} + \tilde{\mathbf{b}}^{(m)}_{U,j} + \mathbf{b}^F_j + \mathbf{\Lambda}^{fc(m)}_{\Delta,j,:}\mathbf{c}^{(m-1)} + \tilde{\mathbf{W}}^{a(m)}_{U,j,:}[\mathbf{o}^{(m-1)}\tanh(\mathbf{c}^{(m-1)})]\\
&= \tilde{\mathbf{W}}^{x(m)}_{U,j,:}\mathbf{x}^{(m)} + \tilde{\mathbf{b}}^{(m)}_{U,j} + \mathbf{b}^F_j + \mathbf{\Lambda}^{fc(m)}_{\Delta,j,:}\mathbf{c}^{(m-1)}\\
&+ \sum_{\tilde{\mathbf{W}}^{a(m)}_{U,j,i}\ge 0}\tilde{\mathbf{W}}^{a(m)}_{U,j,i}[\sigma(\mathbf{y}^{o(m-1)}_i)\tanh(\mathbf{c}^{(m-1)}_i)] + \sum_{\tilde{\mathbf{W}}^{a(m)}_{U,j,i}< 0}\tilde{\mathbf{W}}^{a(m)}_{U,j,i}[\sigma(\mathbf{y}^{o(m-1)}_i)\tanh(\mathbf{c}^{(m-1)}_i)].
\end{aligned}$$

*Assume the activation function* $\sigma(\mathbf{y})\tanh(\mathbf{x})$ *is bounded by two linear functions* $h^{oc(m)}_{L,i}(\mathbf{y},\mathbf{x})$, $h^{oc(m)}_{U,i}(\mathbf{y},\mathbf{x})$*, we have*

$$h^{oc(m-1)}_{L,i}(\mathbf{y}^{o(m-1)}_i, \mathbf{c}^{(m-1)}_i) \le \sigma(\mathbf{y}^{o(m-1)}_i)\tanh(\mathbf{c}^{(m-1)}_i) \le h^{oc(m-1)}_{U,i}(\mathbf{y}^{o(m-1)}_i, \mathbf{c}^{(m-1)}_i).$$

*We can then obtain*

$$\begin{aligned}
F^{U,m}_j(\mathbf{X}) \le\ & \tilde{\mathbf{W}}^{x(m)}_{U,j,:}\mathbf{x}^{(m)} + \tilde{\mathbf{b}}^{(m)}_{U,j} + \mathbf{b}^F_j + \mathbf{\Lambda}^{fc(m)}_{\Delta,j,:}\mathbf{c}^{(m-1)}\\
&+ \sum_{\tilde{\mathbf{W}}^{a(m)}_{U,j,i}\ge 0}\tilde{\mathbf{W}}^{a(m)}_{U,j,i}\ (\alpha^{oc(m-1)}_{U,i}\mathbf{y}^{o(m-1)}_i + \beta^{oc(m-1)}_{U,i}\mathbf{c}^{(m-1)}_i + \gamma^{oc(m-1)}_{U,i})\\
&+ \sum_{\tilde{\mathbf{W}}^{a(m)}_{U,j,i}< 0}\tilde{\mathbf{W}}^{a(m)}_{U,j,i}\ (\alpha^{oc(m-1)}_{L,i}\mathbf{y}^{o(m-1)}_i + \beta^{oc(m-1)}_{L,i}\mathbf{c}^{(m-1)}_i + \gamma^{oc(m-1)}_{L,i}).
\end{aligned}$$

*We then define* $\lambda^{oc(m-1)}_{j,i}$, $\mathbf{\Delta}^{oc(m-1)}_{j,i}$ *and* $\varphi^{oc(m-1)}_{j,i}$ *in the parentheses:*

$$\begin{aligned}
\lambda^{oc(m-1)}_{j,i} &= \begin{cases}\alpha^{oc(m-1)}_{U,i} & \textit{if}\ \ \tilde{\mathbf{W}}^{a(m)}_{U,j,i} \ge 0;\\ \alpha^{oc(m-1)}_{L,i} & \textit{if}\ \ \tilde{\mathbf{W}}^{a(m)}_{U,j,i} < 0;\end{cases}\\
\mathbf{\Delta}^{oc(m-1)}_{j,i} &= \begin{cases}\beta^{oc(m-1)}_{U,i} & \textit{if}\ \ \tilde{\mathbf{W}}^{a(m)}_{U,j,i} \ge 0;\\ \beta^{oc(m-1)}_{L,i} & \textit{if}\ \ \tilde{\mathbf{W}}^{a(m)}_{U,j,i} < 0;\end{cases}\\
\varphi^{oc(m-1)}_{j,i} &= \begin{cases}\gamma^{oc(m-1)}_{U,i} & \textit{if}\ \ \tilde{\mathbf{W}}^{a(m)}_{U,j,i} \ge 0;\\ \gamma^{oc(m-1)}_{L,i} & \textit{if}\ \ \tilde{\mathbf{W}}^{a(m)}_{U,j,i} < 0;\end{cases}
\end{aligned}$$

*and obtain*

$$\begin{aligned}
F^{U,m}_j(\mathbf{X}) \le\ & \tilde{\mathbf{W}}^{x(m)}_{U,j,:}\mathbf{x}^{(m)} + \tilde{\mathbf{b}}^{(m)}_{U,j} + \mathbf{b}^F_j + \mathbf{\Lambda}^{fc(m)}_{\Delta,j,:}\mathbf{c}^{(m-1)}\\
&+ \sum_{i=1}^{s}\tilde{\mathbf{W}}^{a(m)}_{U,j,i}\ (\lambda^{oc(m-1)}_{j,i}\mathbf{y}^{o(m-1)}_i + \mathbf{\Delta}^{oc(m-1)}_{j,i}\mathbf{c}^{(m-1)}_i + \varphi^{oc(m-1)}_{j,i}).
\end{aligned}$$

*We further let*

$$\mathbf{\Lambda}_{\lambda,j,i}^{oc(m-1)} := \tilde{\mathbf{W}}_{U,j,i}^{a(m)}\ \lambda_{j,i}^{oc(m-1)}, \mathbf{\Lambda}_{\Delta,j,i}^{oc(m-1)} := \tilde{\mathbf{W}}_{U,j,i}^{a(m)}\ \mathbf{\Delta}_{j,i}^{oc(m-1)} + \mathbf{\Lambda}_{\Delta,j,i}^{fc(m)}, \mathbf{\Lambda}_{\varphi,j,i}^{oc(m-1)} := \tilde{\mathbf{W}}_{U,j,i}^{a(m)}\ \varphi_{j,i}^{oc(m-1)},$$

*and we have*

$$F_j^{U,m}(\mathbf{X}) \leq \tilde{\mathbf{W}}_{U,j,:}^{x(m)}\mathbf{x}^{(m)} + \tilde{\mathbf{b}}_{U,j}^{(m)} + \sum_{i=1}^{s}(\mathbf{\Lambda}_{\lambda,j,i}^{oc(m-1)}\mathbf{y}_i^{o(m-1)} + \mathbf{\Lambda}_{\Delta,j,i}^{oc(m-1)}\mathbf{c}_i^{(m-1)} + \mathbf{\Lambda}_{\varphi,j,i}^{oc(m-1)}) + \mathbf{b}_j^F. \tag{24}$$

*Notice that Equation* (21) *and Equation* (24) *are in similar forms. Thus,* $\forall r \in s$ *we can define variables as follows:*

$$\lambda_{j,i}^{fc(m-1)} = \begin{cases} \alpha_{U,i}^{fc(m-1)} & \textit{if } \mathbf{\Lambda}_{\Delta,j,i}^{oc(m-1)} \geq 0; \\ \alpha_{L,i}^{fc(m-1)} & \textit{if } \mathbf{\Lambda}_{\Delta,j,i}^{oc(m-1)} < 0; \end{cases} \quad \lambda_{j,i}^{ig(m-1)} = \begin{cases} \alpha_{U,i}^{ig(m-1)} & \textit{if } \mathbf{\Lambda}_{\Delta,j,i}^{oc(m-1)} \geq 0; \\ \alpha_{L,i}^{ig(m-1)} & \textit{if } \mathbf{\Lambda}_{\Delta,j,i}^{oc(m-1)} < 0; \end{cases}$$

$$\mathbf{\Delta}_{j,i}^{fc(m-1)} = \begin{cases} \beta_{U,i}^{fc(m-1)} & \textit{if } \mathbf{\Lambda}_{\Delta,j,i}^{oc(m-1)} \geq 0; \\ \beta_{L,i}^{fc(m-1)} & \textit{if } \mathbf{\Lambda}_{\Delta,j,i}^{oc(m-1)} < 0; \end{cases} \quad \mathbf{\Delta}_{j,i}^{ig(m-1)} = \begin{cases} \beta_{U,i}^{ig(m-1)} & \textit{if } \mathbf{\Lambda}_{\Delta,j,i}^{oc(m-1)} \geq 0; \\ \beta_{L,i}^{ig(m-1)} & \textit{if } \mathbf{\Lambda}_{\Delta,j,i}^{oc(m-1)} < 0; \end{cases}$$

$$\varphi_{j,i}^{fc(m-1)} = \begin{cases} \gamma_{U,i}^{fc(m-1)} & \textit{if } \mathbf{\Lambda}_{\Delta,j,i}^{oc(m-1)} \geq 0; \\ \gamma_{L,i}^{fc(m-1)} & \textit{if } \mathbf{\Lambda}_{\Delta,j,i}^{oc(m-1)} < 0; \end{cases} \quad \varphi_{j,i}^{ig(m-1)} = \begin{cases} \gamma_{U,i}^{ig(m-1)} & \textit{if } \mathbf{\Lambda}_{\Delta,j,i}^{oc(m-1)} \geq 0; \\ \gamma_{L,i}^{ig(m-1)} & \textit{if } \mathbf{\Lambda}_{\Delta,j,i}^{oc(m-1)} < 0; \end{cases}$$

$$\mathbf{\Lambda}_{\lambda,j,i}^{fc(m-1)} := \mathbf{\Lambda}_{\Delta,j,i}^{oc(m-1)}\ \lambda_{j,i}^{fc(m-1)}; \mathbf{\Lambda}_{\Delta,j,i}^{fc(m-1)} := \mathbf{\Lambda}_{\Delta,j,i}^{oc(m-1)}\ \mathbf{\Delta}_{j,i}^{fc(m-1)}; \mathbf{\Lambda}_{\varphi,j,i}^{fc(m-1)} := \mathbf{\Lambda}_{\Delta,j,i}^{oc(m-1)}\ \varphi_{j,i}^{fc(m-1)};$$

$$\mathbf{\Lambda}_{\lambda,j,i}^{ig(m-1)} := \mathbf{\Lambda}_{\Delta,j,i}^{oc(m-1)}\ \lambda_{j,i}^{ig(m-1)}; \mathbf{\Lambda}_{\Delta,j,i}^{ig(m-1)} := \mathbf{\Lambda}_{\Delta,j,i}^{oc(m-1)}\ \mathbf{\Delta}_{j,i}^{ig(m-1)}; \mathbf{\Lambda}_{\varphi,j,i}^{ig(m-1)} := \mathbf{\Lambda}_{\Delta,j,i}^{oc(m-1)}\ \varphi_{j,i}^{ig(m-1)};$$

$$\tilde{\mathbf{W}}_{U,j,q_{m-1}}^{x(m-1)} = \mathbf{\Lambda}_{\lambda,j,:}^{oc(m-1)}\mathbf{W}_{:,q_{m-1}}^{ox} + \mathbf{\Lambda}_{\lambda,j,:}^{fc(m-1)}\mathbf{W}_{:,q_{m-1}}^{fx} + \mathbf{\Lambda}_{\lambda,j,:}^{ig(m-1)}\mathbf{W}_{:,q_{m-1}}^{ix} + \mathbf{\Lambda}_{\Delta,j,:}^{ig(m-1)}\mathbf{W}_{:,q_{m-1}}^{gx};$$

$$\tilde{\mathbf{W}}_{U,j,r}^{a(m-1)} = \mathbf{\Lambda}_{\lambda,j,:}^{oc(m-1)}\mathbf{W}_{:,r}^{oa} + \mathbf{\Lambda}_{\lambda,j,:}^{fc(m-1)}\mathbf{W}_{:,r}^{fa} + \mathbf{\Lambda}_{\lambda,j,:}^{ig(m-1)}\mathbf{W}_{:,r}^{ia} + \mathbf{\Lambda}_{\Delta,j,:}^{ig(m-1)}\mathbf{W}_{:,r}^{ga};$$

$$\tilde{\mathbf{b}}_{U,j}^{(m-1)} = \mathbf{\Lambda}_{\lambda,j,:}^{oc(m-1)}\mathbf{b}^o + \mathbf{\Lambda}_{\lambda,j,:}^{fc(m-1)}\mathbf{b}^f + \mathbf{\Lambda}_{\lambda,j,:}^{ig(m-1)}\mathbf{b}^i + \mathbf{\Lambda}_{\Delta,j,:}^{ig(m-1)}\mathbf{b}^g + \sum_{i=1}^{s}(\mathbf{\Lambda}_{\varphi,j,i}^{oc(m-1)} + \mathbf{\Lambda}_{\varphi,j,i}^{fc(m-1)} + \mathbf{\Lambda}_{\varphi,j,i}^{ig(m-1)}).$$

*Then we can obtain equation similar to Equation* (3)*:*

$$\begin{aligned} F_j^{U,m}(\mathbf{X}) \leq F_j^{U,m-1}(\mathbf{X}) &= \tilde{\mathbf{W}}_{U,j,:}^{x(m)}\mathbf{x}^{(m)} + \tilde{\mathbf{W}}_{U,j,:}^{x(m-1)}\mathbf{x}^{(m-1)} + \tilde{\mathbf{W}}_{U,j,:}^{a(m-1)}\mathbf{a}^{(m-2)} \\ &+ \mathbf{\Lambda}_{\Delta,j,:}^{fc(m-1)}\mathbf{c}^{(m-2)} + \tilde{\mathbf{b}}_{U,j}^{(m)} + \tilde{\mathbf{b}}_{U,j}^{(m-1)} + \mathbf{b}_j^F. \end{aligned}$$

*Thus, we can repeat the above procedure iteratively until we obtain the final upper bound* $F_j^{U,1}(\mathbf{X})$*, where* $F_j(\mathbf{X}) \leq F_j^{U,m}(\mathbf{X}) \leq \cdots \leq F_j^{U,1}(\mathbf{X})$*. We let* $F_j^U(\mathbf{X})$ *denote the final upper bound* $F_j^{U,1}(\mathbf{X})$*, and we have*

$$F_j^U(\mathbf{X}) = \tilde{\mathbf{W}}_{U,j,:}^{a(1)}\mathbf{a}^{(0)} + \mathbf{\Lambda}_{\Delta,j,:}^{fc(1)}\mathbf{c}^{(0)} + \sum_{k=1}^{m}\tilde{\mathbf{W}}_{U,j,:}^{x(k)}\mathbf{x}^{(k)} + \sum_{k=1}^{m}\tilde{\mathbf{b}}_{U,j}^{(k)} + \mathbf{b}_j^F,$$

*where*

$$\begin{aligned} \tilde{\mathbf{W}}_{U,j,q_k}^{x(k)} &= \mathbf{\Lambda}_{\lambda,j,:}^{oc(k)}\mathbf{W}_{:,q_k}^{ox} + \mathbf{\Lambda}_{\lambda,j,:}^{fc(k)}\mathbf{W}_{:,q_k}^{fx} + \mathbf{\Lambda}_{\lambda,j,:}^{ig(k)}\mathbf{W}_{:,q_k}^{ix} + \mathbf{\Lambda}_{\Delta,j,:}^{ig(k)}\mathbf{W}_{:,q_k}^{gx}, \\ \tilde{\mathbf{W}}_{U,j,r}^{a(k)} &= \mathbf{\Lambda}_{\lambda,j,:}^{oc(k)}\mathbf{W}_{:,r}^{oa} + \mathbf{\Lambda}_{\lambda,j,:}^{fc(k)}\mathbf{W}_{:,r}^{fa} + \mathbf{\Lambda}_{\lambda,j,:}^{ig(k)}\mathbf{W}_{:,r}^{ia} + \mathbf{\Lambda}_{\Delta,j,:}^{ig(k)}\mathbf{W}_{:,r}^{ga}, \\ \tilde{\mathbf{b}}_{U,j}^{(k)} &= \mathbf{\Lambda}_{\lambda,j,:}^{oc(k)}\mathbf{b}^o + \mathbf{\Lambda}_{\lambda,j,:}^{fc(k)}\mathbf{b}^f + \mathbf{\Lambda}_{\lambda,j,:}^{ig(k)}\mathbf{b}^i + \mathbf{\Lambda}_{\Delta,j,:}^{ig(k)}\mathbf{b}^g + \sum_{i=1}^{s}(\mathbf{\Lambda}_{\varphi,j,i}^{oc(k)} + \mathbf{\Lambda}_{\varphi,j,i}^{fc(k)} + \mathbf{\Lambda}_{\varphi,j,i}^{ig(k)}), \end{aligned}$$

*and (*$\odot$ *is the Hadamard product)*

$$\mathbf{\Lambda}_{\lambda,j,:}^{oc(k)} = \begin{cases} \mathbf{W}_{j,:}^{Fa} \odot \lambda_{j,:}^{oc(k)} & \textit{if } k = m; \\ \tilde{\mathbf{W}}_{U,j,:}^{a(k+1)} \odot \lambda_{j,:}^{oc(k)} & \textit{if } k \in [m-1]; \end{cases}$$

$$\mathbf{\Lambda}_{\Delta,j,:}^{oc(k)} = \begin{cases} \mathbf{W}_{j,:}^{Fa} \odot \mathbf{\Delta}_{j,:}^{oc(k)} & \textit{if } k = m; \\ \tilde{\mathbf{W}}_{U,j,:}^{a(k+1)} \odot \mathbf{\Delta}_{j,:}^{oc(k)} + \mathbf{\Lambda}_{\Delta,j,:}^{fc(k+1)} & \textit{if } k \in [m-1]; \end{cases}$$

$$\mathbf{\Lambda}_{\varphi,j,:}^{oc(k)} = \begin{cases} \mathbf{W}_{j,:}^{Fa} \odot \varphi_{j,:}^{oc(k)} & \textit{if } k = m; \\ \tilde{\mathbf{W}}_{U,j,:}^{a(k+1)} \odot \varphi_{j,:}^{oc(k)} & \textit{if } k \in [m-1]; \end{cases}$$

$$\begin{aligned}
\mathbf{\Lambda}^{fc(k)}_{\lambda,j,:} &= \mathbf{\Lambda}^{oc(k)}_{\Delta,j,:} \odot \lambda^{fc(k)}_{j,:} \quad \textit{if} \quad k \in [m]; & \mathbf{\Lambda}^{ig(k)}_{\lambda,j,:} &= \mathbf{\Lambda}^{oc(k)}_{\Delta,j,:} \odot \lambda^{ig(k)}_{j,:} \quad \textit{if} \quad k \in [m];\\
\mathbf{\Lambda}^{fc(k)}_{\Delta,j,:} &= \mathbf{\Lambda}^{oc(k)}_{\Delta,j,:} \odot \mathbf{\Delta}^{fc(k)}_{j,:} \quad \textit{if} \quad k \in [m]; & \mathbf{\Lambda}^{ig(k)}_{\Delta,j,:} &= \mathbf{\Lambda}^{oc(k)}_{\Delta,j,:} \odot \mathbf{\Delta}^{ig(k)}_{j,:} \quad \textit{if} \quad k \in [m];\\
\mathbf{\Lambda}^{fc(k)}_{\varphi,j,:} &= \mathbf{\Lambda}^{oc(k)}_{\Delta,j,:} \odot \varphi^{fc(k)}_{j,:} \quad \textit{if} \quad k \in [m]; & \mathbf{\Lambda}^{ig(k)}_{\varphi,j,:} &= \mathbf{\Lambda}^{oc(k)}_{\Delta,j,:} \odot \varphi^{ig(k)}_{j,:} \quad \textit{if} \quad k \in [m];
\end{aligned}$$

*and* $\forall r \in s$,

$$\lambda^{oc(m)}_{j,r} = \begin{cases} \alpha^{oc(m)}_{U,r} & \textit{if} \;\; \mathbf{W}^{Fa}_{j,r} \geq 0;\\ \alpha^{oc(m)}_{L,r} & \textit{if} \;\; \mathbf{W}^{Fa}_{j,r} < 0; \end{cases} \quad \mathbf{\Delta}^{oc(m)}_{j,r} = \begin{cases} \beta^{oc(m)}_{U,r} & \textit{if} \;\; \mathbf{W}^{Fa}_{j,r} \geq 0;\\ \beta^{oc(m)}_{L,r} & \textit{if} \;\; \mathbf{W}^{Fa}_{j,r} < 0; \end{cases} \quad \varphi^{oc(m)}_{j,r} = \begin{cases} \gamma^{oc(m)}_{U,r} & \textit{if} \;\; \mathbf{W}^{Fa}_{j,r} \geq 0;\\ \gamma^{oc(m)}_{L,r} & \textit{if} \;\; \mathbf{W}^{Fa}_{j,r} < 0; \end{cases}$$

*and* $\forall r \in s, k \in [m-1]$,

$$\begin{aligned}
\lambda^{oc(k)}_{j,r} &= \begin{cases} \alpha^{oc(k)}_{U,r} & \textit{if} \;\; \tilde{\mathbf{W}}^{a(k+1)}_{U,j,r} \geq 0;\\ \alpha^{oc(k)}_{L,r} & \textit{if} \;\; \tilde{\mathbf{W}}^{a(k+1)}_{U,j,r} < 0; \end{cases}\\
\mathbf{\Delta}^{oc(k)}_{j,r} &= \begin{cases} \beta^{oc(k)}_{U,r} & \textit{if} \;\; \tilde{\mathbf{W}}^{a(k+1)}_{U,j,r} \geq 0;\\ \beta^{oc(k)}_{L,r} & \textit{if} \;\; \tilde{\mathbf{W}}^{a(k+1)}_{U,j,r} < 0; \end{cases}\\
\varphi^{oc(k)}_{j,r} &= \begin{cases} \gamma^{oc(k)}_{U,r} & \textit{if} \;\; \tilde{\mathbf{W}}^{a(k+1)}_{U,j,r} \geq 0;\\ \gamma^{oc(k)}_{L,r} & \textit{if} \;\; \tilde{\mathbf{W}}^{a(k+1)}_{U,j,r} < 0; \end{cases}
\end{aligned}$$

*and* $\forall r \in s, k \in [m]$,

$$\begin{aligned}
\lambda^{fc(k)}_{j,r} &= \begin{cases} \alpha^{fc(k)}_{U,r} & \textit{if} \;\; \mathbf{\Lambda}^{oc(k)}_{\Delta,j,r} \geq 0;\\ \alpha^{fc(k)}_{L,r} & \textit{if} \;\; \mathbf{\Lambda}^{oc(k)}_{\Delta,j,r} < 0; \end{cases} & \lambda^{ig(k)}_{j,r} &= \begin{cases} \alpha^{ig(k)}_{U,r} & \textit{if} \;\; \mathbf{\Lambda}^{oc(k)}_{\Delta,j,r} \geq 0;\\ \alpha^{ig(k)}_{L,r} & \textit{if} \;\; \mathbf{\Lambda}^{oc(k)}_{\Delta,j,r} < 0; \end{cases}\\
\mathbf{\Delta}^{fc(k)}_{j,r} &= \begin{cases} \beta^{fc(k)}_{U,r} & \textit{if} \;\; \mathbf{\Lambda}^{oc(k)}_{\Delta,j,r} \geq 0;\\ \beta^{fc(k)}_{L,r} & \textit{if} \;\; \mathbf{\Lambda}^{oc(k)}_{\Delta,j,r} < 0; \end{cases} & \mathbf{\Delta}^{ig(k)}_{j,r} &= \begin{cases} \beta^{ig(k)}_{U,r} & \textit{if} \;\; \mathbf{\Lambda}^{oc(k)}_{\Delta,j,r} \geq 0;\\ \beta^{ig(k)}_{L,r} & \textit{if} \;\; \mathbf{\Lambda}^{oc(k)}_{\Delta,j,r} < 0; \end{cases}\\
\varphi^{fc(k)}_{j,r} &= \begin{cases} \gamma^{fc(k)}_{U,r} & \textit{if} \;\; \mathbf{\Lambda}^{oc(k)}_{\Delta,j,r} \geq 0;\\ \gamma^{fc(k)}_{L,r} & \textit{if} \;\; \mathbf{\Lambda}^{oc(k)}_{\Delta,j,r} < 0; \end{cases} & \varphi^{ig(k)}_{j,r} &= \begin{cases} \gamma^{ig(k)}_{U,r} & \textit{if} \;\; \mathbf{\Lambda}^{oc(k)}_{\Delta,j,r} \geq 0;\\ \gamma^{ig(k)}_{L,r} & \textit{if} \;\; \mathbf{\Lambda}^{oc(k)}_{\Delta,j,r} < 0. \end{cases}
\end{aligned}$$

***Lower bound.*** *The above derivations of upper bound can be applied similarly to derive lower bounds of* $F_j(\mathbf{X})$*, and the only difference is now we need to use the left-hand side of inequities (rather than right-hand side when deriving upper bound) to bound the activated terms. Thus, following the same procedure in deriving the upper bounds, we can iteratively unwrap the activation functions and obtain a final lower bound* $F_j^{L,1}(\mathbf{X})$*, where* $F_j(\mathbf{X}) \geq F_j^{L,m}(\mathbf{X}) \geq \cdots \geq F_j^{L,1}(\mathbf{X})$*. We let* $F_j^{L}(\mathbf{X})$ *denote the final lower bound* $F_j^{L,1}(\mathbf{X})$*, and we have*

$$F_j^L(\mathbf{X}) = \tilde{\mathbf{W}}^{a(1)}_{L,j,:}\mathbf{a}^{(0)} + \mathbf{\Omega}^{fc(1)}_{\Delta,j,:}\mathbf{c}^{(0)} + \sum_{k=1}^{m} \tilde{\mathbf{W}}^{x(k)}_{L,j,:}\mathbf{x}^{(k)} + \sum_{k=1}^{m} \tilde{\mathbf{b}}^{(k)}_{L,j} + \mathbf{b}^F_j,$$

*where*

$$\begin{aligned}
\tilde{\mathbf{W}}^{x(k)}_{L,j,q_k} &= \mathbf{\Omega}^{oc(k)}_{\omega,j,:}\mathbf{W}^{ox}_{:,q_k} + \mathbf{\Omega}^{fc(k)}_{\omega,j,:}\mathbf{W}^{fx}_{:,q_k} + \mathbf{\Omega}^{ig(k)}_{\omega,j,:}\mathbf{W}^{ix}_{:,q_k} + \mathbf{\Omega}^{ig(k)}_{\Theta,j,:}\mathbf{W}^{gx}_{:,q_k},\\
\tilde{\mathbf{W}}^{a(k)}_{L,j,r} &= \mathbf{\Omega}^{oc(k)}_{\omega,j,:}\mathbf{W}^{oa}_{:,r} + \mathbf{\Omega}^{fc(k)}_{\omega,j,:}\mathbf{W}^{fa}_{:,r} + \mathbf{\Omega}^{ig(k)}_{\omega,j,:}\mathbf{W}^{ia}_{:,r} + \mathbf{\Omega}^{ig(k)}_{\Theta,j,:}\mathbf{W}^{ga}_{:,r},\\
\tilde{\mathbf{b}}^{(k)}_{L,j} &= \mathbf{\Omega}^{oc(k)}_{\omega,j,:}\mathbf{b}^{o} + \mathbf{\Omega}^{fc(k)}_{\omega,j,:}\mathbf{b}^{f} + \mathbf{\Omega}^{ig(k)}_{\omega,j,:}\mathbf{b}^{i} + \mathbf{\Omega}^{ig(k)}_{\Theta,j,:}\mathbf{b}^{g} + \sum_{i=1}^{s}(\mathbf{\Omega}^{oc(k)}_{\psi,j,i} + \mathbf{\Omega}^{fc(k)}_{\psi,j,i} + \mathbf{\Omega}^{ig(k)}_{\psi,j,i}),
\end{aligned}$$

*and ($\odot$ is the Hadamard product)*

$$\mathbf{\Omega}^{oc(k)}_{\omega,j,:} = \begin{cases} \mathbf{W}^{Fa}_{j,:} \odot \omega^{oc(k)}_{j,:} & \text{if} \quad k = m; \\ \tilde{\mathbf{W}}^{a(k+1)}_{L,j,:} \odot \omega^{oc(k)}_{j,:} & \text{if} \quad k \in [m-1]; \end{cases}$$
$$\mathbf{\Omega}^{oc(k)}_{\Theta,j,:} = \begin{cases} \mathbf{W}^{Fa}_{j,:} \odot \mathbf{\Theta}^{oc(k)}_{j,:} & \text{if} \quad k = m; \\ \tilde{\mathbf{W}}^{a(k+1)}_{L,j,:} \odot \mathbf{\Theta}^{oc(k)}_{j,:} + \mathbf{\Omega}^{fc(k+1)}_{\Theta,j,:} & \text{if} \quad k \in [m-1]; \end{cases}$$
$$\mathbf{\Omega}^{oc(k)}_{\psi,j,:} = \begin{cases} \mathbf{W}^{Fa}_{j,:} \odot \psi^{oc(k)}_{j,:} & \text{if} \quad k = m; \\ \tilde{\mathbf{W}}^{a(k+1)}_{L,j,:} \odot \psi^{oc(k)}_{j,:} & \text{if} \quad k \in [m-1]; \end{cases}$$

$$\mathbf{\Omega}^{fc(k)}_{\omega,j,:} = \mathbf{\Omega}^{oc(k)}_{\Theta,j,:} \odot \omega^{fc(k)}_{j,:} \quad \text{if} \quad k \in [m]; \qquad \mathbf{\Omega}^{ig(k)}_{\omega,j,:} = \mathbf{\Omega}^{oc(k)}_{\Theta,j,:} \odot \omega^{ig(k)}_{j,:} \quad \text{if} \quad k \in [m];$$
$$\mathbf{\Omega}^{fc(k)}_{\Theta,j,:} = \mathbf{\Omega}^{oc(k)}_{\Theta,j,:} \odot \mathbf{\Theta}^{fc(k)}_{j,:} \quad \text{if} \quad k \in [m]; \qquad \mathbf{\Omega}^{ig(k)}_{\Theta,j,:} = \mathbf{\Omega}^{oc(k)}_{\Theta,j,:} \odot \mathbf{\Theta}^{ig(k)}_{j,:} \quad \text{if} \quad k \in [m];$$
$$\mathbf{\Omega}^{fc(k)}_{\psi,j,:} = \mathbf{\Omega}^{oc(k)}_{\Theta,j,:} \odot \psi^{fc(k)}_{j,:} \quad \text{if} \quad k \in [m]; \qquad \mathbf{\Omega}^{ig(k)}_{\psi,j,:} = \mathbf{\Omega}^{oc(k)}_{\Theta,j,:} \odot \psi^{ig(k)}_{j,:} \quad \text{if} \quad k \in [m];$$

*and* $\forall r \in s$,

$$\omega^{oc(m)}_{j,r} = \begin{cases} \alpha^{oc(m)}_{L,r} & \text{if} \;\; \mathbf{W}^{Fa}_{j,r} \geq 0; \\ \alpha^{oc(m)}_{U,r} & \text{if} \;\; \mathbf{W}^{Fa}_{j,r} < 0; \end{cases} \quad \mathbf{\Theta}^{oc(m)}_{j,r} = \begin{cases} \beta^{oc(m)}_{L,r} & \text{if} \;\; \mathbf{W}^{Fa}_{j,r} \geq 0; \\ \beta^{oc(m)}_{U,r} & \text{if} \;\; \mathbf{W}^{Fa}_{j,r} < 0; \end{cases} \quad \psi^{oc(m)}_{j,r} = \begin{cases} \gamma^{oc(m)}_{L,r} & \text{if} \;\; \mathbf{W}^{Fa}_{j,r} \geq 0; \\ \gamma^{oc(m)}_{U,r} & \text{if} \;\; \mathbf{W}^{Fa}_{j,r} < 0; \end{cases}$$

*and* $\forall r \in s, k \in [m-1]$,

$$\omega^{oc(k)}_{j,r} = \begin{cases} \alpha^{oc(k)}_{L,r} & \text{if} \;\; \tilde{\mathbf{W}}^{a(k+1)}_{L,j,r} \geq 0; \\ \alpha^{oc(k)}_{U,r} & \text{if} \;\; \tilde{\mathbf{W}}^{a(k+1)}_{L,j,r} < 0; \end{cases}$$
$$\mathbf{\Theta}^{oc(k)}_{j,r} = \begin{cases} \beta^{oc(k)}_{L,r} & \text{if} \;\; \tilde{\mathbf{W}}^{a(k+1)}_{L,j,r} \geq 0; \\ \beta^{oc(k)}_{U,r} & \text{if} \;\; \tilde{\mathbf{W}}^{a(k+1)}_{L,j,r} < 0; \end{cases}$$
$$\psi^{oc(k)}_{j,r} = \begin{cases} \gamma^{oc(k)}_{L,r} & \text{if} \;\; \tilde{\mathbf{W}}^{a(k+1)}_{L,j,r} \geq 0; \\ \gamma^{oc(k)}_{U,r} & \text{if} \;\; \tilde{\mathbf{W}}^{a(k+1)}_{L,j,r} < 0; \end{cases}$$

*and* $\forall r \in s, k \in [m]$,

$$\omega^{fc(k)}_{j,r} = \begin{cases} \alpha^{fc(k)}_{L,r} & \text{if} \;\; \mathbf{\Omega}^{oc(k)}_{\Theta,j,r} \geq 0; \\ \alpha^{fc(k)}_{U,r} & \text{if} \;\; \mathbf{\Omega}^{oc(k)}_{\Theta,j,r} < 0; \end{cases} \quad \omega^{ig(k)}_{j,r} = \begin{cases} \alpha^{ig(k)}_{L,r} & \text{if} \;\; \mathbf{\Omega}^{oc(k)}_{\Theta,j,r} \geq 0; \\ \alpha^{ig(k)}_{U,r} & \text{if} \;\; \mathbf{\Omega}^{oc(k)}_{\Theta,j,r} < 0; \end{cases}$$
$$\mathbf{\Theta}^{fc(k)}_{j,r} = \begin{cases} \beta^{fc(k)}_{L,r} & \text{if} \;\; \mathbf{\Omega}^{oc(k)}_{\Theta,j,r} \geq 0; \\ \beta^{fc(k)}_{U,r} & \text{if} \;\; \mathbf{\Omega}^{oc(k)}_{\Theta,j,r} < 0; \end{cases} \quad \mathbf{\Theta}^{ig(k)}_{j,r} = \begin{cases} \beta^{ig(k)}_{L,r} & \text{if} \;\; \mathbf{\Omega}^{oc(k)}_{\Theta,j,r} \geq 0; \\ \beta^{ig(k)}_{U,r} & \text{if} \;\; \mathbf{\Omega}^{oc(k)}_{\Theta,j,r} < 0; \end{cases}$$
$$\psi^{fc(k)}_{j,r} = \begin{cases} \gamma^{fc(k)}_{L,r} & \text{if} \;\; \mathbf{\Omega}^{oc(k)}_{\Theta,j,r} \geq 0; \\ \gamma^{fc(k)}_{U,r} & \text{if} \;\; \mathbf{\Omega}^{oc(k)}_{\Theta,j,r} < 0; \end{cases} \quad \psi^{ig(k)}_{j,r} = \begin{cases} \gamma^{ig(k)}_{L,r} & \text{if} \;\; \mathbf{\Omega}^{oc(k)}_{\Theta,j,r} \geq 0; \\ \gamma^{ig(k)}_{U,r} & \text{if} \;\; \mathbf{\Omega}^{oc(k)}_{\Theta,j,r} < 0. \end{cases}$$

**Corollary A. 2 (Closed-form global bounds)** *Given data* $\mathbf{X} \in \mathbb{R}^{n \times m}$, *$l_p$ ball parameters $p \geq 1$ and $\epsilon \geq 0$. For an $m$-layer long short-term memory network $F : \mathbb{R}^{n \times m} \to \mathbb{R}^t$, there exists two fixed values $\gamma^L_j$ and $\gamma^U_j$ such that $\forall\, \mathbf{X} \in \mathbb{R}^{n \times m}$ where $\mathbf{x}^{(k)} \in \mathbb{B}_p(\mathbf{x}^{(k)}_0, \epsilon)$, and $\forall\, j \in [t]$, $1/q = 1 - 1/p$, the inequity $\gamma^L_j \leq F_j(\mathbf{X}) \leq \gamma^U_j$ holds true, where*

$$\gamma^U_j = \tilde{\mathbf{W}}^{a(1)}_{U,j,:}\mathbf{a}^{(0)} + \mathbf{\Lambda}^{fc(1)}_{\Delta,j,:}\mathbf{c}^{(0)} + \sum_{k=1}^{m} \epsilon \|\tilde{\mathbf{W}}^{x(k)}_{U,j,:}\|_q + \sum_{k=1}^{m} \tilde{\mathbf{W}}^{x(k)}_{U,j,:}\mathbf{x}^{(k)}_0 + \sum_{k=1}^{m} \tilde{\mathbf{b}}^{(k)}_{U,j} + \mathbf{b}^F_j\,,$$
$$\gamma^L_j = \tilde{\mathbf{W}}^{a(1)}_{L,j,:}\mathbf{a}^{(0)} + \mathbf{\Omega}^{fc(1)}_{\Theta,j,:}\mathbf{c}^{(0)} - \sum_{k=1}^{m} \epsilon \|\tilde{\mathbf{W}}^{x(k)}_{L,j,:}\|_q + \sum_{k=1}^{m} \tilde{\mathbf{W}}^{x(k)}_{L,j,:}\mathbf{x}^{(k)}_0 + \sum_{k=1}^{m} \tilde{\mathbf{b}}^{(k)}_{L,j} + \mathbf{b}^F_j\,.$$

**Corollary A. 3 (Pre-activation bounds in LSTMs)** *The pre-activation bounds of different gates can be obtained via simple modifications from Theorem A.3. Specifically, we recall the definitions of pre-activations in different gates:*

$$\begin{aligned}
\textit{Input gate:} \quad & \mathbf{y}^{i(k)} = \underline{\mathbf{W}^{ix}\mathbf{x}^{(k)}} + \mathbf{W}^{ia}\mathbf{a}^{(k-1)} + \mathbf{b}^{i}; \\
\textit{Forget gate:} \quad & \mathbf{y}^{f(k)} = \underline{\mathbf{W}^{fx}\mathbf{x}^{(k)}} + \mathbf{W}^{fa}\mathbf{a}^{(k-1)} + \mathbf{b}^{f}; \\
\textit{Cell gate:} \quad & \mathbf{y}^{g(k)} = \underline{\mathbf{W}^{gx}\mathbf{x}^{(k)}} + \mathbf{W}^{ga}\mathbf{a}^{(k-1)} + \mathbf{b}^{g}; \\
\textit{Output gate:} \quad & \mathbf{y}^{o(k)} = \underline{\mathbf{W}^{ox}\mathbf{x}^{(k)}} + \mathbf{W}^{oa}\mathbf{a}^{(k-1)} + \mathbf{b}^{o}.
\end{aligned}$$

*For a given LSTM and input $\mathbf{X}_0$, the underlined part of the equations are bounded by*

$$\mathbf{W}^{gate}\mathbf{x}_0^{(k)} - \epsilon\|\mathbf{W}^{gate}\|_q \le \mathbf{W}^{gate}\mathbf{x}^{(k)} \le \mathbf{W}^{gate}\mathbf{x}_0^{(k)} + \epsilon\|\mathbf{W}^{gate}\|_q,$$

*where gate = $\{ix, fx, gx, ox\}$. Thus to derive pre-activation bounds, we only need to know the ranges of remaining parts in the equations above. These can be computed by replacing the output mapping $\mathbf{W}^{Fa}$ in Theorem A.3 by $\mathbf{W}^{ia}, \mathbf{W}^{fa}, \mathbf{W}^{ga}, \mathbf{W}^{oa}$, respectively. The output bias $\mathbf{b}^F$ is correspondingly substituted with $\mathbf{b}^i, \mathbf{b}^f, \mathbf{b}^g, \mathbf{b}^o$. For example, to derive the bounds for pre-activation bounds of input gates, we replace the output mapping matrix and bias from $\mathbf{W}^{Fa}$ and $\mathbf{b}^F$ by $\mathbf{W}^{ia}$and $\mathbf{b}^i$.*

**Theorem A. 4 (Closed-form cell state bounds of long short-term memory network F)** *For the cell state $\mathbf{c}_j^{(v)}$ of the $v$-th layer in a given $m$-layer ($v \le m$) long short-term memory network, there exists two explicit functions $g_j^{L,v} : \mathbb{R}^{n\times v} \to \mathbb{R}^s$ and $g_j^{U,v} : \mathbb{R}^{n\times v} \to \mathbb{R}^s$ and two fixed values $\mathbf{l}_j^{c(v)}$ and $\mathbf{u}_j^{c(v)}$ such that $\forall\ j \in [s]$ and $\forall\ \mathbf{X}^{(1:v)} \in \mathbb{R}^{n\times v}$ where $\mathbf{x}^{(k)} \in \mathbb{B}_p(\mathbf{x}_0^{(k)}, \epsilon)$ and $1/q = 1 - 1/p$, the inequity $\mathbf{l}_j^{c(v)} \le g_j^{L,v}(\mathbf{X}^{(1:v)}) \le \mathbf{y}_j^{(v)} \le g_j^{U,v}(\mathbf{X}^{(1:v)}) \le \mathbf{u}_j^{c(v)}$ holds true, where*

$$\mathbf{u}_j^{c(v)} = \tilde{\mathbf{W}}^{a(1)}_{U,j,:}\mathbf{a}^{(0)} + \mathbf{\Lambda}^{fc(1)}_{\Delta,j,:}\mathbf{c}^{(0)} + \sum_{k=1}^{v}\epsilon\|\tilde{\mathbf{W}}^{x(k)}_{U,j,:}\|_q + \sum_{k=1}^{v}\tilde{\mathbf{W}}^{x(k)}_{U,j,:}\mathbf{x}_0^{(k)} + \sum_{k=1}^{v}\tilde{\mathbf{b}}^{(k)}_{U,j},$$

$$\mathbf{l}_j^{c(v)} = \tilde{\mathbf{W}}^{a(1)}_{L,j,:}\mathbf{a}^{(0)} + \mathbf{\Omega}^{fc(1)}_{\Theta,j,:}\mathbf{c}^{(0)} - \sum_{k=1}^{v}\epsilon\|\tilde{\mathbf{W}}^{x(k)}_{L,j,:}\|_q + \sum_{k=1}^{v}\tilde{\mathbf{W}}^{x(k)}_{L,j,:}\mathbf{x}_0^{(k)} + \sum_{k=1}^{v}\tilde{\mathbf{b}}^{(k)}_{L,j},$$

*where*

$$\begin{aligned}
\tilde{\mathbf{W}}^{x(v)}_{U,j,q_v} &= \mathbf{\Lambda}^{fc(v)}_{\lambda,j,:}\mathbf{W}^{fx}_{:,q_v} + \mathbf{\Lambda}^{ig(v)}_{\lambda,j,:}\mathbf{W}^{ix}_{:,q_v} + \mathbf{\Lambda}^{ig(v)}_{\Delta,j,:}\mathbf{W}^{gx}_{:,q_v}, \\
\tilde{\mathbf{W}}^{a(v)}_{U,j,r} &= \mathbf{\Lambda}^{fc(v)}_{\lambda,j,:}\mathbf{W}^{fa}_{:,r} + \mathbf{\Lambda}^{ig(v)}_{\lambda,j,:}\mathbf{W}^{ia}_{:,r} + \mathbf{\Lambda}^{ig(v)}_{\Delta,j,:}\mathbf{W}^{ga}_{:,r}, \\
\tilde{\mathbf{b}}^{(v)}_{U,j} &= \mathbf{\Lambda}^{fc(v)}_{\lambda,j,:}\mathbf{b}^{f} + \mathbf{\Lambda}^{ig(v)}_{\lambda,j,:}\mathbf{b}^{i} + \mathbf{\Lambda}^{ig(v)}_{\Delta,j,:}\mathbf{b}^{g} + \sum_{i=1}^{s}(\mathbf{\Lambda}^{fc(v)}_{\varphi,j,i} + \mathbf{\Lambda}^{ig(v)}_{\varphi,j,i}), \\
\tilde{\mathbf{W}}^{x(v)}_{L,j,q_v} &= \mathbf{\Omega}^{fc(v)}_{\omega,j,:}\mathbf{W}^{fx}_{:,q_v} + \mathbf{\Omega}^{ig(v)}_{\omega,j,:}\mathbf{W}^{ix}_{:,q_v} + \mathbf{\Omega}^{ig(v)}_{\Theta,j,:}\mathbf{W}^{gx}_{:,q_v}, \\
\tilde{\mathbf{W}}^{a(v)}_{L,j,r} &= \mathbf{\Omega}^{fc(v)}_{\omega,j,:}\mathbf{W}^{fa}_{:,r} + \mathbf{\Omega}^{ig(v)}_{\omega,j,:}\mathbf{W}^{ia}_{:,r} + \mathbf{\Omega}^{ig(v)}_{\Theta,j,:}\mathbf{W}^{ga}_{:,r}, \\
\tilde{\mathbf{b}}^{(v)}_{L,j} &= \mathbf{\Omega}^{fc(v)}_{\omega,j,:}\mathbf{b}^{f} + \mathbf{\Omega}^{ig(v)}_{\omega,j,:}\mathbf{b}^{i} + \mathbf{\Omega}^{ig(v)}_{\Theta,j,:}\mathbf{b}^{g} + \sum_{i=1}^{s}(\mathbf{\Omega}^{fc(v)}_{\psi,j,i} + \mathbf{\Omega}^{ig(v)}_{\psi,j,i}),
\end{aligned}$$

*and* $\forall k \in [v-1]$

$$\begin{aligned}
\tilde{\mathbf{W}}^{x(k)}_{U,j,q_k} &= \mathbf{\Lambda}^{oc(k)}_{\lambda,j,:}\mathbf{W}^{ox}_{:,q_k} + \mathbf{\Lambda}^{fc(k)}_{\lambda,j,:}\mathbf{W}^{fx}_{:,q_k} + \mathbf{\Lambda}^{ig(k)}_{\lambda,j,:}\mathbf{W}^{ix}_{:,q_k} + \mathbf{\Lambda}^{ig(k)}_{\Delta,j,:}\mathbf{W}^{gx}_{:,q_k}, \\
\tilde{\mathbf{W}}^{a(k)}_{U,j,r} &= \mathbf{\Lambda}^{oc(k)}_{\lambda,j,:}\mathbf{W}^{oa}_{:,r} + \mathbf{\Lambda}^{fc(k)}_{\lambda,j,:}\mathbf{W}^{fa}_{:,r} + \mathbf{\Lambda}^{ig(k)}_{\lambda,j,:}\mathbf{W}^{ia}_{:,r} + \mathbf{\Lambda}^{ig(k)}_{\Delta,j,:}\mathbf{W}^{ga}_{:,r}, \\
\tilde{\mathbf{b}}^{(k)}_{U,j} &= \mathbf{\Lambda}^{oc(k)}_{\lambda,j,:}\mathbf{b}^{o} + \mathbf{\Lambda}^{fc(k)}_{\lambda,j,:}\mathbf{b}^{f} + \mathbf{\Lambda}^{ig(k)}_{\lambda,j,:}\mathbf{b}^{i} + \mathbf{\Lambda}^{ig(k)}_{\Delta,j,:}\mathbf{b}^{g} + \sum_{i=1}^{s}(\mathbf{\Lambda}^{oc(k)}_{\varphi,j,i} + \mathbf{\Lambda}^{fc(k)}_{\varphi,j,i} + \mathbf{\Lambda}^{ig(k)}_{\varphi,j,i}), \\
\tilde{\mathbf{W}}^{x(k)}_{L,j,q_k} &= \mathbf{\Omega}^{oc(k)}_{\omega,j,:}\mathbf{W}^{ox}_{:,q_k} + \mathbf{\Omega}^{fc(k)}_{\omega,j,:}\mathbf{W}^{fx}_{:,q_k} + \mathbf{\Omega}^{ig(k)}_{\omega,j,:}\mathbf{W}^{ix}_{:,q_k} + \mathbf{\Omega}^{ig(k)}_{\Theta,j,:}\mathbf{W}^{gx}_{:,q_k},
\end{aligned}$$

$$\tilde{\mathbf{W}}^{a(k)}_{L,j,r} = \boldsymbol{\Omega}^{oc(k)}_{\omega,j,:}\mathbf{W}^{oa}_{:,r} + \boldsymbol{\Omega}^{fc(k)}_{\omega,j,:}\mathbf{W}^{fa}_{:,r} + \boldsymbol{\Omega}^{ig(k)}_{\omega,j,:}\mathbf{W}^{ia}_{:,r} + \boldsymbol{\Omega}^{ig(k)}_{\Theta,j,:}\mathbf{W}^{ga}_{:,r},$$

$$\tilde{\mathbf{b}}^{(k)}_{L,j} = \boldsymbol{\Omega}^{oc(k)}_{\omega,j,:}\mathbf{b}^{o} + \boldsymbol{\Omega}^{fc(k)}_{\omega,j,:}\mathbf{b}^{f} + \boldsymbol{\Omega}^{ig(k)}_{\omega,j,:}\mathbf{b}^{i} + \boldsymbol{\Omega}^{ig(k)}_{\Theta,j,:}\mathbf{b}^{g} + \sum_{i=1}^{s}(\boldsymbol{\Omega}^{oc(k)}_{\psi,j,i} + \boldsymbol{\Omega}^{fc(k)}_{\psi,j,i} + \boldsymbol{\Omega}^{ig(k)}_{\psi,j,i}),$$

*and*

$$\boldsymbol{\Lambda}^{oc(k)}_{\lambda,:,:} = \tilde{\mathbf{W}}^{a(k+1)}_{U,:,:} \odot \lambda^{oc(k)}_{:,:} \quad \textit{if} \;\; k \in [v-1]; \qquad \boldsymbol{\Omega}^{oc(k)}_{\omega,:,:} = \tilde{\mathbf{W}}^{a(k+1)}_{L,:,:} \odot \omega^{oc(k)}_{:,:} \quad \textit{if} \;\; k \in [v-1];$$

$$\boldsymbol{\Lambda}^{oc(k)}_{\Delta,:,:} = \tilde{\mathbf{W}}^{a(k+1)}_{U,:,:} \odot \boldsymbol{\Delta}^{oc(k)}_{:,:} + \boldsymbol{\Lambda}^{fc(k+1)}_{\Delta,:,:} \quad \textit{if} \;\; k \in [v-1]; \qquad \boldsymbol{\Omega}^{oc(k)}_{\Theta,:,:} = \tilde{\mathbf{W}}^{a(k+1)}_{L,:,:} \odot \boldsymbol{\Theta}^{oc(k)}_{:,:} + \boldsymbol{\Omega}^{fc(k+1)}_{\Theta,:,:} \quad \textit{if} \;\; k \in [v-1];$$

$$\boldsymbol{\Lambda}^{oc(k)}_{\varphi,:,:} = \tilde{\mathbf{W}}^{a(k+1)}_{U,:,:} \odot \varphi^{oc(k)}_{:,:} \quad \textit{if} \;\; k \in [v-1]; \qquad \boldsymbol{\Omega}^{oc(k)}_{\psi,:,:} = \tilde{\mathbf{W}}^{a(k+1)}_{L,:,:} \odot \psi^{oc(k)}_{:,:} \quad \textit{if} \;\; k \in [v-1];$$

$$\boldsymbol{\Lambda}^{fc(k)}_{\lambda,:,:} = \begin{cases} diag(\alpha^{fc(k)}_{U,:}) & \textit{if} \;\; k = v; \\ \boldsymbol{\Lambda}^{oc(k)}_{\Delta,:,:} \odot \lambda^{fc(k)}_{:,:} & \textit{if} \;\; k \in [v-1]; \end{cases} \qquad \boldsymbol{\Omega}^{fc(k)}_{\omega,:,:} = \begin{cases} diag(\alpha^{fc(k)}_{L,:}) & \textit{if} \;\; k = v; \\ \boldsymbol{\Omega}^{oc(k)}_{\Theta,:,:} \odot \omega^{fc(k)}_{:,:} & \textit{if} \;\; k \in [v-1]; \end{cases}$$

$$\boldsymbol{\Lambda}^{fc(k)}_{\Delta,:,:} = \begin{cases} diag(\beta^{fc(k)}_{U,:}) & \textit{if} \;\; k = v; \\ \boldsymbol{\Lambda}^{oc(k)}_{\Delta,:,:} \odot \boldsymbol{\Delta}^{fc(k)}_{:,:} & \textit{if} \;\; k \in [v-1]; \end{cases} \qquad \boldsymbol{\Omega}^{fc(k)}_{\Theta,:,:} = \begin{cases} diag(\beta^{fc(k)}_{L,:}) & \textit{if} \;\; k = v; \\ \boldsymbol{\Omega}^{oc(k)}_{\Theta,:,:} \odot \boldsymbol{\Theta}^{fc(k)}_{:,:} & \textit{if} \;\; k \in [v-1]; \end{cases}$$

$$\boldsymbol{\Lambda}^{fc(k)}_{\varphi,:,:} = \begin{cases} diag(\gamma^{fc(k)}_{U,:}) & \textit{if} \;\; k = v; \\ \boldsymbol{\Lambda}^{oc(k)}_{\Delta,:,:} \odot \varphi^{fc(k)}_{:,:} & \textit{if} \;\; k \in [v-1]; \end{cases} \qquad \boldsymbol{\Omega}^{fc(k)}_{\psi,:,:} = \begin{cases} diag(\gamma^{fc(k)}_{L,:}) & \textit{if} \;\; k = v; \\ \boldsymbol{\Omega}^{oc(k)}_{\Theta,:,:} \odot \psi^{fc(k)}_{:,:} & \textit{if} \;\; k \in [v-1]; \end{cases}$$

$$\boldsymbol{\Lambda}^{ig(k)}_{\lambda,:,:} = \begin{cases} diag(\alpha^{ig(k)}_{U,:}) & \textit{if} \;\; k = v; \\ \boldsymbol{\Lambda}^{oc(k)}_{\Delta,:,:} \odot \lambda^{ig(k)}_{:,:} & \textit{if} \;\; k \in [v-1]; \end{cases} \qquad \boldsymbol{\Omega}^{ig(k)}_{\omega,:,:} = \begin{cases} diag(\alpha^{ig(k)}_{L,:}) & \textit{if} \;\; k = v; \\ \boldsymbol{\Omega}^{oc(k)}_{\Theta,:,:} \odot \omega^{ig(k)}_{:,:} & \textit{if} \;\; k \in [v-1]; \end{cases}$$

$$\boldsymbol{\Lambda}^{ig(k)}_{\Delta,:,:} = \begin{cases} diag(\beta^{ig(k)}_{U,:}) & \textit{if} \;\; k = v; \\ \boldsymbol{\Lambda}^{oc(k)}_{\Delta,:,:} \odot \boldsymbol{\Delta}^{ig(k)}_{:,:} & \textit{if} \;\; k \in [v-1]; \end{cases} \qquad \boldsymbol{\Omega}^{ig(k)}_{\Theta,:,:} = \begin{cases} diag(\beta^{ig(k)}_{L,:}) & \textit{if} \;\; k = v; \\ \boldsymbol{\Omega}^{oc(k)}_{\Theta,:,:} \odot \boldsymbol{\Theta}^{ig(k)}_{:,:} & \textit{if} \;\; k \in [v-1]; \end{cases}$$

$$\boldsymbol{\Lambda}^{ig(k)}_{\varphi,:,:} = \begin{cases} diag(\gamma^{ig(k)}_{U,:}) & \textit{if} \;\; k = v; \\ \boldsymbol{\Lambda}^{oc(k)}_{\Delta,:,:} \odot \varphi^{ig(k)}_{:,:} & \textit{if} \;\; k \in [v-1]; \end{cases} \qquad \boldsymbol{\Omega}^{ig(k)}_{\psi,:,:} = \begin{cases} diag(\gamma^{ig(k)}_{L,:}) & \textit{if} \;\; k = v; \\ \boldsymbol{\Omega}^{oc(k)}_{\Theta,:,:} \odot \psi^{ig(k)}_{:,:} & \textit{if} \;\; k \in [v-1]; \end{cases}$$

*and* $\forall r \in s, k \in [v-1]$,

$$\lambda^{oc(k)}_{j,r} = \begin{cases} \alpha^{oc(k)}_{U,r} & \textit{if} \;\; \tilde{\mathbf{W}}^{a(k+1)}_{U,j,r} \geq 0; \\ \alpha^{oc(k)}_{L,r} & \textit{if} \;\; \tilde{\mathbf{W}}^{a(k+1)}_{U,j,r} < 0; \end{cases} \qquad \omega^{oc(k)}_{j,r} = \begin{cases} \alpha^{oc(k)}_{L,r} & \textit{if} \;\; \tilde{\mathbf{W}}^{a(k+1)}_{L,j,r} \geq 0; \\ \alpha^{oc(k)}_{U,r} & \textit{if} \;\; \tilde{\mathbf{W}}^{a(k+1)}_{L,j,r} < 0; \end{cases}$$

$$\boldsymbol{\Delta}^{oc(k)}_{j,r} = \begin{cases} \beta^{oc(k)}_{U,r} & \textit{if} \;\; \tilde{\mathbf{W}}^{a(k+1)}_{U,j,r} \geq 0; \\ \beta^{oc(k)}_{L,r} & \textit{if} \;\; \tilde{\mathbf{W}}^{a(k+1)}_{U,j,r} < 0; \end{cases} \qquad \boldsymbol{\Theta}^{oc(k)}_{j,r} = \begin{cases} \beta^{oc(k)}_{L,r} & \textit{if} \;\; \tilde{\mathbf{W}}^{a(k+1)}_{L,j,r} \geq 0; \\ \beta^{oc(k)}_{U,r} & \textit{if} \;\; \tilde{\mathbf{W}}^{a(k+1)}_{L,j,r} < 0; \end{cases}$$

$$\varphi^{oc(k)}_{j,r} = \begin{cases} \gamma^{oc(k)}_{U,r} & \textit{if} \;\; \tilde{\mathbf{W}}^{a(k+1)}_{U,j,r} \geq 0; \\ \gamma^{oc(k)}_{L,r} & \textit{if} \;\; \tilde{\mathbf{W}}^{a(k+1)}_{U,j,r} < 0; \end{cases} \qquad \psi^{oc(k)}_{j,r} = \begin{cases} \gamma^{oc(k)}_{L,r} & \textit{if} \;\; \tilde{\mathbf{W}}^{a(k+1)}_{L,j,r} \geq 0; \\ \gamma^{oc(k)}_{U,r} & \textit{if} \;\; \tilde{\mathbf{W}}^{a(k+1)}_{L,j,r} < 0; \end{cases}$$

$$\lambda^{fc(k)}_{j,r} = \begin{cases} \alpha^{fc(k)}_{U,r} & \textit{if} \;\; \boldsymbol{\Lambda}^{oc(k)}_{\Delta,j,r} \geq 0; \\ \alpha^{fc(k)}_{L,r} & \textit{if} \;\; \boldsymbol{\Lambda}^{oc(k)}_{\Delta,j,r} < 0; \end{cases} \qquad \omega^{fc(k)}_{j,r} = \begin{cases} \alpha^{fc(k)}_{L,r} & \textit{if} \;\; \boldsymbol{\Omega}^{oc(k)}_{\Theta,j,r} \geq 0; \\ \alpha^{fc(k)}_{U,r} & \textit{if} \;\; \boldsymbol{\Omega}^{oc(k)}_{\Theta,j,r} < 0; \end{cases}$$

$$\boldsymbol{\Delta}^{fc(k)}_{j,r} = \begin{cases} \beta^{fc(k)}_{U,r} & \textit{if} \;\; \boldsymbol{\Lambda}^{oc(k)}_{\Delta,j,r} \geq 0; \\ \beta^{fc(k)}_{L,r} & \textit{if} \;\; \boldsymbol{\Lambda}^{oc(k)}_{\Delta,j,r} < 0; \end{cases} \qquad \boldsymbol{\Theta}^{fc(k)}_{j,r} = \begin{cases} \beta^{fc(k)}_{L,r} & \textit{if} \;\; \boldsymbol{\Omega}^{oc(k)}_{\Theta,j,r} \geq 0; \\ \beta^{fc(k)}_{U,r} & \textit{if} \;\; \boldsymbol{\Omega}^{oc(k)}_{\Theta,j,r} < 0; \end{cases}$$

$$\varphi^{fc(k)}_{j,r} = \begin{cases} \gamma^{fc(k)}_{U,r} & \textit{if} \;\; \boldsymbol{\Lambda}^{oc(k)}_{\Delta,j,r} \geq 0; \\ \gamma^{fc(k)}_{L,r} & \textit{if} \;\; \boldsymbol{\Lambda}^{oc(k)}_{\Delta,j,r} < 0; \end{cases} \qquad \psi^{fc(k)}_{j,r} = \begin{cases} \gamma^{fc(k)}_{L,r} & \textit{if} \;\; \boldsymbol{\Omega}^{oc(k)}_{\Theta,j,r} \geq 0; \\ \gamma^{fc(k)}_{U,r} & \textit{if} \;\; \boldsymbol{\Omega}^{oc(k)}_{\Theta,j,r} < 0; \end{cases}$$

$$\lambda^{ig(k)}_{j,r} = \begin{cases} \alpha^{ig(k)}_{U,r} & \textit{if} \;\; \boldsymbol{\Lambda}^{oc(k)}_{\Delta,j,r} \geq 0; \\ \alpha^{ig(k)}_{L,r} & \textit{if} \;\; \boldsymbol{\Lambda}^{oc(k)}_{\Delta,j,r} < 0; \end{cases} \qquad \omega^{ig(k)}_{j,r} = \begin{cases} \alpha^{ig(k)}_{L,r} & \textit{if} \;\; \boldsymbol{\Omega}^{oc(k)}_{\Theta,j,r} \geq 0; \\ \alpha^{ig(k)}_{U,r} & \textit{if} \;\; \boldsymbol{\Omega}^{oc(k)}_{\Theta,j,r} < 0; \end{cases}$$

$$\boldsymbol{\Delta}^{ig(k)}_{j,r} = \begin{cases} \beta^{ig(k)}_{U,r} & \textit{if} \;\; \boldsymbol{\Lambda}^{oc(k)}_{\Delta,j,r} \geq 0; \\ \beta^{ig(k)}_{L,r} & \textit{if} \;\; \boldsymbol{\Lambda}^{oc(k)}_{\Delta,j,r} < 0; \end{cases} \qquad \boldsymbol{\Theta}^{ig(k)}_{j,r} = \begin{cases} \beta^{ig(k)}_{L,r} & \textit{if} \;\; \boldsymbol{\Omega}^{oc(k)}_{\Theta,j,r} \geq 0; \\ \beta^{ig(k)}_{U,r} & \textit{if} \;\; \boldsymbol{\Omega}^{oc(k)}_{\Theta,j,r} < 0; \end{cases}$$

$$\varphi_{j,r}^{ig(k)} = \begin{cases} \gamma_{U,r}^{ig(k)} & \textit{if} \quad \mathbf{\Lambda}_{\Delta,j,r}^{oc(k)} \geq 0; \\ \gamma_{L,r}^{ig(k)} & \textit{if} \quad \mathbf{\Lambda}_{\Delta,j,r}^{oc(k)} < 0; \end{cases} \qquad \psi_{j,r}^{ig(k)} = \begin{cases} \gamma_{L,r}^{ig(k)} & \textit{if} \quad \mathbf{\Omega}_{\Theta,j,r}^{oc(k)} \geq 0; \\ \gamma_{U,r}^{ig(k)} & \textit{if} \quad \mathbf{\Omega}_{\Theta,j,r}^{oc(k)} < 0; \end{cases}$$

*where* $\odot$ *is the Hadamard product.*

### A.4 Bounding Planes for 2D Nonlinear Activation Functions

In this part, we elaborate on how bounding linear functions (planes) $h_{L,r}^{oc(k)}$, $h_{U,r}^{oc(k)}$, $h_{L,r}^{fc(k)}$, $h_{U,r}^{fc(k)}$, $h_{L,r}^{ig(k)}$, and $h_{U,r}^{ig(k)}$ mentioned in Definition 1 are computed. This problem corresponds to finding two bounding planes $h_{L,r}(\mathbf{v},\mathbf{z}) = \alpha_{L,r}\mathbf{v} + \beta_{L,r}\mathbf{z} + \gamma_{L,r}$ and $h_{U,r}(\mathbf{v},\mathbf{z}) = \alpha_{U,r}\mathbf{v} + \beta_{U,r}\mathbf{z} + \gamma_{U,r}$ for the two 2D nonlinear functions $\sigma(\mathbf{v})\mathbf{z}$ and $\sigma(\mathbf{v})\tanh(\mathbf{z})$ given the range of their inputs, namely, $\mathbf{v} \in [\mathbf{l}_r^v, \mathbf{u}_r^v]$ and $\mathbf{z} \in [\mathbf{l}_r^z, \mathbf{u}_r^z]$, $\forall r \in [s]$.

As we will exemplify the procedures for one single neuron, the subscript $r$ is omitted hereafter. We formulate the problem of finding 2D bounding planes as minimizing the volumes between upper-bounding/ lower-bounding planes and $\mathbf{v}$-$\mathbf{z}$ plane (See Figure 3 in the main text.) for the given $\mathbf{v}$, $\mathbf{z}$ intervals, under the constraints that the planes should be larger/ smaller than the nonlinear planes. Specifically, the two constrained optimization problems are formulated as

$$\begin{aligned} \underset{\alpha_L,\beta_L,\gamma_L}{\operatorname{argmax}} \quad & \iint_A (\alpha_L\mathbf{v} + \beta_L\mathbf{z} + \gamma_L)\, d\mathbf{v}\, d\mathbf{z} \\ \text{subject to} \quad & \alpha_L\mathbf{v} + \beta_L\mathbf{z} + \gamma_L \le f(\mathbf{v},\mathbf{z}),\ \forall(\mathbf{v},\mathbf{z}) \in A \end{aligned} \tag{25}$$

and

$$\begin{aligned} \underset{\alpha_U,\beta_U,\gamma_U}{\operatorname{argmin}} \quad & \iint_A (\alpha_U\mathbf{v} + \beta_U\mathbf{z} + \gamma_U)\, d\mathbf{v}\, d\mathbf{z} \\ \text{subject to} \quad & \alpha_U\mathbf{v} + \beta_U\mathbf{z} + \gamma_U \ge f(\mathbf{v},\mathbf{z}),\ \forall(\mathbf{v},\mathbf{z}) \in A \end{aligned} \tag{26}$$

where $f(\mathbf{v},\mathbf{z})$ is $\sigma(\mathbf{v})\mathbf{z}$ or $\sigma(\mathbf{v})\tanh(\mathbf{z})$, $A = \{(\mathbf{v},\mathbf{z}) \,|\, \mathbf{v} \in [\mathbf{l}^v, \mathbf{u}^v], \mathbf{z} \in [\mathbf{l}^z, \mathbf{u}^z]\}$.

To solve Problem (25), we first construct a differentiable indicator function $I(\alpha_L, \beta_L, \gamma_L)$ such that

$$I(\alpha_L,\beta_L,\gamma_L) \begin{cases} \le 0 & \text{if } h_L(\mathbf{v},\mathbf{z}) \le f(\mathbf{v},\mathbf{z}),\ \forall(\mathbf{v},\mathbf{z}) \in A; \\ > 0 & \text{otherwise.} \end{cases}$$

Then we define loss function as

$$loss(\alpha_L,\beta_L,\gamma_L) = \begin{cases} -\iint_A (\alpha_L\mathbf{v} + \beta_L\mathbf{z} + \gamma_L)\, d\mathbf{v}\, d\mathbf{z} & \text{if } I(\alpha_L,\beta_L,\gamma_L) \le 0; \\ -\theta * \iint_A (\alpha_L\mathbf{v} + \beta_L\mathbf{z} + \gamma_L)\, d\mathbf{v}\, d\mathbf{z} + I(\alpha_L,\beta_L,\gamma_L) & \text{otherwise,} \end{cases}$$

where $\theta$ is a small constant and we usually set it to 0.1. Then we can minimize the loss function using a standard gradient descent algorithm. We record the result of every gradient descend step and choose the $(\alpha_L, \beta_L, \gamma_L)$ with the maximum value of $\iint_A (\alpha_L\mathbf{v} + \beta_L\mathbf{z} + \gamma_L)\, d\mathbf{v}\, d\mathbf{z}$ and the indicator function value $I(\alpha_L, \beta_L, \gamma_L) \le 0$ as the lower bounding plane. The process of solving Problem (26) is similar.

The key step in the above process is to construct the indicator function $I(\alpha_L, \beta_L, \gamma_L)$ for the functions $f(\mathbf{v},\mathbf{z})$ and $h_L(\mathbf{v},\mathbf{z}) = \alpha_L\mathbf{v} + \beta_L\mathbf{z} + \gamma_L$ in the area $A$. Here we use $f(\mathbf{v},\mathbf{z}) = \sigma(\mathbf{v})\mathbf{z}$ (case $f(\mathbf{v},\mathbf{z}) = \sigma(\mathbf{v})\tanh(\mathbf{z})$ can be handled similarly) as an example to elaborate on how to construct the indicator function. First we observe that

$$h_L(\mathbf{v},\mathbf{z}) \le \sigma(\mathbf{v})\mathbf{z}, \forall(\mathbf{v},\mathbf{z}) \in A \Leftrightarrow \begin{cases} \alpha_L\mathbf{v} + \beta_L\mathbf{l}^z + \gamma_L \le \mathbf{l}^z\sigma(\mathbf{v}), & \forall \mathbf{v} \in [\mathbf{l}^v, \mathbf{u}^v] \\ \alpha_L\mathbf{v} + \beta_L\mathbf{u}^z + \gamma_L \le \mathbf{u}^z\sigma(\mathbf{v}), & \forall \mathbf{v} \in [\mathbf{l}^v, \mathbf{u}^v] \end{cases} \tag{27}$$

This greatly reduces the complexity to construct the indicator function $I(\alpha_L, \beta_L, \gamma_L)$ since the right hand side of Equation (27) are two inequalities of 1D functions. The indicator function $I$ now can be constructed as

$$I(\alpha_L,\beta_L,\gamma_L) = \max(I_1(\alpha_L,\beta_L,\gamma_L), 0) + \max(I_2(\alpha_L,\beta_L,\gamma_L), 0) \tag{28}$$

where

$$I_1(\alpha_L,\beta_L,\gamma_L) \begin{cases} \le 0 & \text{if } \alpha_L\mathbf{v} + \beta_L\mathbf{l}^z + \gamma_L \le \mathbf{l}^z\sigma(\mathbf{v}),\ \forall \mathbf{v} \in [\mathbf{l}^v, \mathbf{u}^v]; \\ > 0 & \text{otherwise;} \end{cases}$$

$$I_2(\alpha_L,\beta_L,\gamma_L) \begin{cases} \le 0 & \text{if } \alpha_L\mathbf{v} + \beta_L\mathbf{u}^z + \gamma_L \le \mathbf{u}^z\sigma(\mathbf{v}),\ \forall \mathbf{v} \in [\mathbf{l}^v, \mathbf{u}^v]; \\ > 0 & \text{otherwise.} \end{cases}$$

The construction of $I_1$ and $I_2$ corresponds to constructing an indicator function $I_3(\alpha, \beta)$ for two 1D functions $h(\mathbf{v}) = \alpha\mathbf{v} + \beta$ and $s\sigma(\mathbf{v})$ in the interval $[\mathbf{l}^v, \mathbf{u}^v]$, where

$$\begin{aligned}
\alpha &= \alpha_L \\
\beta &= \beta_L \mathbf{l}^z (\text{or } \mathbf{u}^z) + \gamma_L \\
s &= \mathbf{l}^z (\text{or } \mathbf{u}^z)
\end{aligned}$$

and

$$I_3(\alpha, \beta) \begin{cases} \leq 0 & \text{if } \alpha\mathbf{v} + \beta \leq s\sigma(\mathbf{v}),\ \forall \mathbf{v} \in [\mathbf{l}^v, \mathbf{u}^v]; \\ > 0 & \text{otherwise.} \end{cases}$$

The construction of $I_3$ can be easily achieved using the linearity of $h(\mathbf{v})$ and piecewise convexity of $s\sigma(\mathbf{v})$. Then we can use $I_3$ to construct $I_1$ and $I_2$. Finally $I(\alpha_L, \beta_L, \gamma_L)$ can be obtained according to Equation (28).

### A.5 Algorithms for Long Short-term Memory Networks

**Algorithm 2** *Compute POPQORN robustness bound of an $m$-layer LSTM (true label: c, target label: i)*

***Input****: an $m$-layer LSTM, input sequence $[\mathbf{x}^{(1)}, \dots, \mathbf{x}^{(m)}]$, p-norm, $\epsilon_0$.*

***Output****: a robustness bound $\tilde{\epsilon}$.*

*Replace the last layer weights $\overline{\mathbf{w}} \leftarrow \mathbf{W}^{Fa}_{c,:} - \mathbf{W}^{Fa}_{i,:}$*
*Initialize $\epsilon \leftarrow \epsilon_0$*
***while** $\epsilon$ has not achieved a desired accuracy and iteration limit has not reached **do***
    ***for** v=1,...,m **do***
        ***for** j=1,...,s **do***
            $\mathbf{l}^{i(v)}_j$, $\mathbf{l}^{f(v)}_j$, $\mathbf{l}^{g(v)}_j$, $\mathbf{l}^{o(v)}_j$, $\mathbf{u}^{i(v)}_j$, $\mathbf{u}^{f(v)}_j$, $\mathbf{u}^{g(v)}_j$, $\mathbf{u}^{o(v)}_j$ $\leftarrow$ *Corollary A.3*
            $h^{fc(v)}_{L,j}(\mathbf{y}^{f(v)}_j, \mathbf{c}^{(v-1)}_j)$, $h^{fc(v)}_{U,j}(\mathbf{y}^{f(v)}_j, \mathbf{c}^{(v-1)}_j)$ $\leftarrow$ *compute bounding planes for* $\sigma(\mathbf{y}^{f(v)}_j)\mathbf{c}^{(v-1)}_j$ *given* $\mathbf{l}^{f(v)}_j$, $\mathbf{u}^{f(v)}_j$, $\mathbf{l}^{c(v-1)}_j$, $\mathbf{u}^{c(v-1)}_j$
            $h^{ig(v)}_{L,j}(\mathbf{y}^{i(v)}_j, \mathbf{y}^{g(v)}_j)$, $h^{ig(v)}_{U,j}(\mathbf{y}^{i(v)}_j, \mathbf{y}^{g(v)}_j)$ $\leftarrow$ *compute bounding planes for* $\sigma(\mathbf{y}^{i(v)}_j)\tanh(\mathbf{y}^{g(v)}_j)$ *given* $\mathbf{l}^{i(v)}_j$, $\mathbf{u}^{i(v)}_j$, $\mathbf{l}^{g(v)}_j$, $\mathbf{u}^{g(v)}_j$
            $\mathbf{l}^{c(v)}_j$, $\mathbf{u}^{c(v)}_j$ $\leftarrow$ *Theorem A.4*
            $h^{oc(v)}_{L,j}(\mathbf{y}^{o(v)}_j, \mathbf{c}^{(v)}_j)$, $h^{oc(v)}_{U,j}(\mathbf{y}^{o(v)}_j, \mathbf{c}^{(v)}_j)$ $\leftarrow$ *compute bounding planes for* $\sigma(\mathbf{y}^{o(v)}_j)\tanh(\mathbf{c}^{(v)}_j)$ *given* $\mathbf{l}^{o(v)}_j$, $\mathbf{u}^{o(v)}_j$, $\mathbf{l}^{c(v)}_j$, $\mathbf{u}^{c(v)}_j$
        ***end for***
    ***end for***
    $\gamma^U, \gamma^L \leftarrow$ *Corollary A.2*
    ***if** $\gamma^L \geq 0$ **then***
        *$\epsilon$ is a lower bound; increase $\epsilon$ using a binary search procedure*
    ***else***
        *$\epsilon$ is not a lower bound; decrease $\epsilon$ using a binary search procedure*
    ***end if***
    $\tilde{\epsilon} \leftarrow \epsilon$
***end while***

As in the above, we provide a succinct algorithm summary to compute a robustness bound for an $m$-layer LSTM, below we also list a more detailed version of algorithms to compute lower and upper bounds for the final output $\mathbf{W}^{Fa}\mathbf{a}^{(m)} + \mathbf{b}^F$ of the LSTM and then provide a robustness bound for it. We first introduce an auxiliary algorithm that is needed in the computation.

**Algorithm 3** *Compute lower and upper bounds of the term* $\mathbf{W}\mathbf{a}^{(v)} + \mathbf{b}$

***Input****: layer index $v$ (range from 0 to $m$), weight matrix $\mathbf{W}$ and bias vector $\mathbf{b}$, bounding planes $[h^{oc(1)}_{L/U}, \dots, h^{oc(v)}_{L/U}]$, $[h^{fc(1)}_{L/U}, \dots, h^{fc(v)}_{L/U}]$ and $[h^{ig(1)}_{L/U}, \dots, h^{ig(v)}_{L/U}]$, an $m$-layer LSTM, LSTM input sequence $[\mathbf{x}^{(1)}, \dots, \mathbf{x}^{(v)}]$, p-norm, $\epsilon$.*

***Output****: lower bound $(\mathbf{W}\mathbf{a}^{(v)} + \mathbf{b})_{L,j}$ and upper bound $(\mathbf{W}\mathbf{a}^{(v)} + \mathbf{b})_{U,j}$, $j = 1, \dots, t$.(Here $t$ is the number of rows in $W$.)*

***Implementation****: As is shortly pointed out in Corollary A.3, this algorithm can be adapted from Theorem A.3 and Corollary A.2. Theorem A.3 is provided to compute the lower and upper bounds of the final output of an $m$-layer LSTM, which is $\mathbf{W}^{Fa}\mathbf{a}^{(m)} + \mathbf{b}^F$. Therefore, we only need to replace the output mapping $\mathbf{W}^{Fa}$ and $\mathbf{b}^F$ in Theorem A.3 by the input weight matrix $\mathbf{W}$ and bias vector $\mathbf{b}$, respectively, to evalute the bounds of $\mathbf{W}\mathbf{a}^{(m)} + \mathbf{b}$. Although Theorem A.3 is stated to compute bounds for the final layer ($m$-th layer) of the LSTM, it is also straightforward to generalize Theorem A.3 to compute bounds for an arbitrary layer $v$. Note that when $v = 0$, both the lower bound and upper bound of $\mathbf{W}\mathbf{a}^{(0)} + \mathbf{b}$ is just $\mathbf{W}\mathbf{a}^{(0)} + \mathbf{b}$ itself.*

It may seem like one can directly use Algorithm 3 to compute lower and upper bounds of the final output $\mathbf{W}^{Fa}\mathbf{a}^{(m)} + \mathbf{b}^F$ of an $m$-layer LSTM, but this is in fact not feasible as Algorithm 3 requires the bounding planes $h^{oc}_{L/U}$, $h^{fc}_{L/U}$, $h^{ig}_{L/U}$, which can only be computed after we know the lower and upper bounds of the gate pre-activations $\mathbf{y}^i$, $\mathbf{y}^f$, $\mathbf{y}^g$, $\mathbf{y}^o$ and lower and upper bounds of the cell state $\mathbf{c}$. Therefore, we need to introduce two more auxiliary algorithms below to compute bounds for $\mathbf{y}^i$, $\mathbf{y}^f$, $\mathbf{y}^g$, $\mathbf{y}^o$ and $\mathbf{c}$. Note that Algorithm 3 will be used in Algorithm 4. That is why we adapt Theorem A.3 and Corollary A.2 to construct this more general Algorithm 3.

**Algorithm 4** *Compute pre-activation bounds for the 4 gates* $\mathbf{y}^{i(v)}$, $\mathbf{y}^{f(v)}$, $\mathbf{y}^{g(v)}$ *and* $\mathbf{y}^{o(v)}$
***Input***: *layer index* $v$ *(range from* $1$ *to* $m$*), bounding planes* $[h^{oc(1)}_{L/U}, \ldots, h^{oc(v-1)}_{L/U}]$, $[h^{fc(1)}_{L/U}, \ldots, h^{fc(v-1)}_{L/U}]$ *and* $[h^{ig(1)}_{L/U}, \ldots, h^{ig(v-1)}_{L/U}]$, *an* $m$*-layer LSTM, LSTM input sequence* $[\mathbf{x}^{(1)}, \ldots, \mathbf{x}^{(v)}]$, *p-norm,* $\epsilon$.
***Output***: *lower bounds* $\mathbf{l}^{i(v)}_j$, $\mathbf{l}^{f(v)}_j$, $\mathbf{l}^{g(v)}_j$, $\mathbf{l}^{o(v)}_j$ *and upper bounds* $\mathbf{u}^{i(v)}_j$, $\mathbf{u}^{f(v)}_j$, $\mathbf{u}^{g(v)}_j$, $\mathbf{u}^{o(v)}_j$, $j = 1, \ldots, s$.
***Implementation***: *As stated in Corollary A.3, pre-activation bounds of the 4 gates can be computed using Algorithm 3 (Inputs: layer index* $v-1$*, weight matrix* $\mathbf{W}^{ia}/\mathbf{W}^{fa}/\mathbf{W}^{ga}/\mathbf{W}^{oa}$*, bias vector* $\mathbf{b}^{i}/\mathbf{b}^{f}/\mathbf{b}^{g}/\mathbf{b}^{o}$*, bounding planes* $[h^{oc(1)}_{L/U}, \ldots, h^{oc(v-1)}_{L/U}]$, $[h^{fc(1)}_{L/U}, \ldots, h^{fc(v-1)}_{L/U}]$ *and* $[h^{ig(1)}_{L/U}, \ldots, h^{ig(v-1)}_{L/U}]$*, the LSTM, LSTM input sequence* $[\mathbf{x}^{(1)}, \ldots, \mathbf{x}^{(v)}]$*, p-norm,* $\epsilon$*). Note that when* $v = 1$*, the upper and lower bounds can be directly computed according to the definitions of the 4 gates without using the bounding planes* $h^{oc}_{L/U}$, $h^{fc}_{L/U}$, $h^{ig}_{L/U}$.

**Algorithm 5** *Compute lower and upper bounds for the cell state* $\mathbf{c}^{(v)}$
***Input***: *layer index* $v$ *(range from* $0$ *to* $m$*), bounding planes* $[h^{oc(1)}_{L/U}, \ldots, h^{oc(v-1)}_{L/U}]$, $[h^{fc(1)}_{L/U}, \ldots, h^{fc(v)}_{L/U}]$ *and* $[h^{ig(1)}_{L/U}, \ldots, h^{ig(v)}_{L/U}]$, *an* $m$*-layer LSTM, LSTM input sequence* $[\mathbf{x}^{(1)}, \ldots, \mathbf{x}^{(v)}]$, *p-norm,* $\epsilon$.
***Output***: *lower bound* $\mathbf{l}^{c(v)}_j$ *and upper bound* $\mathbf{u}^{c(v)}_j$, $j = 1, \ldots, s$.
***Implementation***: *Implementation details are stated in Theorem A.4. Note that when* $v = 0$*, both the lower bound and upper bound of* $\mathbf{c}^{(0)}$ *is just* $\mathbf{c}^{(0)}$ *itself. No bounding plane is needed in this case. And when* $v = 1$*,* $h^{oc}_{L/U}$ *is actually not needed either.*

Now we have got all the necessary auxiliary algorithms to compute lower and upper bounds of the final output $\mathbf{W}^{Fa}\mathbf{a}^{(m)} + \mathbf{b}^{F}$ of an $m$-layer LSTM. Algorithm 3, Algorithm 4 and Algorithm 5 will be used iteratively to compute bounds for the final output of an LSTM. The resulting algorithm is stated below.

**Algorithm 6** *Compute lower and upper bounds for the final output* $\mathbf{W}^{Fa}\mathbf{a}^{(m)} + \mathbf{b}^{F}$ *of an* $m$*-layer LSTM*
***Input***: *an* $m$*-layer LSTM, LSTM input sequence* $[\mathbf{x}^{(1)}, \ldots, \mathbf{x}^{(m)}]$, *p-norm,* $\epsilon$.
***Output***: *lower bound* $(\mathbf{W}^{Fa}\mathbf{a}^{(m)} + \mathbf{b}^{F})_{L,j}$ *and upper bounds* $(\mathbf{W}^{Fa}\mathbf{a}^{(m)} + \mathbf{b}^{F})_{U,j}$, $j = 1, \ldots, t$.

***for*** *v=1,...,m* ***do***
    ***for*** *j=1,...,s* ***do***
        $\mathbf{l}^{i(v)}_j$, $\mathbf{l}^{f(v)}_j$, $\mathbf{l}^{g(v)}_j$, $\mathbf{l}^{o(v)}_j$, $\mathbf{u}^{i(v)}_j$, $\mathbf{u}^{f(v)}_j$, $\mathbf{u}^{g(v)}_j$, $\mathbf{u}^{o(v)}_j$ $\leftarrow$ *Algorithm 4 (Inputs: layer index* $v$*, bounding planes* $[h^{oc(1)}_{L/U}, \ldots, h^{oc(v-1)}_{L/U}]$, $[h^{fc(1)}_{L/U}, \ldots, h^{fc(v-1)}_{L/U}]$ *and* $[h^{ig(1)}_{L/U}, \ldots, h^{ig(v-1)}_{L/U}]$*, the LSTM, LSTM input sequence* $[\mathbf{x}^{(1)}, \ldots, \mathbf{x}^{(v)}]$*, p-norm,* $\epsilon$*)*
        $h^{fc(v)}_{L,j}(\mathbf{y}^{f(v)}_j, \mathbf{c}^{(v-1)}_j)$, $h^{fc(v)}_{U,j}(\mathbf{y}^{f(v)}_j, \mathbf{c}^{(v-1)}_j)$ $\leftarrow$ *compute bounding planes for* $\sigma(\mathbf{y}^{f(v)}_j)\mathbf{c}^{(v-1)}_j$ *given* $\mathbf{l}^{f(v)}_j$, $\mathbf{u}^{f(v)}_j$, $\mathbf{l}^{c(v-1)}_j$, $\mathbf{u}^{c(v-1)}_j$ *(Note* $\mathbf{l}^{c(0)}_j = \mathbf{u}^{c(0)}_j = \mathbf{c}^{(0)}_j$*)*
        $h^{ig(v)}_{L,j}(\mathbf{y}^{i(v)}_j, \mathbf{y}^{g(v)}_j)$, $h^{ig(v)}_{U,j}(\mathbf{y}^{i(v)}_j, \mathbf{y}^{g(v)}_j)$ $\leftarrow$ *compute bounding planes for* $\sigma(\mathbf{y}^{i(v)}_j)\tanh(\mathbf{y}^{g(v)}_j)$ *given* $\mathbf{l}^{i(v)}_j$, $\mathbf{u}^{i(v)}_j$, $\mathbf{l}^{g(v)}_j$, $\mathbf{u}^{g(v)}_j$
        $\mathbf{l}^{c(v)}_j$, $\mathbf{u}^{c(v)}_j$ $\leftarrow$ *Algorithm 5 (Inputs: layer index* $v$*, bounding planes* $[h^{oc(1)}_{L/U}, \ldots, h^{oc(v-1)}_{L/U}]$, $[h^{fc(1)}_{L/U}, \ldots, h^{fc(v)}_{L/U}]$ *and* $[h^{ig(1)}_{L/U}, \ldots, h^{ig(v)}_{L/U}]$*, the LSTM, LSTM input sequence* $[\mathbf{x}^{(1)}, \ldots, \mathbf{x}^{(v)}]$*, p-norm,* $\epsilon$*)*
        $h^{oc(v)}_{L,j}(\mathbf{y}^{o(v)}_j, \mathbf{c}^{(v)}_j)$, $h^{oc(v)}_{U,j}(\mathbf{y}^{o(v)}_j, \mathbf{c}^{(v)}_j)$ $\leftarrow$ *compute bounding planes for* $\sigma(\mathbf{y}^{o(v)}_j)\tanh(\mathbf{c}^{(v)}_j)$ *given* $\mathbf{l}^{o(v)}_j$, $\mathbf{u}^{o(v)}_j$, $\mathbf{l}^{c(v)}_j$, $\mathbf{u}^{c(v)}_j$
    ***end for***
***end for***
$(\mathbf{W}^{Fa}\mathbf{a}^{(m)} + \mathbf{b}^{F})_{L,j}$, $(\mathbf{W}^{Fa}\mathbf{a}^{(m)} + \mathbf{b}^{F})_{U,j}$, $j = 1, \ldots, t$ $\leftarrow$ *Algorithm 3 (Inputs: layer index* $m$*, weight matrix* $\mathbf{W}^{Fa}$ *and bias vector* $\mathbf{b}^{F}$*, bounding planes* $[h^{oc(1)}_{L/U}, \ldots, h^{oc(v)}_{L/U}]$, $[h^{fc(1)}_{L/U}, \ldots, h^{fc(v)}_{L/U}]$ *and* $[h^{ig(1)}_{L/U}, \ldots, h^{ig(v)}_{L/U}]$*, the LSTM, LSTM input sequence* $[\mathbf{x}^{(1)}, \ldots, \mathbf{x}^{(m)}]$*, p-norm,* $\epsilon$*)*

Finally, we can use Algorithm 6 to get a robustness bound for an LSTM through a binary search procedure. Assume the true class of the sequence $[\mathbf{x}^{(1)}, \ldots, \mathbf{x}^{(m)}]$ is $c$. The algorithm to certify the largest possible lower bound of targeted attacks (target class be $i$) is stated below.

**Algorithm 7** *Compute POPQORN robustness bound of an* $m$*-layer LSTM*
***Input***: *an* $m$*-layer LSTM, LSTM input sequence* $[\mathbf{x}^{(1)}, \ldots, \mathbf{x}^{(m)}]$, *p-norm,* $\epsilon_0$.
***Output***: *a robustness bound* $\tilde{\epsilon}$.

*Replace the last layer weights* $\overline{\mathbf{w}} \leftarrow \mathbf{W}^{Fa}_{c,:} - \mathbf{W}^{Fa}_{i,:}$
*Initialize* $\epsilon \leftarrow \epsilon_0$
***while*** *$\epsilon$ has not achieved a desired accuracy and iteration limit has not reached* ***do***
    $\gamma^L, \gamma^U \leftarrow$ *Algorithm 6 (Inputs: the LSTM, LSTM input sequence* $[\mathbf{x}^{(1)}, \ldots, \mathbf{x}^{(m)}]$, *p-norm,* $\epsilon$*)*
    ***if*** $\gamma^L \geq 0$ ***then***
        *$\epsilon$ is a lower bound; increase $\epsilon$ using a binary search procedure*
    ***else***
        *$\epsilon$ is not a lower bound; decrease $\epsilon$ using a binary search procedure*
    ***end if***
    $\tilde{\epsilon} \leftarrow \epsilon$
***end while***

### A.6 Long Short-term Memory Network (1D bounding lines)

**Theorem A. 5 (Explicit output bound of long short-term memory network F with 1D bounding technique)** *Given an $m$-layer long short-term memory network $F : \mathbb{R}^{n\times m} \to \mathbb{R}^t$, we can derive two explicit functions $F_j^L : \mathbb{R}^{n\times m} \to \mathbb{R}$ and $F_j^U : \mathbb{R}^{n\times m} \to \mathbb{R}$ such that $\forall\ j \in [t]$ and $\forall\ \mathbf{X} \in \mathbb{R}^{n\times m}$ where $\mathbf{x}^{(k)} \in \mathbb{B}_p(\mathbf{x}_0^{(k)}, \epsilon)$, the inequity $F_j^L(\mathbf{X}) \leq F_j(\mathbf{X}) \leq F_j^U(\mathbf{X})$ holds true. We can obtain them through following steps: Starting from $k = m$, $\forall r \in s$ we*

**1. define unified slopes and intercepts;**

$$\lambda_{j,r}^{(k)} = \begin{cases} \alpha_{U,r}^{(k)} & \textit{if} \ \ \tilde{\mathbf{W}}_{U,j,r}^{a(k+1)} \geq 0; \\ \alpha_{L,r}^{o} & \textit{if} \ \ \tilde{\mathbf{W}}_{U,j,r}^{a(k+1)} < 0; \end{cases} \quad \omega_{j,r}^{(k)} = \begin{cases} \alpha_{L,r}^{(k)} & \textit{if} \ \ \tilde{\mathbf{W}}_{L,j,r}^{a(k+1)} \geq 0; \\ \alpha_{U,r}^{(k)} & \textit{if} \ \ \tilde{\mathbf{W}}_{L,j,r}^{a(k+1)} < 0; \end{cases}$$

$$\mathbf{\Delta}_{j,r}^{(k)} = \begin{cases} \beta_{U,r}^{(k)} & \textit{if} \ \ \tilde{\mathbf{W}}_{U,j,r}^{a(k+1)} \geq 0; \\ \beta_{L,r}^{(k)} & \textit{if} \ \ \tilde{\mathbf{W}}_{U,j,r}^{a(k+1)} < 0; \end{cases} \quad \mathbf{\Theta}_{j,r}^{(k)} = \begin{cases} \beta_{L,r}^{(k)} & \textit{if} \ \ \tilde{\mathbf{W}}_{L,j,r}^{a(k+1)} \geq 0; \\ \beta_{U,r}^{(k)} & \textit{if} \ \ \tilde{\mathbf{W}}_{L,j,r}^{a(k+1)} < 0; \end{cases}$$

*where* $\tilde{\mathbf{W}}_{U,j,r}^{a(m+1)} = \tilde{\mathbf{W}}_{L,j,r}^{a(m+1)} = \mathbf{W}_{j,r}^{Fa}$;

**2. collect coefficients in front of *pre-activation*, and constants;**

$$\mathbf{\Lambda}_{\lambda,j,:}^{(k)} = \begin{cases} \mathbf{W}_{j,:}^{Fa} \odot \lambda_{j,:}^{(k)} & \textit{if} \ \ k = m; \\ \tilde{\mathbf{W}}_{U,j,:}^{a(k+1)} \odot \lambda_{j,:}^{(k)} & \textit{if} \ \ k \in [m-1]; \end{cases} \quad \mathbf{\Omega}_{\omega,j,:}^{(k)} = \begin{cases} \mathbf{W}_{j,:}^{Fa} \odot \omega_{j,:}^{(k)} & \textit{if} \ \ k = m; \\ \tilde{\mathbf{W}}_{L,j,:}^{a(k+1)} \odot \omega_{j,:}^{(k)} & \textit{if} \ \ k \in [m-1]; \end{cases}$$

$$\mathbf{\Lambda}_{\Delta,j,:}^{(k)} = \begin{cases} \mathbf{W}_{j,:}^{Fa} \odot \mathbf{\Delta}_{j,:}^{(k)} & \textit{if} \ \ k = m; \\ \tilde{\mathbf{W}}_{U,j,:}^{a(k+1)} \odot \mathbf{\Delta}_{j,:}^{(k)} & \textit{if} \ \ k \in [m-1]; \end{cases} \quad \mathbf{\Omega}_{\Theta,j,:}^{(k)} = \begin{cases} \mathbf{W}_{j,:}^{Fa} \odot \mathbf{\Theta}_{j,:}^{(k)} & \textit{if} \ \ k = m; \\ \tilde{\mathbf{W}}_{L,j,:}^{a(k+1)} \odot \mathbf{\Theta}_{j,:}^{(k)} & \textit{if} \ \ k \in [m-1]; \end{cases}$$

**3. define equivalent weight matrices and biases;**

$$\tilde{\mathbf{W}}_{U,j,q_k}^{x(k)} = \mathbf{\Lambda}_{\lambda,j,:}^{(k)} \mathbf{W}_{:,q_k}^{ox}, \qquad \tilde{\mathbf{W}}_{U,j,r}^{a(k)} = \mathbf{\Lambda}_{\lambda,j,:}^{(k)} \mathbf{W}_{:,r}^{oa}, \qquad \tilde{\mathbf{b}}_{U,j}^{(k)} = \mathbf{\Lambda}_{\lambda,j,:}^{(k)} \mathbf{b}^o + \sum_{i=1}^{s} \mathbf{\Lambda}_{\Delta,j,i}^{(k)};$$

$$\tilde{\mathbf{W}}_{L,j,q_k}^{x(k)} = \mathbf{\Omega}_{\omega,j,:}^{o} \mathbf{W}_{:,q_k}^{ox}, \qquad \tilde{\mathbf{W}}_{L,j,r}^{a(k)} = \mathbf{\Omega}_{\omega,j,:}^{(k)} \mathbf{W}_{:,r}^{oa}, \qquad \tilde{\mathbf{b}}_{L,j}^{(k)} = \mathbf{\Omega}_{\omega,j,:}^{(k)} \mathbf{b}^o + \sum_{i=1}^{s} \mathbf{\Omega}_{\Theta,j,i}^{oc(k)};$$

**4. After looping steps 1 to 3 from $k = m$ to $k = 1$, the bounds are given by**

$$F_j^U(\mathbf{X}) = \tilde{\mathbf{W}}_{U,j,:}^{a(1)} \mathbf{a}^{(0)} + \sum_{k=1}^{m} \tilde{\mathbf{W}}_{U,j,:}^{x(k)} \mathbf{x}^{(k)} + \sum_{k=1}^{m} \tilde{\mathbf{b}}_{U,j}^{(k)} + \mathbf{b}_j^F,$$

$$F_j^L(\mathbf{X}) = \tilde{\mathbf{W}}_{L,j,:}^{a(1)} \mathbf{a}^{(0)} + \sum_{k=1}^{m} \tilde{\mathbf{W}}_{L,j,:}^{x(k)} \mathbf{x}^{(k)} + \sum_{k=1}^{m} \tilde{\mathbf{b}}_{L,j}^{(k)} + \mathbf{b}_j^F.$$

***Proof 4*** *Given an $m$-layer long short-term memory network $F : \mathbb{R}^{n\times m} \to \mathbb{R}^t$ with pre-activation bounds $\mathbf{l}^{o(k)}$,$\mathbf{u}^{o(k)}$, $\mathbf{l}^{c(k)}$,$\mathbf{u}^{c(k)}$ for $\mathbf{X} \in \mathbb{R}^{n\times m}$, where $\mathbf{x}^{(k)} \in \mathbb{B}_p(\mathbf{x}_0^{(k)}, \epsilon)$, let the pre-activation inputs for the $j$-th neuron at the output*

*layer be* $F_j(\mathbf{X}) = \mathbf{W}^{Fa}_{j,:}\mathbf{a}^{(m)} + \mathbf{b}^F_j$*. The* $j$*-th output of the recurrent neural network is the following:*

$$
\begin{aligned}
F_j(\mathbf{X}) &= \mathbf{W}^{Fa}_{j,:}\mathbf{a}^{(m)} + \mathbf{b}^F_j, \\
&= \sum_{i=1}^{s} \mathbf{W}^{Fa}_{j,i}\mathbf{a}^{(m)}_i + \mathbf{b}^F_j, \\
&= \sum_{i=1}^{s} \mathbf{W}^{Fa}_{j,i}[\mathbf{o}^{(m)}_i \tanh(\mathbf{c}^{(m)}_i)] + \mathbf{b}^F_j, \\
&= \sum_{i=1}^{s} \mathbf{W}^{Fa}_{j,i}[\sigma(\mathbf{y}^{o(m)}_i) \tanh(\mathbf{c}^{(m)}_i)] + \mathbf{b}^F_j, \\
&= \sum_{\mathbf{W}^{Fa}_{j,i}\geq 0} \mathbf{W}^{Fa}_{j,i}[\sigma(\mathbf{y}^{o(m)}_i) \tanh(\mathbf{c}^{(m)}_i)] + \sum_{\mathbf{W}^{Fa}_{j,i}< 0} \mathbf{W}^{Fa}_{j,i}[\sigma(\mathbf{y}^{o(m)}_i) \tanh(\mathbf{c}^{(m)}_i)] + \mathbf{b}^F_j.
\end{aligned}
$$

*Assume* $\mathbf{c}^{(m)}_i$ *is bounded by* $\mathbf{l}^{c(m)}$,$\mathbf{u}^{c(m)}$, $\tanh(\mathbf{c}^{(m)}_i)$ *can be bounded by* $\mathbf{c}^{(m)}_{U,i}$ *and* $\mathbf{c}^{(m)}_{L,i}$*, such that* $\mathbf{c}^{(m)}_{L,i} \leq \tanh(\mathbf{c}^{(m)}_i) \leq \mathbf{c}^{(m)}_{U,i}$*. We also assume the positive activation function* $\sigma(\mathbf{y})$ *is bounded by two linear functions* $h^{(m)}_{L,i}(\mathbf{y})$*,* $h^{(m)}_{U,i}(\mathbf{y})$*, which yield* $H^{(m)}_{L,i}(\mathbf{y}) \leq \sigma(\mathbf{y}^{o(m)}_i)\tanh(\mathbf{c}^{(m)}_i) \leq H^{(m)}_{U,i}(\mathbf{y})$*, where*

$$
\begin{aligned}
H^{(m)}_{L,i}(\mathbf{y}) &= \mathbb{1}_{\mathbf{c}^{(m)}_{L,i}\leq 0} h^{(m)}_{U,i}(\mathbf{y}^{o(m)}_i)\mathbf{c}^{(m)}_{L,i} + \mathbb{1}_{\mathbf{c}^{(m)}_{L,i}> 0} h^{(m)}_{L,i}(\mathbf{y}^{o(m)}_i)\mathbf{c}^{(m)}_{L,i}; \\
H^{(m)}_{U,i}(\mathbf{y}) &= \mathbb{1}_{\mathbf{c}^{(m)}_{U,i}\geq 0} h^{(m)}_{U,i}(\mathbf{y}^{o(m)}_i)\mathbf{c}^{(m)}_{U,i} + \mathbb{1}_{\mathbf{c}^{(m)}_{U,i}< 0} h^{(m)}_{L,i}(\mathbf{y}^{o(m)}_i)\mathbf{c}^{(m)}_{U,i}.
\end{aligned}
$$

***Upper bound.*** *We can then obtain*

$$
\begin{aligned}
F_j(\mathbf{X}) &\leq \sum_{\mathbf{W}^{Fa}_{j,i}\geq 0} \mathbf{W}^{Fa}_{j,i} H^{(m)}_{U,i}(\mathbf{y}^{o(m)}_i) + \sum_{\mathbf{W}^{Fa}_{j,i}< 0} \mathbf{W}^{Fa}_{j,i} H^{(m)}_{L,i}(\mathbf{y}^{o(m)}_i) + \mathbf{b}^F_j, \\
&= \sum_{\mathbf{W}^{Fa}_{j,i}\geq 0} \mathbf{W}^{Fa}_{j,i}\ (\alpha^{(m)}_{U,i}\mathbf{y}^{o(m)}_i + \beta^{(m)}_{U,i}) + \sum_{\mathbf{W}^{Fa}_{j,i}< 0} \mathbf{W}^{fa}_{j,i}\ (\alpha^{(m)}_{L,i}\mathbf{y}^{o(m)}_i + \beta^{(m)}_{L,i}) + \mathbf{b}^F_j.
\end{aligned}
$$

*We then define* $\lambda^{(m)}_{j,i}$ *and* $\boldsymbol{\Delta}^{(m)}_{j,i}$ *in the parentheses:*

$$
\lambda^{(m)}_{j,i} = \begin{cases} \alpha^{(m)}_{U,i} & \text{if } \mathbf{W}^{Fa}_{j,i} \geq 0; \\ \alpha^{(m)}_{L,i} & \text{if } \mathbf{W}^{Fa}_{j,i} < 0; \end{cases} \qquad \boldsymbol{\Delta}^{(m)}_{j,i} = \begin{cases} \beta^{(m)}_{U,i} & \text{if } \mathbf{W}^{Fa}_{j,i} \geq 0; \\ \beta^{(m)}_{L,i} & \text{if } \mathbf{W}^{Fa}_{j,i} < 0; \end{cases}
$$

*and obtain*

$$
F_j(\mathbf{X}) \leq \sum_{i=1}^{s} \mathbf{W}^{Fa}_{j,i}\ (\lambda^{(m)}_{j,i}\mathbf{y}^{o(m)}_i + \boldsymbol{\Delta}^{(m)}_{j,i}) + \mathbf{b}^F_j.
$$

*We further let* $\boldsymbol{\Lambda}^{(m)}_{\lambda,j,i} := \mathbf{W}^{Fa}_{j,i}\ \lambda^{(m)}_{j,i}$, $\boldsymbol{\Lambda}^{(m)}_{\Delta,j,i} := \mathbf{W}^{Fa}_{j,i}\ \boldsymbol{\Delta}^{(m)}_{j,i}$*, and we have*

$$
\begin{aligned}
F_j(\mathbf{X}) &\leq \sum_{i=1}^{s}(\boldsymbol{\Lambda}^{(m)}_{\lambda,j,i}\mathbf{y}^{o(m)}_i + \boldsymbol{\Lambda}^{(m)}_{\Delta,j,i}) + \mathbf{b}^F_j, \\
&= \sum_{i=1}^{s}[\boldsymbol{\Lambda}^{(m)}_{\lambda,j,i}(\mathbf{W}^{ox}_{i,:}\mathbf{x}^{(m)} + \mathbf{W}^{oa}_{i,:}\mathbf{a}^{(m-1)} + \mathbf{b}^o_i) + \boldsymbol{\Lambda}^{(m)}_{\Delta,j,i}] + \mathbf{b}^F_j, \\
&= \sum_{q_m=1}^{n}(\sum_{i=1}^{s}\boldsymbol{\Lambda}^{(m)}_{\lambda,j,i}\mathbf{W}^{ox}_{i,q_m})\mathbf{x}^{(m)}_{q_m} + \sum_{r=1}^{s}(\sum_{i=1}^{s}\boldsymbol{\Lambda}^{(m)}_{\lambda,j,i}\mathbf{W}^{oa}_{i,r})\mathbf{a}^{(m-1)}_r + \sum_{i=1}^{s}(\boldsymbol{\Lambda}^{(m)}_{\lambda,j,i}\mathbf{b}^o_i + \boldsymbol{\Lambda}^{(m)}_{\Delta,j,i}) + \mathbf{b}^F_j, \\
&= \sum_{q_m=1}^{n}(\boldsymbol{\Lambda}^{(m)}_{\lambda,j,:}\mathbf{W}^{ox}_{:,q_m})\mathbf{x}^{(m)}_{q_m} + \sum_{r=1}^{s}(\boldsymbol{\Lambda}^{(m)}_{\lambda,j,:}\mathbf{W}^{oa}_{:,r})\mathbf{a}^{(m-1)}_r + \boldsymbol{\Lambda}^{(m)}_{\lambda,j,:}\mathbf{b}^o + \sum_{i=1}^{s}\boldsymbol{\Lambda}^{(m)}_{\Delta,j,i} + \mathbf{b}^F_j.
\end{aligned}
$$

*We combine coefficients above into equivalent weights $\tilde{\mathbf{W}}^{x(m)}_{U,j,q_m}$, $\tilde{\mathbf{W}}^{a(m)}_{U,j,r}$ and bias $\tilde{\mathbf{b}}^{(m)}_{U,j}$ as defined by*

$$\tilde{\mathbf{W}}^{x(m)}_{U,j,q_m} = \mathbf{\Lambda}^{(m)}_{\lambda,j,:}\mathbf{W}^{ox}_{:,q_m}, \quad \tilde{\mathbf{W}}^{a(m)}_{U,j,r} = \mathbf{\Lambda}^{(m)}_{\lambda,j,:}\mathbf{W}^{oa}_{:,r}, \quad \tilde{\mathbf{b}}^{(m)}_{U,j} = \mathbf{\Lambda}^{(m)}_{\lambda,j,:}\mathbf{b}^{o} + \sum_{i=1}^{s}\mathbf{\Lambda}^{(m)}_{\Delta,j,i},$$

*and obtain*

$$\begin{aligned}
F_j(\mathbf{X}) \le F_j^{U,m}(\mathbf{X}) &= \tilde{\mathbf{W}}^{x(m)}_{U,j,:}\mathbf{x}^{(m)} + \tilde{\mathbf{W}}^{a(m)}_{U,j,:}\mathbf{a}^{(m-1)} + \tilde{\mathbf{b}}^{(m)}_{U,j} + \mathbf{b}^F_j, \\
&= \tilde{\mathbf{W}}^{x(m)}_{U,j,:}\mathbf{x}^{(m)} + \tilde{\mathbf{b}}^{(m)}_{U,j} + \mathbf{b}^F_j + \tilde{\mathbf{W}}^{a(m)}_{U,j,:}[\mathbf{o}^{(m-1)}\tanh(\mathbf{c}^{(m-1)})] \\
&= \tilde{\mathbf{W}}^{x(m)}_{U,j,:}\mathbf{x}^{(m)} + \tilde{\mathbf{b}}^{(m)}_{U,j} + \mathbf{b}^F_j \\
&+ \sum_{\tilde{\mathbf{W}}^{a(m)}_{U,j,i}\ge 0} \tilde{\mathbf{W}}^{a(m)}_{U,j,i}[\sigma(\mathbf{y}_i^{o(m-1)})\tanh(\mathbf{c}_i^{(m-1)})] + \sum_{\tilde{\mathbf{W}}^{a(m)}_{U,j,i}< 0} \tilde{\mathbf{W}}^{a(m)}_{U,j,i}[\sigma(\mathbf{y}_i^{o(m-1)})\tanh(\mathbf{c}_i^{(m-1)})].
\end{aligned}$$

*Assume $\mathbf{c}_i^{(m-1)}$ is bounded by $\mathbf{l}^{c(m-1)}$,$\mathbf{u}^{c(m-1)}$, $\tanh(\mathbf{c}_i^{(m-1)})$ can be bounded by $\mathbf{c}^{(m-1)}_{U,i}$ and $\mathbf{c}^{(m-1)}_{L,i}$, such that $\mathbf{c}^{(m-1)}_{L,i} \le \tanh(\mathbf{c}_i^{(m-1)}) \le \mathbf{c}^{(m-1)}_{U,i}$. We also assume the positive activation function $\sigma(\mathbf{y})$ is bounded by two linear functions $h^{(m-1)}_{L,i}(\mathbf{y})$, $h^{(m-1)}_{U,i}(\mathbf{y})$, which yield $H^{(m-1)}_{L,i}(\mathbf{y}) \le \sigma(\mathbf{y}_i^{o(m-1)})\tanh(\mathbf{c}_i^{(m-1)}) \le H^{(m-1)}_{U,i}(\mathbf{y})$, where*

$$\begin{aligned}
H^{(m-1)}_{L,i}(\mathbf{y}) &= \mathbb{1}_{\mathbf{c}^{(m-1)}_{L,i}\le 0} h^{(m-1)}_{U,i}(\mathbf{y}_i^{o(m-1)})\mathbf{c}^{(m-1)}_{L,i} + \mathbb{1}_{\mathbf{c}^{(m-1)}_{L,i}> 0} h^{(m-1)}_{L,i}(\mathbf{y}_i^{o(m-1)})\mathbf{c}^{(m-1)}_{L,i}; \\
H^{(m-1)}_{U,i}(\mathbf{y}) &= \mathbb{1}_{\mathbf{c}^{(m-1)}_{U,i}\ge 0} h^{(m-1)}_{U,i}(\mathbf{y}_i^{o(m-1)})\mathbf{c}^{(m-1)}_{U,i} + \mathbb{1}_{\mathbf{c}^{(m-1)}_{U,i}< 0} h^{(m-1)}_{L,i}(\mathbf{y}_i^{o(m-1)})\mathbf{c}^{(m-1)}_{U,i}.
\end{aligned}$$

*We can then obtain*

$$\begin{aligned}
F_j^{U,m}(\mathbf{X}) &\le \tilde{\mathbf{W}}^{x(m)}_{U,j,:}\mathbf{x}^{(m)} + \tilde{\mathbf{b}}^{(m)}_{U,j} + \mathbf{b}^F_j \\
&+ \sum_{\tilde{\mathbf{W}}^{a(m)}_{U,j,i}\ge 0} \tilde{\mathbf{W}}^{a(m)}_{U,j,i}\,(\alpha^{(m-1)}_{U,i}\mathbf{y}_i^{o(m-1)} + \beta^{(m-1)}_{U,i}) + \sum_{\tilde{\mathbf{W}}^{a(m)}_{U,j,i}< 0} \tilde{\mathbf{W}}^{a(m)}_{U,j,i}\,(\alpha^{(m-1)}_{L,i}\mathbf{y}_i^{o(m-1)} + \beta^{(m-1)}_{L,i}).
\end{aligned}$$

*We then define $\lambda^{(m-1)}_{j,i}$ and $\mathbf{\Delta}^{(m-1)}_{j,i}$ in the parentheses:*

$$\lambda^{(m-1)}_{j,i} = \begin{cases} \alpha^{(m-1)}_{U,i} & \text{if } \tilde{\mathbf{W}}^{a(m)}_{U,j,i} \ge 0; \\ \alpha^{(m-1)}_{L,i} & \text{if } \tilde{\mathbf{W}}^{a(m)}_{U,j,i} < 0; \end{cases} \qquad \mathbf{\Delta}^{(m-1)}_{j,i} = \begin{cases} \beta^{(m-1)}_{U,i} & \text{if } \tilde{\mathbf{W}}^{a(m)}_{U,j,i} \ge 0; \\ \beta^{(m-1)}_{L,i} & \text{if } \tilde{\mathbf{W}}^{a(m)}_{U,j,i} < 0; \end{cases}$$

*and obtain*

$$F_j^{U,m}(\mathbf{X}) \le \tilde{\mathbf{W}}^{x(m)}_{U,j,:}\mathbf{x}^{(m)} + \tilde{\mathbf{b}}^{(m)}_{U,j} + \mathbf{b}^F_j + \sum_{i=1}^{s}\tilde{\mathbf{W}}^{a(m)}_{U,j,i}\,(\lambda^{(m-1)}_{j,i}\mathbf{y}_i^{o(m-1)} + \mathbf{\Delta}^{(m-1)}_{j,i}).$$

*We further let $\mathbf{\Lambda}^{(m-1)}_{\lambda,j,i} := \tilde{\mathbf{W}}^{a(m)}_{U,j,i}\ \lambda^{(m-1)}_{j,i}$, $\quad \mathbf{\Lambda}^{(m-1)}_{\Delta,j,i} := \tilde{\mathbf{W}}^{a(m)}_{U,j,i}\ \mathbf{\Delta}^{(m-1)}_{j,i}$ and we have*

$$F_j^{U,m}(\mathbf{X}) \le \tilde{\mathbf{W}}^{x(m)}_{U,j,:}\mathbf{x}^{(m)} + \tilde{\mathbf{b}}^{(m)}_{U,j} + \sum_{i=1}^{s}(\mathbf{\Lambda}^{(m-1)}_{\lambda,j,i}\mathbf{y}_i^{o(m-1)} + \mathbf{\Lambda}^{(m-1)}_{\Delta,j,i}) + \mathbf{b}^F_j.$$

*Similarly, $\forall r \in s$ we can define variables as follows:*

$$\tilde{\mathbf{W}}^{x(m-1)}_{U,j,q_{m-1}} = \mathbf{\Lambda}^{(m-1)}_{\lambda,j,:}\mathbf{W}^{ox}_{:,q_{m-1}};\ \tilde{\mathbf{W}}^{a(m-1)}_{U,j,r} = \mathbf{\Lambda}^{(m-1)}_{\lambda,j,:}\mathbf{W}^{oa}_{:,r};\ \tilde{\mathbf{b}}^{(m-1)}_{U,j} = \mathbf{\Lambda}^{(m-1)}_{\lambda,j,:}\mathbf{b}^{o} + \sum_{i=1}^{s}\mathbf{\Lambda}^{(m-1)}_{\Delta,j,i}.$$

*Then we can obtain*

$$\begin{aligned}
F_j^{U,m}(\mathbf{X}) \le F_j^{U,m-1}(\mathbf{X}) &= \tilde{\mathbf{W}}^{x(m)}_{U,j,:}\mathbf{x}^{(m)} + \tilde{\mathbf{W}}^{x(m-1)}_{U,j,:}\mathbf{x}^{(m-1)} + \tilde{\mathbf{W}}^{a(m-1)}_{U,j,:}\mathbf{a}^{(m-2)} \\
&+ \tilde{\mathbf{b}}^{(m)}_{U,j} + \tilde{\mathbf{b}}^{(m-1)}_{U,j} + \mathbf{b}^F_j.
\end{aligned}$$

*Thus, we can repeat the above procedure iteratively until we obtain the final upper bound $F_j^{U,1}(\mathbf{X})$, where $F_j(\mathbf{X}) \leq F_j^{U,m}(\mathbf{X}) \leq \cdots \leq F_j^{U,1}(\mathbf{X})$. We let $F_j^U(\mathbf{X})$ denote the final upper bound $F_j^{U,1}(\mathbf{X})$, and we have*

$$F_j^U(\mathbf{X}) = \tilde{\mathbf{W}}_{U,j,:}^{a(1)}\mathbf{a}^{(0)} + \sum_{k=1}^{m} \tilde{\mathbf{W}}_{U,j,:}^{x(k)}\mathbf{x}^{(k)} + \sum_{k=1}^{m} \tilde{\mathbf{b}}_{U,j}^{(k)} + \mathbf{b}_j^F,$$

*where*

$$\tilde{\mathbf{W}}_{U,j,q_k}^{x(k)} = \mathbf{\Lambda}_{\lambda,j,:}^{(k)}\mathbf{W}_{:,q_k}^{ox}, \quad \tilde{\mathbf{W}}_{U,j,r}^{a(k)} = \mathbf{\Lambda}_{\lambda,j,:}^{(k)}\mathbf{W}_{:,r}^{oa}, \quad \tilde{\mathbf{b}}_{U,j}^{(k)} = \mathbf{\Lambda}_{\lambda,j,:}^{(k)}\mathbf{b}^o + \sum_{i=1}^{s} \mathbf{\Lambda}_{\Delta,j,i}^{(k)},$$

*and ($\odot$ is the Hadamard product)*

$$\mathbf{\Lambda}_{\lambda,j,:}^{(k)} = \begin{cases} \mathbf{W}_{j,:}^{Fa} \odot \lambda_{j,:}^{(k)} & \text{if } \ k = m; \\ \tilde{\mathbf{W}}_{U,j,:}^{a(k+1)} \odot \lambda_{j,:}^{(k)} & \text{if } \ k \in [m-1]; \end{cases} \quad \mathbf{\Lambda}_{\Delta,j,:}^{(k)} = \begin{cases} \mathbf{W}_{j,:}^{Fa} \odot \mathbf{\Delta}_{j,:}^{(k)} & \text{if } \ k = m; \\ \tilde{\mathbf{W}}_{U,j,:}^{a(k+1)} \odot \mathbf{\Delta}_{j,:}^{(k)} & \text{if } \ k \in [m-1]; \end{cases}$$

*and $\forall r \in s$,*

$$\lambda_{j,r}^{(m)} = \begin{cases} \alpha_{U,r}^{(m)} & \text{if } \ \mathbf{W}_{j,r}^{Fa} \geq 0; \\ \alpha_{L,r}^{(m)} & \text{if } \ \mathbf{W}_{j,r}^{Fa} < 0; \end{cases} \quad \mathbf{\Delta}_{j,r}^{(m)} = \begin{cases} \beta_{U,r}^{(m)} & \text{if } \ \mathbf{W}_{j,r}^{Fa} \geq 0; \\ \beta_{L,r}^{(m)} & \text{if } \ \mathbf{W}_{j,r}^{Fa} < 0; \end{cases}$$

*and $\forall r \in s, k \in [m-1]$,*

$$\lambda_{j,r}^{(k)} = \begin{cases} \alpha_{U,r}^{(k)} & \text{if } \ \tilde{\mathbf{W}}_{U,j,r}^{a(k+1)} \geq 0; \\ \alpha_{L,r}^{(k)} & \text{if } \ \tilde{\mathbf{W}}_{U,j,r}^{a(k+1)} < 0; \end{cases} \quad \mathbf{\Delta}_{j,r}^{(k)} = \begin{cases} \beta_{U,r}^{(k)} & \text{if } \ \tilde{\mathbf{W}}_{U,j,r}^{a(k+1)} \geq 0; \\ \beta_{L,r}^{(k)} & \text{if } \ \tilde{\mathbf{W}}_{U,j,r}^{a(k+1)} < 0. \end{cases}$$

***Lower bound.*** *The above derivations of upper bound can be applied similarly to derive lower bounds of $F_j(\mathbf{X})$, and the only difference is now we need to use the left-hand side of inequities (rather than right-hand side when deriving upper bound) to bound the activated terms. Thus, following the same procedure in deriving the upper bounds, we can iteratively unwrap the activation functions and obtain a final lower bound $F_j^{L,1}(\mathbf{X})$, where $F_j(\mathbf{X}) \geq F_j^{L,m}(\mathbf{X}) \geq \cdots \geq F_j^{L,1}(\mathbf{X})$. We let $F_j^L(\mathbf{X})$ denote the final lower bound $F_j^{L,1}(\mathbf{X})$, and we have*

$$F_j^L(\mathbf{X}) = \tilde{\mathbf{W}}_{L,j,:}^{a(1)}\mathbf{a}^{(0)} + \sum_{k=1}^{m} \tilde{\mathbf{W}}_{L,j,:}^{x(k)}\mathbf{x}^{(k)} + \sum_{k=1}^{m} \tilde{\mathbf{b}}_{L,j}^{(k)} + \mathbf{b}_j^F,$$

*where*

$$\tilde{\mathbf{W}}_{L,j,q_k}^{x(k)} = \mathbf{\Omega}_{\omega,j,:}^{(k)}\mathbf{W}_{:,q_k}^{ox}, \quad \tilde{\mathbf{W}}_{L,j,r}^{a(k)} = \mathbf{\Omega}_{\omega,j,:}^{(k)}\mathbf{W}_{:,r}^{oa}, \quad \tilde{\mathbf{b}}_{L,j}^{(k)} = \mathbf{\Omega}_{\omega,j,:}^{(k)}\mathbf{b}^o + \sum_{i=1}^{s} \mathbf{\Omega}_{\Theta,j,i}^{(k)},$$

*and ($\odot$ is the Hadamard product)*

$$\mathbf{\Omega}_{\omega,j,:}^{(k)} = \begin{cases} \mathbf{W}_{j,:}^{Fa} \odot \omega_{j,:}^{(k)} & \text{if } \ k = m; \\ \tilde{\mathbf{W}}_{L,j,:}^{a(k+1)} \odot \omega_{j,:}^{(k)} & \text{if } \ k \in [m-1]; \end{cases} \quad \mathbf{\Omega}_{\Theta,j,:}^{(k)} = \begin{cases} \mathbf{W}_{j,:}^{Fa} \odot \mathbf{\Theta}_{j,:}^{(k)} & \text{if } \ k = m; \\ \tilde{\mathbf{W}}_{L,j,:}^{a(k+1)} \odot \mathbf{\Theta}_{j,:}^{(k)} & \text{if } \ k \in [m-1]; \end{cases}$$

*and $\forall r \in s$,*

$$\omega_{j,r}^{(m)} = \begin{cases} \alpha_{L,r}^{(m)} & \text{if } \ \mathbf{W}_{j,r}^{Fa} \geq 0; \\ \alpha_{U,r}^{(m)} & \text{if } \ \mathbf{W}_{j,r}^{Fa} < 0; \end{cases} \quad \mathbf{\Theta}_{j,r}^{(m)} = \begin{cases} \beta_{L,r}^{(m)} & \text{if } \ \mathbf{W}_{j,r}^{Fa} \geq 0; \\ \beta_{U,r}^{(m)} & \text{if } \ \mathbf{W}_{j,r}^{Fa} < 0; \end{cases}$$

*and $\forall r \in s, k \in [m-1]$,*

$$\omega_{j,r}^{(k)} = \begin{cases} \alpha_{L,r}^{(k)} & \text{if } \ \tilde{\mathbf{W}}_{L,j,r}^{a(k+1)} \geq 0; \\ \alpha_{U,r}^{(k)} & \text{if } \ \tilde{\mathbf{W}}_{L,j,r}^{a(k+1)} < 0; \end{cases} \quad \mathbf{\Theta}_{j,r}^{(k)} = \begin{cases} \beta_{L,r}^{(k)} & \text{if } \ \tilde{\mathbf{W}}_{L,j,r}^{a(k+1)} \geq 0; \\ \beta_{U,r}^{(k)} & \text{if } \ \tilde{\mathbf{W}}_{L,j,r}^{a(k+1)} < 0. \end{cases}$$

**Corollary A. 4 (Closed-form global bounds)** *Given data $\mathbf{X} \in \mathbb{R}^{n\times m}$, $l_p$ ball parameters $p \geq 1$ and $\epsilon \geq 0$. For an $m$-layer long short-term memory network $F : \mathbb{R}^{n\times m} \to \mathbb{R}^t$, there exists two fixed values $\gamma_j^L$ and $\gamma_j^U$ such that $\forall\, \mathbf{X} \in \mathbb{R}^{n\times m}$ where $\mathbf{x}^{(k)} \in \mathbb{B}_p(\mathbf{x}_0^{(k)}, \epsilon)$, and $\forall\, j \in [t]$, $1/q = 1 - 1/p$, the inequity $\gamma_j^L \leq F_j(\mathbf{X}) \leq \gamma_j^U$ holds true, where*

$$\gamma_j^U = \tilde{\mathbf{W}}_{U,j,:}^{a(1)}\mathbf{a}^{(0)} + \sum_{k=1}^{m} \epsilon\|\tilde{\mathbf{W}}_{U,j,:}^{x(k)}\|_q + \sum_{k=1}^{m} \tilde{\mathbf{W}}_{U,j,:}^{x(k)}\mathbf{x}_0^{(k)} + \sum_{k=1}^{m} \tilde{\mathbf{b}}_{U,j}^{(k)} + \mathbf{b}_j^F,$$
$$\gamma_j^L = \tilde{\mathbf{W}}_{L,j,:}^{a(1)}\mathbf{a}^{(0)} - \sum_{k=1}^{m} \epsilon\|\tilde{\mathbf{W}}_{L,j,:}^{x(k)}\|_q + \sum_{k=1}^{m} \tilde{\mathbf{W}}_{L,j,:}^{x(k)}\mathbf{x}_0^{(k)} + \sum_{k=1}^{m} \tilde{\mathbf{b}}_{L,j}^{(k)} + \mathbf{b}_j^F.$$

### A.7 Gated Recurrent Unit Network

**Notations** In the derivation of gated recurrent unit network (GRU), we define the equations as follows:

$$
\begin{aligned}
\text{Reset gate:}\quad & \mathbf{r}^{(k)} = \sigma(\mathbf{y}^{r(k)}) = \sigma(\mathbf{W}^{rx}\mathbf{x}^{(k)} + \mathbf{W}^{ra}\mathbf{a}^{(k-1)} + \mathbf{b}^{r});\\
\text{Update gate:}\quad & \mathbf{z}^{(k)} = \sigma(\mathbf{y}^{z(k)}) = \sigma(\mathbf{W}^{zx}\mathbf{x}^{(k)} + \mathbf{W}^{za}\mathbf{a}^{(k-1)} + \mathbf{b}^{z});\\
\text{New gate:}\quad & \mathbf{n}^{(k)} = \tanh(\mathbf{y}^{n(k)}) = \tanh(\mathbf{W}^{nx}\mathbf{x}^{(k)} + \mathbf{b}^{nx} + \mathbf{r}^{(k)} \odot (\mathbf{W}^{na}\mathbf{a}^{(k-1)} + \mathbf{b}^{na}));\\
\text{Hidden state:}\quad & \mathbf{a}^{(k)} = (1 - \mathbf{z}^{(k)}) \odot \mathbf{n}^{(k)} + \mathbf{z}^{(k)} \odot \mathbf{a}^{(k-1)}.
\end{aligned}
$$

**Theorem A. 6 (Explicit output bound of gated recurrent unit network F)** *Given an $m$-layer gated recurrent unit network $F : \mathbb{R}^{n\times m} \to \mathbb{R}^t$, we can derive two explicit functions $F_j^L : \mathbb{R}^{n\times m} \to \mathbb{R}$ and $F_j^U : \mathbb{R}^{n\times m} \to \mathbb{R}$ such that $\forall\, j \in [t]$ and $\forall\, \mathbf{X} \in \mathbb{R}^{n\times m}$ where $\mathbf{x}^{(k)} \in \mathbb{B}_p(\mathbf{x}_0^{(k)}, \epsilon)$, the inequity $F_j^L(\mathbf{X}) \le F_j(\mathbf{X}) \le F_j^U(\mathbf{X})$ holds true. We can obtain them through following steps: Starting from $k = m$, $\forall r \in s$ we*

**1. define unified slopes and intercepts of cross terms of the update gate and the new gate, the update gate and the hidden state;**

$$
\lambda^{zn(k)}_{j,r} = \begin{cases} \alpha^{zn(k)}_{U,r} & \text{if } \tilde{\mathbf{W}}^{a(k+1)}_{U,j,r} \ge 0;\\ \alpha^{zn(k)}_{L,r} & \text{if } \tilde{\mathbf{W}}^{a(k+1)}_{U,j,r} < 0; \end{cases} \quad
\omega^{zn(k)}_{j,r} = \begin{cases} \alpha^{zn(k)}_{L,r} & \text{if } \tilde{\mathbf{W}}^{a(k+1)}_{L,j,r} \ge 0;\\ \alpha^{zn(k)}_{U,r} & \text{if } \tilde{\mathbf{W}}^{a(k+1)}_{L,j,r} < 0; \end{cases}
$$

$$
\boldsymbol{\Delta}^{zn(k)}_{j,r} = \begin{cases} \beta^{zn(k)}_{U,r} & \text{if } \tilde{\mathbf{W}}^{a(k+1)}_{U,j,r} \ge 0;\\ \beta^{zn(k)}_{L,r} & \text{if } \tilde{\mathbf{W}}^{a(k+1)}_{U,j,r} < 0; \end{cases} \quad
\boldsymbol{\Theta}^{zn(k)}_{j,r} = \begin{cases} \beta^{zn(k)}_{L,r} & \text{if } \tilde{\mathbf{W}}^{a(k+1)}_{L,j,r} \ge 0;\\ \beta^{zn(k)}_{U,r} & \text{if } \tilde{\mathbf{W}}^{a(k+1)}_{L,j,r} < 0; \end{cases}
$$

$$
\varphi^{zn(k)}_{j,r} = \begin{cases} \gamma^{zn(k)}_{U,r} & \text{if } \tilde{\mathbf{W}}^{a(k+1)}_{U,j,r} \ge 0;\\ \gamma^{zn(k)}_{L,r} & \text{if } \tilde{\mathbf{W}}^{a(k+1)}_{U,j,r} < 0; \end{cases} \quad
\psi^{zn(k)}_{j,r} = \begin{cases} \gamma^{zn(k)}_{L,r} & \text{if } \tilde{\mathbf{W}}^{a(k+1)}_{L,j,r} \ge 0;\\ \gamma^{zn(k)}_{U,r} & \text{if } \tilde{\mathbf{W}}^{a(k+1)}_{L,j,r} < 0; \end{cases}
$$

$$
\lambda^{za(k)}_{j,r} = \begin{cases} \alpha^{za(k)}_{U,r} & \text{if } \tilde{\mathbf{W}}^{a(k+1)}_{U,j,r} \ge 0;\\ \alpha^{za(k)}_{L,r} & \text{if } \tilde{\mathbf{W}}^{a(k+1)}_{U,j,r} < 0; \end{cases} \quad
\omega^{za(k)}_{j,r} = \begin{cases} \alpha^{za(k)}_{L,r} & \text{if } \tilde{\mathbf{W}}^{a(k+1)}_{L,j,r} \ge 0;\\ \alpha^{za(k)}_{U,r} & \text{if } \tilde{\mathbf{W}}^{a(k+1)}_{L,j,r} < 0; \end{cases}
$$

$$
\boldsymbol{\Delta}^{za(k)}_{j,r} = \begin{cases} \beta^{za(k)}_{U,r} & \text{if } \tilde{\mathbf{W}}^{a(k+1)}_{U,j,r} \ge 0;\\ \beta^{za(k)}_{L,r} & \text{if } \tilde{\mathbf{W}}^{a(k+1)}_{U,j,r} < 0; \end{cases} \quad
\boldsymbol{\Theta}^{za(k)}_{j,r} = \begin{cases} \beta^{za(k)}_{L,r} & \text{if } \tilde{\mathbf{W}}^{a(k+1)}_{L,j,r} \ge 0;\\ \beta^{za(k)}_{U,r} & \text{if } \tilde{\mathbf{W}}^{a(k+1)}_{L,j,r} < 0; \end{cases}
$$

$$
\varphi^{za(k)}_{j,r} = \begin{cases} \gamma^{za(k)}_{U,r} & \text{if } \tilde{\mathbf{W}}^{a(k+1)}_{U,j,r} \ge 0;\\ \gamma^{za(k)}_{L,r} & \text{if } \tilde{\mathbf{W}}^{a(k+1)}_{U,j,r} < 0; \end{cases} \quad
\psi^{za(k)}_{j,r} = \begin{cases} \gamma^{za(k)}_{L,r} & \text{if } \tilde{\mathbf{W}}^{a(k+1)}_{L,j,r} \ge 0;\\ \gamma^{za(k)}_{U,r} & \text{if } \tilde{\mathbf{W}}^{a(k+1)}_{L,j,r} < 0; \end{cases}
$$

*where* $\tilde{\mathbf{W}}^{a(m+1)}_{U,j,r} = \tilde{\mathbf{W}}^{a(m+1)}_{L,j,r} = \mathbf{W}^{Fa}_{j,r}$*;*

**2. collect coefficients in front of the update gate *pre-activations*, the new gate *pre-activation*, the hidden state, and constants of the two couplings;**

$$
\boldsymbol{\Lambda}^{zn(k)}_{\lambda,j,:} = \begin{cases} \mathbf{W}^{Fa}_{j,:} \odot \lambda^{zn(k)}_{j,:} & \text{if } k = m;\\ \tilde{\mathbf{W}}^{a(k+1)}_{U,j,:} \odot \lambda^{zn(k)}_{j,:} & \text{if } k \in [m-1]; \end{cases} \quad
\boldsymbol{\Omega}^{zn(k)}_{\omega,j,:} = \begin{cases} \mathbf{W}^{Fa}_{j,:} \odot \omega^{zn(k)}_{j,:} & \text{if } k = m;\\ \tilde{\mathbf{W}}^{a(k+1)}_{L,j,:} \odot \omega^{zn(k)}_{j,:} & \text{if } k \in [m-1]; \end{cases}
$$

$$
\boldsymbol{\Lambda}^{zn(k)}_{\Delta,j,:} = \begin{cases} \mathbf{W}^{Fa}_{j,:} \odot \boldsymbol{\Delta}^{zn(k)}_{j,:} & \text{if } k = m;\\ \tilde{\mathbf{W}}^{a(k+1)}_{U,j,:} \odot \boldsymbol{\Delta}^{zn(k)}_{j,:} & \text{if } k \in [m-1]; \end{cases} \quad
\boldsymbol{\Omega}^{zn(k)}_{\Theta,j,:} = \begin{cases} \mathbf{W}^{Fa}_{j,:} \odot \boldsymbol{\Theta}^{zn(k)}_{j,:} & \text{if } k = m;\\ \tilde{\mathbf{W}}^{a(k+1)}_{L,j,:} \odot \boldsymbol{\Theta}^{zn(k)}_{j,:} & \text{if } k \in [m-1]; \end{cases}
$$

$$
\boldsymbol{\Lambda}^{zn(k)}_{\varphi,j,:} = \begin{cases} \mathbf{W}^{Fa}_{j,:} \odot \varphi^{zn(k)}_{j,:} & \text{if } k = m;\\ \tilde{\mathbf{W}}^{a(k+1)}_{U,j,:} \odot \varphi^{zn(k)}_{j,:} & \text{if } k \in [m-1]; \end{cases} \quad
\boldsymbol{\Omega}^{zn(k)}_{\psi,j,:} = \begin{cases} \mathbf{W}^{Fa}_{j,:} \odot \psi^{zn(k)}_{j,:} & \text{if } k = m;\\ \tilde{\mathbf{W}}^{a(k+1)}_{L,j,:} \odot \psi^{zn(k)}_{j,:} & \text{if } k \in [m-1]; \end{cases}
$$

$$
\boldsymbol{\Lambda}^{za(k)}_{\lambda,j,:} = \begin{cases} \mathbf{W}^{Fa}_{j,:} \odot \lambda^{za(k)}_{j,:} & \text{if } k = m;\\ \tilde{\mathbf{W}}^{a(k+1)}_{U,j,:} \odot \lambda^{za(k)}_{j,:} & \text{if } k \in [m-1]; \end{cases} \quad
\boldsymbol{\Omega}^{za(k)}_{\omega,j,:} = \begin{cases} \mathbf{W}^{Fa}_{j,:} \odot \omega^{za(k)}_{j,:} & \text{if } k = m;\\ \tilde{\mathbf{W}}^{a(k+1)}_{L,j,:} \odot \omega^{za(k)}_{j,:} & \text{if } k \in [m-1]; \end{cases}
$$

$$
\boldsymbol{\Lambda}^{za(k)}_{\Delta,j,:} = \begin{cases} \mathbf{W}^{Fa}_{j,:} \odot \boldsymbol{\Delta}^{za(k)}_{j,:} & \text{if } k = m;\\ \tilde{\mathbf{W}}^{a(k+1)}_{U,j,:} \odot \boldsymbol{\Delta}^{za(k)}_{j,:} & \text{if } k \in [m-1]; \end{cases} \quad
\boldsymbol{\Omega}^{za(k)}_{\Theta,j,:} = \begin{cases} \mathbf{W}^{Fa}_{j,:} \odot \boldsymbol{\Theta}^{za(k)}_{j,:} & \text{if } k = m;\\ \tilde{\mathbf{W}}^{a(k+1)}_{L,j,:} \odot \boldsymbol{\Theta}^{za(k)}_{j,:} & \text{if } k \in [m-1]; \end{cases}
$$

$$\mathbf{\Lambda}^{za(k)}_{\varphi,j,:} = \begin{cases} \mathbf{W}^{Fa}_{j,:} \odot \varphi^{za(k)}_{j,:} & \textit{if} \quad k = m; \\ \tilde{\mathbf{W}}^{a(k+1)}_{U,j,:} \odot \varphi^{za(k)}_{j,:} & \textit{if} \quad k \in [m-1]; \end{cases} \quad \mathbf{\Omega}^{za(k)}_{\psi,j,:} = \begin{cases} \mathbf{W}^{Fa}_{j,:} \odot \psi^{za(k)}_{j,:} & \textit{if} \quad k = m; \\ \tilde{\mathbf{W}}^{a(k+1)}_{L,j,:} \odot \psi^{za(k)}_{j,:} & \textit{if} \quad k \in [m-1]; \end{cases}$$

**3. define unified slopes and intercepts of cross terms of the reset gate and the hidden state;**

$$\lambda^{ra(k)}_{j,r} = \begin{cases} \alpha^{ra(k)}_{U,r} & \textit{if} \quad \mathbf{\Lambda}^{zn(k)}_{\Delta,j,r} \geq 0; \\ \alpha^{ra(k)}_{L,r} & \textit{if} \quad \mathbf{\Lambda}^{zn(k)}_{\Delta,j,r} < 0; \end{cases} \quad \omega^{ra(k)}_{j,r} = \begin{cases} \alpha^{ra(k)}_{L,r} & \textit{if} \quad \mathbf{\Omega}^{zn(k)}_{\Theta,j,r} \geq 0; \\ \alpha^{ra(k)}_{U,r} & \textit{if} \quad \mathbf{\Omega}^{zn(k)}_{\Theta,j,r} < 0; \end{cases}$$

$$\mathbf{\Delta}^{ra(k)}_{j,r} = \begin{cases} \beta^{ra(k)}_{U,r} & \textit{if} \quad \mathbf{\Lambda}^{zn(k)}_{\Delta,j,r} \geq 0; \\ \beta^{ra(k)}_{L,r} & \textit{if} \quad \mathbf{\Lambda}^{zn(k)}_{\Delta,j,r} < 0; \end{cases} \quad \mathbf{\Theta}^{ra(k)}_{j,r} = \begin{cases} \beta^{ra(k)}_{L,r} & \textit{if} \quad \mathbf{\Omega}^{zn(k)}_{\Theta,j,r} \geq 0; \\ \beta^{ra(k)}_{U,r} & \textit{if} \quad \mathbf{\Omega}^{zn(k)}_{\Theta,j,r} < 0; \end{cases}$$

$$\varphi^{ra(k)}_{j,r} = \begin{cases} \gamma^{ra(k)}_{U,r} & \textit{if} \quad \mathbf{\Lambda}^{zn(k)}_{\Delta,j,r} \geq 0; \\ \gamma^{ra(k)}_{L,r} & \textit{if} \quad \mathbf{\Lambda}^{zn(k)}_{\Delta,j,r} < 0; \end{cases} \quad \psi^{ra(k)}_{j,r} = \begin{cases} \gamma^{ra(k)}_{L,r} & \textit{if} \quad \mathbf{\Omega}^{zn(k)}_{\Theta,j,r} \geq 0; \\ \gamma^{ra(k)}_{U,r} & \textit{if} \quad \mathbf{\Omega}^{zn(k)}_{\Theta,j,r} < 0; \end{cases}$$

**4. collect coefficients in front of the reset gate *pre-activation* and the hidden state, and constants;**

$$\begin{aligned} \mathbf{\Lambda}^{ra(k)}_{\lambda,j,:} &= \mathbf{\Lambda}^{zn(k)}_{\Delta,j,:} \odot \lambda^{ra(k)}_{j,:} \quad \textit{if} \quad k \in [m]; & \mathbf{\Omega}^{ra(k)}_{\omega,j,:} &= \mathbf{\Omega}^{zn(k)}_{\Theta,j,:} \odot \omega^{ra(k)}_{j,:} \quad \textit{if} \quad k \in [m]; \\ \mathbf{\Lambda}^{ra(k)}_{\Delta,j,:} &= \mathbf{\Lambda}^{zn(k)}_{\Delta,j,:} \odot \mathbf{\Delta}^{ra(k)}_{j,:} \quad \textit{if} \quad k \in [m]; & \mathbf{\Omega}^{ra(k)}_{\Theta,j,:} &= \mathbf{\Omega}^{zn(k)}_{\Theta,j,:} \odot \mathbf{\Theta}^{ra(k)}_{j,:} \quad \textit{if} \quad k \in [m]; \\ \mathbf{\Lambda}^{ra(k)}_{\varphi,j,:} &= \mathbf{\Lambda}^{zn(k)}_{\Delta,j,:} \odot \varphi^{ra(k)}_{j,:} \quad \textit{if} \quad k \in [m]; & \mathbf{\Omega}^{ra(k)}_{\psi,j,:} &= \mathbf{\Omega}^{zn(k)}_{\Theta,j,:} \odot \psi^{ra(k)}_{j,:} \quad \textit{if} \quad k \in [m]; \end{aligned}$$

**5. define equivalent weight matrices and biases.**

$$\begin{aligned} \tilde{\mathbf{W}}^{x(k)}_{U,j,q_k} &= \mathbf{\Lambda}^{zn(k)}_{\lambda,j,:}\mathbf{W}^{zx}_{:,q_k} + \mathbf{\Lambda}^{za(k)}_{\lambda,j,:}\mathbf{W}^{zx}_{:,q_k} + \mathbf{\Lambda}^{zn(k)}_{\Delta,j,:}\mathbf{W}^{nx}_{:,q_k} + \mathbf{\Lambda}^{ra(k)}_{\lambda,j,:}\mathbf{W}^{rx}_{:,q_k}, \\ \tilde{\mathbf{W}}^{a(k)}_{U,j,r} &= \mathbf{\Lambda}^{zn(k)}_{\lambda,j,:}\mathbf{W}^{za}_{:,r} + \mathbf{\Lambda}^{za(k)}_{\lambda,j,:}\mathbf{W}^{za}_{:,r} + \mathbf{\Lambda}^{za(k)}_{\Delta,j,r} + \mathbf{\Lambda}^{ra(k)}_{\lambda,j,:}\mathbf{W}^{ra}_{:,r} + \mathbf{\Lambda}^{ra(k)}_{\Delta,j,:}\mathbf{W}^{na}_{:,r}, \\ \tilde{\mathbf{b}}^{(k)}_{U,j} &= \mathbf{\Lambda}^{zn(k)}_{\lambda,j,:}\mathbf{b}^{z} + \mathbf{\Lambda}^{za(k)}_{\lambda,j,:}\mathbf{b}^{z} + \mathbf{\Lambda}^{zn(k)}_{\Delta,j,:}\mathbf{b}^{nx} + \mathbf{\Lambda}^{ra(k)}_{\lambda,j,:}\mathbf{b}^{r} + \mathbf{\Lambda}^{ra(k)}_{\Delta,j,:}\mathbf{b}^{na} + \sum_{i=1}^{s}(\mathbf{\Lambda}^{zn(k)}_{\varphi,j,i} + \mathbf{\Lambda}^{za(k)}_{\varphi,j,i} + \mathbf{\Lambda}^{ra(k)}_{\varphi,j,i}), \\ \tilde{\mathbf{W}}^{x(k)}_{L,j,q_k} &= \mathbf{\Omega}^{zn(k)}_{\omega,j,:}\mathbf{W}^{zx}_{:,q_k} + \mathbf{\Omega}^{za(k)}_{\omega,j,:}\mathbf{W}^{zx}_{:,q_k} + \mathbf{\Omega}^{zn(k)}_{\Theta,j,:}\mathbf{W}^{nx}_{:,q_k} + \mathbf{\Omega}^{ra(k)}_{\omega,j,:}\mathbf{W}^{rx}_{:,q_k}, \\ \tilde{\mathbf{W}}^{a(k)}_{L,j,r} &= \mathbf{\Omega}^{zn(k)}_{\omega,j,:}\mathbf{W}^{za}_{:,r} + \mathbf{\Omega}^{za(k)}_{\omega,j,:}\mathbf{W}^{za}_{:,r} + \mathbf{\Omega}^{za(k)}_{\Theta,j,r} + \mathbf{\Omega}^{ra(k)}_{\omega,j,:}\mathbf{W}^{ra}_{:,r} + \mathbf{\Omega}^{ra(k)}_{\Theta,j,:}\mathbf{W}^{na}_{:,r}, \\ \tilde{\mathbf{b}}^{(k)}_{L,j} &= \mathbf{\Omega}^{zn(k)}_{\omega,j,:}\mathbf{b}^{z} + \mathbf{\Omega}^{za(k)}_{\omega,j,:}\mathbf{b}^{z} + \mathbf{\Omega}^{zn(k)}_{\Theta,j,:}\mathbf{b}^{nx} + \mathbf{\Omega}^{ra(k)}_{\omega,j,:}\mathbf{b}^{r} + \mathbf{\Omega}^{ra(k)}_{\Theta,j,:}\mathbf{b}^{na} + \sum_{i=1}^{s}(\mathbf{\Omega}^{zn(k)}_{\psi,j,i} + \mathbf{\Omega}^{za(k)}_{\psi,j,i} + \mathbf{\Omega}^{ra(k)}_{\psi,j,i}), \end{aligned}$$

**6. After looping steps 1 to 5 from $k = m$ to $k = 1$, the bounds are given by**

$$\begin{aligned} F^{U}_{j}(\mathbf{X}) &= \tilde{\mathbf{W}}^{a(1)}_{U,j,:}\mathbf{a}^{(0)} + \sum_{k=1}^{m}\tilde{\mathbf{W}}^{x(k)}_{U,j,:}\mathbf{x}^{(k)} + \sum_{k=1}^{m}\tilde{\mathbf{b}}^{(k)}_{U,j} + \mathbf{b}^{F}_{j}, \\ F^{L}_{j}(\mathbf{X}) &= \tilde{\mathbf{W}}^{a(1)}_{L,j,:}\mathbf{a}^{(0)} + \sum_{k=1}^{m}\tilde{\mathbf{W}}^{x(k)}_{L,j,:}\mathbf{x}^{(k)} + \sum_{k=1}^{m}\tilde{\mathbf{b}}^{(k)}_{L,j} + \mathbf{b}^{F}_{j}. \end{aligned}$$

***Proof 5*** *Given an $m$-layer gated recurrent unit network $F : \mathbb{R}^{n\times m} \to \mathbb{R}^{t}$ with pre-activation bounds $\mathbf{l}^{z(k)}$,$\mathbf{u}^{z(k)}$, $\mathbf{l}^{n(k)}$,$\mathbf{u}^{n(k)}$, $\mathbf{l}^{a(k)}$,$\mathbf{u}^{a(k)}$, $\mathbf{l}^{r(k)}$,$\mathbf{u}^{r(k)}$, $\mathbf{l}^{na(k)}$ and $\mathbf{u}^{na(k)}$ for $\mathbf{X} \in \mathbb{R}^{n\times m}$, where $\mathbf{x}^{(k)} \in \mathbb{B}_p(\mathbf{x}^{(k)}_0, \epsilon)$, let the pre-activation inputs for the $j$-th neuron at the output layer be $F_j(\mathbf{X}) = \mathbf{W}^{Fa}_{j,:}\mathbf{a}^{(m)} + \mathbf{b}^{F}_{j}$. The $j$-th output of the recurrent neural*

*network is the following:*

$$
\begin{aligned}
F_j(\mathbf{X}) &= \mathbf{W}^{Fa}_{j,:}\mathbf{a}^{(m)} + \mathbf{b}^F_j, \\
&= \sum_{i=1}^{s} \mathbf{W}^{Fa}_{j,i}\mathbf{a}^{(m)}_i + \mathbf{b}^F_j, \\
&= \sum_{i=1}^{s} \mathbf{W}^{Fa}_{j,i}[(1-\mathbf{z}^{(m)}_i)\mathbf{n}^{(m)}_i + \mathbf{z}^{(m)}_i\mathbf{a}^{(m-1)}_i] + \mathbf{b}^F_j, \\
&= \sum_{i=1}^{s} \mathbf{W}^{Fa}_{j,i}[(1-\sigma(\mathbf{y}^{z(m)}_i))\tanh(\mathbf{y}^{n(m)}_i) + \sigma(\mathbf{y}^{z(m)}_i)\mathbf{a}^{(m-1)}_i] + \mathbf{b}^F_j, \\
&= \sum_{\mathbf{W}^{Fa}_{j,i}\geq 0} \mathbf{W}^{Fa}_{j,i}[(1-\sigma(\mathbf{y}^{z(m)}_i))\tanh(\mathbf{y}^{n(m)}_i) + \sigma(\mathbf{y}^{z(m)}_i)\mathbf{a}^{(m-1)}_i] \\
&+ \sum_{\mathbf{W}^{Fa}_{j,i}< 0} \mathbf{W}^{Fa}_{j,i}[(1-\sigma(\mathbf{y}^{z(m)}_i))\tanh(\mathbf{y}^{n(m)}_i) + \sigma(\mathbf{y}^{z(m)}_i)\mathbf{a}^{(m-1)}_i] + \mathbf{b}^F_j.
\end{aligned}
\tag{29}
$$

*Assume the activation function* $(1-\sigma(\mathbf{y}))\tanh(\mathbf{x})$ *is bounded by two linear functions* $h^{zn(m)}_{L,i}(\mathbf{y},\mathbf{x})$, $h^{zn(m)}_{U,i}(\mathbf{y},\mathbf{x})$ *and* $\sigma(\mathbf{y})\mathbf{x}$ *is bounded by two linear functions* $h^{za(m)}_{L,i}(\mathbf{y},\mathbf{x})$, $h^{za(m)}_{U,i}(\mathbf{y},\mathbf{x})$, *we have*

$$
\begin{aligned}
h^{zn(m)}_{L,i}(\mathbf{y}^{z(m)}_i,\mathbf{y}^{n(m)}_i) \leq (1-\sigma(\mathbf{y}^{z(m)}_i))\tanh(\mathbf{y}^{n(m)}_i) \leq h^{zn(m)}_{U,i}(\mathbf{y}^{z(m)}_i,\mathbf{y}^{n(m)}_i), \\
h^{za(m)}_{L,i}(\mathbf{y}^{z(m)}_i,\mathbf{a}^{(m-1)}_i) \leq \sigma(\mathbf{y}^{z(m)}_i)\mathbf{a}^{(m-1)}_i \leq h^{za(m)}_{U,i}(\mathbf{y}^{z(m)}_i,\mathbf{a}^{(m-1)}_i).
\end{aligned}
$$

***Upper bound.*** *We can then obtain*

$$
\begin{aligned}
F_j(\mathbf{X}) \leq & \sum_{\mathbf{W}^{Fa}_{j,i}\geq 0} \mathbf{W}^{Fa}_{j,i}\ (\alpha^{zn(m)}_{U,i}\mathbf{y}^{z(m)}_i + \beta^{zn(m)}_{U,i}\mathbf{y}^{n(m)}_i + \gamma^{zn(m)}_{U,i} \\
& + \alpha^{za(m)}_{U,i}\mathbf{y}^{z(m)}_i + \beta^{za(m)}_{U,i}\mathbf{a}^{(m-1)}_i + \gamma^{za(m)}_{U,i}) \\
& + \sum_{\mathbf{W}^{Fa}_{j,i}< 0} \mathbf{W}^{fa}_{j,i}\ (\alpha^{zn(m)}_{L,i}\mathbf{y}^{z(m)}_i + \beta^{zn(m)}_{L,i}\mathbf{y}^{n(m)}_i + \gamma^{zn(m)}_{L,i} \\
& + \alpha^{za(m)}_{L,i}\mathbf{y}^{z(m)}_i + \beta^{za(m)}_{L,i}\mathbf{a}^{(m-1)}_i + \gamma^{za(m)}_{L,i}) + \mathbf{b}^F_j.
\end{aligned}
$$

*We then define* $\lambda^{zn(m)}_{j,i}$, $\mathbf{\Delta}^{zn(m)}_{j,i}$, $\varphi^{zn(m)}_{j,i}$, $\lambda^{za(m)}_{j,i}$, $\mathbf{\Delta}^{za(m)}_{j,i}$ *and* $\varphi^{za(m)}_{j,i}$ *in the parentheses:*

$$
\lambda^{zn(m)}_{j,i} = \begin{cases} \alpha^{zn(m)}_{U,i} & \text{if } \mathbf{W}^{Fa}_{j,i} \geq 0; \\ \alpha^{zn(m)}_{L,i} & \text{if } \mathbf{W}^{Fa}_{j,i} < 0; \end{cases} \quad \lambda^{za(m)}_{j,i} = \begin{cases} \alpha^{za(m)}_{U,i} & \text{if } \mathbf{W}^{Fa}_{j,i} \geq 0; \\ \alpha^{za(m)}_{L,i} & \text{if } \mathbf{W}^{Fa}_{j,i} < 0; \end{cases}
$$

$$
\mathbf{\Delta}^{zn(m)}_{j,i} = \begin{cases} \beta^{zn(m)}_{U,i} & \text{if } \mathbf{W}^{Fa}_{j,i} \geq 0; \\ \beta^{zn(m)}_{L,i} & \text{if } \mathbf{W}^{Fa}_{j,i} < 0; \end{cases} \quad \mathbf{\Delta}^{za(m)}_{j,i} = \begin{cases} \beta^{za(m)}_{U,i} & \text{if } \mathbf{W}^{Fa}_{j,i} \geq 0; \\ \beta^{za(m)}_{L,i} & \text{if } \mathbf{W}^{Fa}_{j,i} < 0; \end{cases}
$$

$$
\varphi^{zn(m)}_{j,i} = \begin{cases} \gamma^{zn(m)}_{U,i} & \text{if } \mathbf{W}^{Fa}_{j,i} \geq 0; \\ \gamma^{zn(m)}_{L,i} & \text{if } \mathbf{W}^{Fa}_{j,i} < 0; \end{cases} \quad \varphi^{za(m)}_{j,i} = \begin{cases} \gamma^{za(m)}_{U,i} & \text{if } \mathbf{W}^{Fa}_{j,i} \geq 0; \\ \gamma^{za(m)}_{L,i} & \text{if } \mathbf{W}^{Fa}_{j,i} < 0; \end{cases}
$$

*and obtain*

$$
\begin{aligned}
F_j(\mathbf{X}) \leq \sum_{i=1}^{s} \mathbf{W}^{Fa}_{j,i}\ (\lambda^{zn(m)}_{j,i}\mathbf{y}^{z(m)}_i + \mathbf{\Delta}^{zn(m)}_{j,i}\mathbf{y}^{n(m)}_i + \varphi^{zn(m)}_{j,i} \\
+ \lambda^{za(m)}_{j,i}\mathbf{y}^{z(m)}_i + \mathbf{\Delta}^{za(m)}_{j,i}\mathbf{a}^{(m-1)}_i + \varphi^{za(m)}_{j,i}) + \mathbf{b}^F_j.
\end{aligned}
$$

*We further let*

$$
\begin{aligned}
\mathbf{\Lambda}^{zn(m)}_{\lambda,j,i} := \mathbf{W}^{Fa}_{j,i}\ \lambda^{zn(m)}_{j,i}, \mathbf{\Lambda}^{zn(m)}_{\Delta,j,i} := \mathbf{W}^{Fa}_{j,i}\ \mathbf{\Delta}^{zn(m)}_{j,i}, \mathbf{\Lambda}^{zn(m)}_{\varphi,j,i} := \mathbf{W}^{Fa}_{j,i}\ \varphi^{zn(m)}_{j,i}, \\
\mathbf{\Lambda}^{za(m)}_{\lambda,j,i} := \mathbf{W}^{Fa}_{j,i}\ \lambda^{za(m)}_{j,i}, \mathbf{\Lambda}^{za(m)}_{\Delta,j,i} := \mathbf{W}^{Fa}_{j,i}\ \mathbf{\Delta}^{za(m)}_{j,i}, \mathbf{\Lambda}^{za(m)}_{\varphi,j,i} := \mathbf{W}^{Fa}_{j,i}\ \varphi^{za(m)}_{j,i},
\end{aligned}
$$

*and we have*

$$\begin{aligned}
F_j(\mathbf{X}) \leq & \sum_{i=1}^{s}(\mathbf{\Lambda}^{zn(m)}_{\lambda,j,i}\mathbf{y}^{z(m)}_i + \mathbf{\Lambda}^{zn(m)}_{\Delta,j,i}\mathbf{y}^{n(m)}_i + \mathbf{\Lambda}^{zn(m)}_{\varphi,j,i} + \mathbf{\Lambda}^{za(m)}_{\lambda,j,i}\mathbf{y}^{z(m)}_i + \mathbf{\Lambda}^{za(m)}_{\Delta,j,i}\mathbf{a}^{(m-1)}_i + \mathbf{\Lambda}^{za(m)}_{\varphi,j,i}) + \mathbf{b}^F_j, \\
= & \sum_{i=1}^{s}[(\mathbf{\Lambda}^{zn(m)}_{\lambda,j,i} + \mathbf{\Lambda}^{za(m)}_{\lambda,j,i})(\mathbf{W}^{zx}_{i,:}\mathbf{x}^{(m)} + \mathbf{W}^{za}_{i,:}\mathbf{a}^{(m-1)} + \mathbf{b}^z_i) + \mathbf{\Lambda}^{zn(m)}_{\Delta,j,i}(\mathbf{W}^{nx}_{i,:}\mathbf{x}^{(m)} + \mathbf{b}^{nx}_i \\
& + \mathbf{r}^{(m)}_i(\mathbf{W}^{na}_{i,:}\mathbf{a}^{(m-1)} + \mathbf{b}^{na}_i)) + \mathbf{\Lambda}^{zn(m)}_{\varphi,j,i} + \mathbf{\Lambda}^{za(m)}_{\varphi,j,i} + \mathbf{\Lambda}^{za(m)}_{\Delta,j,i}\mathbf{a}^{(m-1)}_i] + \mathbf{b}^F_j, \\
= & \sum_{q_m=1}^{n}(\sum_{i=1}^{s}(\mathbf{\Lambda}^{zn(m)}_{\lambda,j,i} + \mathbf{\Lambda}^{za(m)}_{\lambda,j,i})\mathbf{W}^{zx}_{i,q_m} + \sum_{i=1}^{s}\mathbf{\Lambda}^{zn(m)}_{\Delta,j,i}\mathbf{W}^{nx}_{i,q_m})\mathbf{x}^{(m)}_{q_m} \\
& + \sum_{r=1}^{s}(\sum_{i=1}^{s}(\mathbf{\Lambda}^{zn(m)}_{\lambda,j,i} + \mathbf{\Lambda}^{za(m)}_{\lambda,j,i})\mathbf{W}^{za}_{i,r} + \mathbf{\Lambda}^{za(m)}_{\Delta,j,r})\mathbf{a}^{(m-1)}_r \\
& + \sum_{i=1}^{s}\mathbf{\Lambda}^{zn(m)}_{\lambda,j,i}\mathbf{b}^z_i + \sum_{i=1}^{s}\mathbf{\Lambda}^{za(m)}_{\lambda,j,i}\mathbf{b}^z_i + \sum_{i=1}^{s}\mathbf{\Lambda}^{zn(m)}_{\Delta,j,i}\mathbf{b}^{nx}_i + \sum_{i=1}^{s}(\mathbf{\Lambda}^{zn(m)}_{\varphi,j,i} + \mathbf{\Lambda}^{za(m)}_{\varphi,j,i}) \\
& + \sum_{i=1}^{s}\mathbf{\Lambda}^{zn(m)}_{\Delta,j,i}(\sigma(\mathbf{y}^{r(m)}_i)(\mathbf{W}^{na}_{i,:}\mathbf{a}^{(m-1)} + \mathbf{b}^{na}_i)) + \mathbf{b}^F_j.
\end{aligned}$$

*Assume the activation function $\sigma(\mathbf{y})\mathbf{x}$ is bounded by two linear functions $h^{ra(m)}_{L,i}(\mathbf{y},\mathbf{x})$, $h^{ra(m)}_{U,i}(\mathbf{y},\mathbf{x})$, we have*

$$h^{ra(m)}_{L,i}(\mathbf{y}^{r(m)}_i, \mathbf{W}^{na}_{i,:}\mathbf{a}^{(m-1)} + \mathbf{b}^{na}_i) \leq \sigma(\mathbf{y}^{r(m)}_i)(\mathbf{W}^{na}_{i,:}\mathbf{a}^{(m-1)} + \mathbf{b}^{na}_i) \leq h^{ra(m)}_{U,i}(\mathbf{y}^{r(m)}_i, \mathbf{W}^{na}_{i,:}\mathbf{a}^{(m-1)} + \mathbf{b}^{na}_i).$$

*We then have*

$$\begin{aligned}
F_j(\mathbf{X}) \leq & \sum_{q_m=1}^{n}((\mathbf{\Lambda}^{zn(m)}_{\lambda,j,:} + \mathbf{\Lambda}^{za(m)}_{\lambda,j,:})\mathbf{W}^{zx}_{:,q_m} + \mathbf{\Lambda}^{zn(m)}_{\Delta,j,:}\mathbf{W}^{nx}_{:,q_m})\mathbf{x}^{(m)}_{q_m} \\
& + \sum_{r=1}^{s}((\mathbf{\Lambda}^{zn(m)}_{\lambda,j,:} + \mathbf{\Lambda}^{za(m)}_{\lambda,j,:})\mathbf{W}^{za}_{:,r} + \mathbf{\Lambda}^{za(m)}_{\Delta,j,r})\mathbf{a}^{(m-1)}_r \\
& + \mathbf{\Lambda}^{zn(m)}_{\lambda,j,:}\mathbf{b}^z + \mathbf{\Lambda}^{za(m)}_{\lambda,j,:}\mathbf{b}^z + \mathbf{\Lambda}^{zn(m)}_{\Delta,j,:}\mathbf{b}^{nx} + \sum_{i=1}^{s}(\mathbf{\Lambda}^{zn(m)}_{\varphi,j,i} + \mathbf{\Lambda}^{za(m)}_{\varphi,j,i}) \\
& + \sum_{\mathbf{\Lambda}^{zn(m)}_{\Delta,j,i}\geq 0}\mathbf{\Lambda}^{zn(m)}_{\Delta,j,i}[\alpha^{ra(m)}_{U,i}\mathbf{y}^{r(m)}_i + \beta^{ra(m)}_{U,i}(\mathbf{W}^{na}_{i,:}\mathbf{a}^{(m-1)} + \mathbf{b}^{na}_i) + \gamma^{ra(m)}_{U,i}] \\
& + \sum_{\mathbf{\Lambda}^{zn(m)}_{\Delta,j,i}< 0}\mathbf{\Lambda}^{zn(m)}_{\Delta,j,i}[\alpha^{ra(m)}_{L,i}\mathbf{y}^{r(m)}_i + \beta^{ra(m)}_{L,i}(\mathbf{W}^{na}_{i,:}\mathbf{a}^{(m-1)} + \mathbf{b}^{na}_i) + \gamma^{ra(m)}_{L,i}] + \mathbf{b}^F_j.
\end{aligned}$$

*We then define $\lambda^{ra(m)}_{j,i}$, $\mathbf{\Delta}^{ra(m)}_{j,i}$, $\varphi^{ra(m)}_{j,i}$, $\mathbf{\Lambda}^{ra(m)}_{\lambda,j,i}$, $\mathbf{\Lambda}^{ra(m)}_{\Delta,j,i}$ and $\mathbf{\Lambda}^{ra(m)}_{\varphi,j,i}$ in the parentheses:*

$$\lambda^{ra(m)}_{j,i} = \begin{cases} \alpha^{ra(m)}_{U,i} & \textit{if } \mathbf{\Lambda}^{zn(m)}_{\Delta,j,i} \geq 0; \\ \alpha^{ra(m)}_{L,i} & \textit{if } \mathbf{\Lambda}^{zn(m)}_{\Delta,j,i} < 0; \end{cases} \quad \mathbf{\Lambda}^{ra(m)}_{\lambda,j,i} := \mathbf{\Lambda}^{zn(m)}_{\Delta,j,i}\ \lambda^{ra(m)}_{j,i};$$

$$\mathbf{\Delta}^{ra(m)}_{j,i} = \begin{cases} \beta^{ra(m)}_{U,i} & \textit{if } \mathbf{\Lambda}^{zn(m)}_{\Delta,j,i} \geq 0; \\ \beta^{ra(m)}_{L,i} & \textit{if } \mathbf{\Lambda}^{zn(m)}_{\Delta,j,i} < 0; \end{cases} \quad \mathbf{\Lambda}^{ra(m)}_{\Delta,j,i} := \mathbf{\Lambda}^{zn(m)}_{\Delta,j,i}\ \mathbf{\Delta}^{ra(m)}_{j,i};$$

$$\varphi^{ra(m)}_{j,i} = \begin{cases} \gamma^{ra(m)}_{U,i} & \textit{if } \mathbf{\Lambda}^{zn(m)}_{\Delta,j,i} \geq 0; \\ \gamma^{ra(m)}_{L,i} & \textit{if } \mathbf{\Lambda}^{zn(m)}_{\Delta,j,i} < 0; \end{cases} \quad \mathbf{\Lambda}^{ra(m)}_{\varphi,j,i} := \mathbf{\Lambda}^{zn(m)}_{\Delta,j,i}\ \varphi^{ra(m)}_{j,i};$$

*and obtain*

$$
\begin{aligned}
F_j(\mathbf{X}) \leq & \sum_{q_m=1}^{n}((\mathbf{\Lambda}^{zn(m)}_{\lambda,j,:}+\mathbf{\Lambda}^{za(m)}_{\lambda,j,:})\mathbf{W}^{zx}_{:,q_m}+\mathbf{\Lambda}^{zn(m)}_{\Delta,j,:}\mathbf{W}^{nx}_{:,q_m})\mathbf{x}^{(m)}_{q_m} \\
&+\sum_{r=1}^{s}((\mathbf{\Lambda}^{zn(m)}_{\lambda,j,:}+\mathbf{\Lambda}^{za(m)}_{\lambda,j,:})\mathbf{W}^{za}_{:,r}+\mathbf{\Lambda}^{za(m)}_{\Delta,j,r})\mathbf{a}^{(m-1)}_{r} \\
&+\mathbf{\Lambda}^{zn(m)}_{\lambda,j,:}\mathbf{b}^{z}+\mathbf{\Lambda}^{za(m)}_{\lambda,j,:}\mathbf{b}^{z}+\mathbf{\Lambda}^{zn(m)}_{\Delta,j,:}\mathbf{b}^{nx}+\sum_{i=1}^{s}(\mathbf{\Lambda}^{zn(m)}_{\varphi,j,i}+\mathbf{\Lambda}^{za(m)}_{\varphi,j,i}) \\
&+\sum_{i=1}^{s}[\mathbf{\Lambda}^{ra(m)}_{\lambda,j,i}\mathbf{y}^{r(m)}_{i}+\mathbf{\Lambda}^{ra(m)}_{\Delta,j,i}(\mathbf{W}^{na}_{i,:}\mathbf{a}^{(m-1)}+\mathbf{b}^{na}_{i})+\mathbf{\Lambda}^{ra(m)}_{\varphi,j,i}]+\mathbf{b}^{F}_{j} \\
&=\sum_{q_m=1}^{n}((\mathbf{\Lambda}^{zn(m)}_{\lambda,j,:}+\mathbf{\Lambda}^{za(m)}_{\lambda,j,:})\mathbf{W}^{zx}_{:,q_m}+\mathbf{\Lambda}^{zn(m)}_{\Delta,j,:}\mathbf{W}^{nx}_{:,q_m})\mathbf{x}^{(m)}_{q_m} \\
&+\sum_{r=1}^{s}((\mathbf{\Lambda}^{zn(m)}_{\lambda,j,:}+\mathbf{\Lambda}^{za(m)}_{\lambda,j,:})\mathbf{W}^{za}_{:,r}+\mathbf{\Lambda}^{za(m)}_{\Delta,j,r})\mathbf{a}^{(m-1)}_{r} \\
&+\mathbf{\Lambda}^{zn(m)}_{\lambda,j,:}\mathbf{b}^{z}+\mathbf{\Lambda}^{za(m)}_{\lambda,j,:}\mathbf{b}^{z}+\mathbf{\Lambda}^{zn(m)}_{\Delta,j,:}\mathbf{b}^{nx}+\sum_{i=1}^{s}(\mathbf{\Lambda}^{zn(m)}_{\varphi,j,i}+\mathbf{\Lambda}^{za(m)}_{\varphi,j,i}) \\
&+\sum_{i=1}^{s}\mathbf{\Lambda}^{ra(m)}_{\lambda,j,i}(\mathbf{W}^{rx}_{i,:}\mathbf{x}^{(m)}+\mathbf{W}^{ra}_{i,:}\mathbf{a}^{(m-1)}+\mathbf{b}^{r}_{i})+\sum_{i=1}^{s}\mathbf{\Lambda}^{ra(m)}_{\Delta,j,i}(\mathbf{W}^{na}_{i,:}\mathbf{a}^{(m-1)}+\mathbf{b}^{na}_{i})+\sum_{i=1}^{s}\mathbf{\Lambda}^{ra(m)}_{\varphi,j,i}+\mathbf{b}^{F}_{j} \\
&=\sum_{q_m=1}^{n}((\mathbf{\Lambda}^{zn(m)}_{\lambda,j,:}+\mathbf{\Lambda}^{za(m)}_{\lambda,j,:})\mathbf{W}^{zx}_{:,q_m}+\mathbf{\Lambda}^{zn(m)}_{\Delta,j,:}\mathbf{W}^{nx}_{:,q_m})\mathbf{x}^{(m)}_{q_m} \\
&+\sum_{r=1}^{s}((\mathbf{\Lambda}^{zn(m)}_{\lambda,j,:}+\mathbf{\Lambda}^{za(m)}_{\lambda,j,:})\mathbf{W}^{za}_{:,r}+\mathbf{\Lambda}^{za(m)}_{\Delta,j,r})\mathbf{a}^{(m-1)}_{r} \\
&+\mathbf{\Lambda}^{zn(m)}_{\lambda,j,:}\mathbf{b}^{z}+\mathbf{\Lambda}^{za(m)}_{\lambda,j,:}\mathbf{b}^{z}+\mathbf{\Lambda}^{zn(m)}_{\Delta,j,:}\mathbf{b}^{nx}+\sum_{i=1}^{s}(\mathbf{\Lambda}^{zn(m)}_{\varphi,j,i}+\mathbf{\Lambda}^{za(m)}_{\varphi,j,i}) \\
&+\sum_{q_m=1}^{n}(\sum_{i=1}^{s}\mathbf{\Lambda}^{ra(m)}_{\lambda,j,i}\mathbf{W}^{rx}_{i,q_m})\mathbf{x}^{(m)}_{q_m}+\sum_{r=1}^{s}(\sum_{i=1}^{s}\mathbf{\Lambda}^{ra(m)}_{\lambda,j,i}\mathbf{W}^{ra}_{i,r})\mathbf{a}^{(m-1)}_{r}+\sum_{i=1}^{s}\mathbf{\Lambda}^{ra(m)}_{\lambda,j,i}\mathbf{b}^{r}_{i} \\
&+\sum_{r=1}^{s}(\sum_{i=1}^{s}\mathbf{\Lambda}^{ra(m)}_{\Delta,j,i}\mathbf{W}^{na}_{i,r})\mathbf{a}^{(m-1)}_{r}+\sum_{i=1}^{s}\mathbf{\Lambda}^{ra(m)}_{\Delta,j,i}\mathbf{b}^{na}_{i}+\sum_{i=1}^{s}\mathbf{\Lambda}^{ra(m)}_{\varphi,j,i}+\mathbf{b}^{F}_{j} \\
&=\sum_{q_m=1}^{n}((\mathbf{\Lambda}^{zn(m)}_{\lambda,j,:}+\mathbf{\Lambda}^{za(m)}_{\lambda,j,:})\mathbf{W}^{zx}_{:,q_m}+\mathbf{\Lambda}^{zn(m)}_{\Delta,j,:}\mathbf{W}^{nx}_{:,q_m}+\mathbf{\Lambda}^{ra(m)}_{\lambda,j,:}\mathbf{W}^{rx}_{:,q_m})\mathbf{x}^{(m)}_{q_m} \\
&+\sum_{r=1}^{s}((\mathbf{\Lambda}^{zn(m)}_{\lambda,j,:}+\mathbf{\Lambda}^{za(m)}_{\lambda,j,:})\mathbf{W}^{za}_{:,r}+\mathbf{\Lambda}^{za(m)}_{\Delta,j,r}+\mathbf{\Lambda}^{ra(m)}_{\lambda,j,:}\mathbf{W}^{ra}_{:,r}+\mathbf{\Lambda}^{ra(m)}_{\Delta,j,:}\mathbf{W}^{na}_{:,r})\mathbf{a}^{(m-1)}_{r} \\
&+\mathbf{\Lambda}^{zn(m)}_{\lambda,j,:}\mathbf{b}^{z}+\mathbf{\Lambda}^{za(m)}_{\lambda,j,:}\mathbf{b}^{z}+\mathbf{\Lambda}^{zn(m)}_{\Delta,j,:}\mathbf{b}^{nx}+\mathbf{\Lambda}^{ra(m)}_{\lambda,j,:}\mathbf{b}^{r}+\mathbf{\Lambda}^{ra(m)}_{\Delta,j,:}\mathbf{b}^{na}+\sum_{i=1}^{s}(\mathbf{\Lambda}^{zn(m)}_{\varphi,j,i}+\mathbf{\Lambda}^{za(m)}_{\varphi,j,i}+\mathbf{\Lambda}^{ra(m)}_{\varphi,j,i}) \\
&+\mathbf{b}^{F}_{j}. \qquad (30)
\end{aligned}
$$

*We combine coefficients in Equation* (30) *into equivalent weights* $\tilde{\mathbf{W}}^{x(m)}_{U,j,q_m}$, $\tilde{\mathbf{W}}^{a(m)}_{U,j,r}$ *and bias* $\tilde{\mathbf{b}}^{(m)}_{U,j}$ *as defined by*

$$
\begin{aligned}
\tilde{\mathbf{W}}^{x(m)}_{U,j,q_m} &= \mathbf{\Lambda}^{zn(m)}_{\lambda,j,:}\mathbf{W}^{zx}_{:,q_m}+\mathbf{\Lambda}^{za(m)}_{\lambda,j,:}\mathbf{W}^{zx}_{:,q_k}+\mathbf{\Lambda}^{zn(m)}_{\Delta,j,:}\mathbf{W}^{nx}_{:,q_m}+\mathbf{\Lambda}^{ra(m)}_{\lambda,j,:}\mathbf{W}^{rx}_{:,q_m}, \\
\tilde{\mathbf{W}}^{a(m)}_{U,j,r} &= \mathbf{\Lambda}^{zn(m)}_{\lambda,j,:}\mathbf{W}^{za}_{:,r}+\mathbf{\Lambda}^{za(m)}_{\lambda,j,:}\mathbf{W}^{za}_{:,r}+\mathbf{\Lambda}^{za(m)}_{\Delta,j,r}+\mathbf{\Lambda}^{ra(m)}_{\lambda,j,:}\mathbf{W}^{ra}_{:,r}+\mathbf{\Lambda}^{ra(m)}_{\Delta,j,:}\mathbf{W}^{na}_{:,r},
\end{aligned}
$$

$$\tilde{\mathbf{b}}_{U,j}^{(m)} = \mathbf{\Lambda}_{\lambda,j,:}^{zn(m)}\mathbf{b}^z + \mathbf{\Lambda}_{\lambda,j,:}^{za(m)}\mathbf{b}^z + \mathbf{\Lambda}_{\Delta,j,:}^{zn(m)}\mathbf{b}^{nx} + \mathbf{\Lambda}_{\lambda,j,:}^{ra(m)}\mathbf{b}^r + \mathbf{\Lambda}_{\Delta,j,:}^{ra(m)}\mathbf{b}^{na} + \sum_{i=1}^{s}(\mathbf{\Lambda}_{\varphi,j,i}^{zn(m)} + \mathbf{\Lambda}_{\varphi,j,i}^{za(m)} + \mathbf{\Lambda}_{\varphi,j,i}^{ra(m)}),$$

*and obtain*

$$F_j(\mathbf{X}) \leq F_j^{U,m}(\mathbf{X}) = \tilde{\mathbf{W}}_{U,j,:}^{x(m)}\mathbf{x}^{(m)} + \tilde{\mathbf{W}}_{U,j,:}^{a(m)}\mathbf{a}^{(m-1)} + \tilde{\mathbf{b}}_{U,j}^{(m)} + \mathbf{b}_j^F. \tag{31}$$

*Notice that Equation* (29) *and Equation* (31) *are in similar forms. Thus,* $\forall r \in s$ *we can define variables as follows:*

$$\lambda_{j,r}^{zn(m-1)} = \begin{cases} \alpha_{U,r}^{zn(m-1)} & \text{if } \tilde{\mathbf{W}}_{U,j,r}^{a(m)} \geq 0; \\ \alpha_{L,r}^{zn(m-1)} & \text{if } \tilde{\mathbf{W}}_{U,j,r}^{a(m)} < 0; \end{cases} \quad \lambda_{j,r}^{za(m-1)} = \begin{cases} \alpha_{U,r}^{za(m-1)} & \text{if } \tilde{\mathbf{W}}_{U,j,r}^{a(m)} \geq 0; \\ \alpha_{L,r}^{za(m-1)} & \text{if } \tilde{\mathbf{W}}_{U,j,r}^{a(m)} < 0; \end{cases}$$

$$\mathbf{\Delta}_{j,r}^{zn(m-1)} = \begin{cases} \beta_{U,r}^{zn(m-1)} & \text{if } \tilde{\mathbf{W}}_{U,j,r}^{a(m)} \geq 0; \\ \beta_{L,r}^{zn(m-1)} & \text{if } \tilde{\mathbf{W}}_{U,j,r}^{a(m)} < 0; \end{cases} \quad \mathbf{\Delta}_{j,r}^{za(m-1)} = \begin{cases} \beta_{U,r}^{za(m-1)} & \text{if } \tilde{\mathbf{W}}_{U,j,r}^{a(m)} \geq 0; \\ \beta_{L,r}^{za(m-1)} & \text{if } \tilde{\mathbf{W}}_{U,j,r}^{a(m)} < 0; \end{cases}$$

$$\varphi_{j,r}^{zn(m-1)} = \begin{cases} \gamma_{U,r}^{zn(m-1)} & \text{if } \tilde{\mathbf{W}}_{U,j,r}^{a(m)} \geq 0; \\ \gamma_{L,r}^{zn(m-1)} & \text{if } \tilde{\mathbf{W}}_{U,j,r}^{a(m)} < 0; \end{cases} \quad \varphi_{j,r}^{za(m-1)} = \begin{cases} \gamma_{U,r}^{za(m-1)} & \text{if } \tilde{\mathbf{W}}_{U,j,r}^{a(m)} \geq 0; \\ \gamma_{L,r}^{za(m-1)} & \text{if } \tilde{\mathbf{W}}_{U,j,r}^{a(m)} < 0; \end{cases}$$

$$\mathbf{\Lambda}_{\lambda,j,:}^{zn(m-1)} = \tilde{\mathbf{W}}_{U,j,:}^{a(m)} \odot \lambda_{j,:}^{zn(m-1)}; \quad \mathbf{\Lambda}_{\lambda,j,:}^{za(m-1)} = \tilde{\mathbf{W}}_{U,j,:}^{a(m)} \odot \lambda_{j,:}^{za(m-1)};$$

$$\mathbf{\Lambda}_{\Delta,j,:}^{zn(m-1)} = \tilde{\mathbf{W}}_{U,j,:}^{a(m)} \odot \mathbf{\Delta}_{j,:}^{zn(m-1)}; \quad \mathbf{\Lambda}_{\Delta,j,:}^{za(m-1)} = \tilde{\mathbf{W}}_{U,j,:}^{a(m)} \odot \mathbf{\Delta}_{j,:}^{za(m-1)};$$

$$\mathbf{\Lambda}_{\varphi,j,:}^{zn(m-1)} = \tilde{\mathbf{W}}_{U,j,:}^{a(m)} \odot \varphi_{j,:}^{zn(m-1)}; \quad \mathbf{\Lambda}_{\varphi,j,:}^{za(m-1)} = \tilde{\mathbf{W}}_{U,j,:}^{a(m)} \odot \varphi_{j,:}^{za(m-1)};$$

$$\lambda_{j,r}^{ra(m-1)} = \begin{cases} \alpha_{U,r}^{ra(m-1)} & \text{if } \mathbf{\Lambda}_{\Delta,j,r}^{zn(m-1)} \geq 0; \\ \alpha_{L,r}^{ra(m-1)} & \text{if } \mathbf{\Lambda}_{\Delta,j,r}^{zn(m-1)} < 0; \end{cases} \quad \mathbf{\Lambda}_{\lambda,j,:}^{ra(m-1)} = \mathbf{\Lambda}_{\Delta,j,:}^{zn(m-1)} \odot \lambda_{j,:}^{ra(m-1)};$$

$$\mathbf{\Delta}_{j,r}^{ra(m-1)} = \begin{cases} \beta_{U,r}^{ra(m-1)} & \text{if } \mathbf{\Lambda}_{\Delta,j,r}^{zn(m-1)} \geq 0; \\ \beta_{L,r}^{ra(m-1)} & \text{if } \mathbf{\Lambda}_{\Delta,j,r}^{zn(m-1)} < 0; \end{cases} \quad \mathbf{\Lambda}_{\Delta,j,:}^{ra(m-1)} = \mathbf{\Lambda}_{\Delta,j,:}^{zn(m-1)} \odot \mathbf{\Delta}_{j,:}^{ra(m-1)};$$

$$\varphi_{j,r}^{ra(m-1)} = \begin{cases} \gamma_{U,r}^{ra(m-1)} & \text{if } \mathbf{\Lambda}_{\Delta,j,r}^{zn(m-1)} \geq 0; \\ \gamma_{L,r}^{ra(m-1)} & \text{if } \mathbf{\Lambda}_{\Delta,j,r}^{zn(m-1)} < 0; \end{cases} \quad \mathbf{\Lambda}_{\varphi,j,:}^{ra(m-1)} = \mathbf{\Lambda}_{\Delta,j,:}^{zn(m-1)} \odot \varphi_{j,:}^{ra(m-1)}.$$

*Then we have*

$$F_j^{U,m}(\mathbf{X}) \leq F_j^{U,m-1}(\mathbf{X}) = \tilde{\mathbf{W}}_{U,j,:}^{x(m)}\mathbf{x}^{(m)} + \tilde{\mathbf{W}}_{U,j,:}^{x(m-1)}\mathbf{x}^{(m-1)} + \tilde{\mathbf{W}}_{U,j,:}^{a(m-1)}\mathbf{a}^{(m-2)} + \tilde{\mathbf{b}}_{U,j}^{(m)} + \tilde{\mathbf{b}}_{U,j}^{(m-1)} + \mathbf{b}_j^F.$$

*Thus, we can repeat the above procedure iteratively until we obtain the final upper bound* $F_j^{U,1}(\mathbf{X})$*, where* $F_j(\mathbf{X}) \leq F_j^{U,m}(\mathbf{X}) \leq \cdots \leq F_j^{U,1}(\mathbf{X})$*. We let* $F_j^U(\mathbf{X})$ *denote the final upper bound* $F_j^{U,1}(\mathbf{X})$*, and we have*

$$F_j^U(\mathbf{X}) = \tilde{\mathbf{W}}_{U,j,:}^{a(1)}\mathbf{a}^{(0)} + \sum_{k=1}^{m}\tilde{\mathbf{W}}_{U,j,:}^{x(k)}\mathbf{x}^{(k)} + \sum_{k=1}^{m}\tilde{\mathbf{b}}_{U,j}^{(k)} + \mathbf{b}_j^F,$$

*where*

$$\tilde{\mathbf{W}}_{U,j,q_k}^{x(k)} = \mathbf{\Lambda}_{\lambda,j,:}^{zn(k)}\mathbf{W}_{:,q_k}^{zx} + \mathbf{\Lambda}_{\lambda,j,:}^{za(k)}\mathbf{W}_{:,q_k}^{zx} + \mathbf{\Lambda}_{\Delta,j,:}^{zn(k)}\mathbf{W}_{:,q_k}^{nx} + \mathbf{\Lambda}_{\lambda,j,:}^{ra(k)}\mathbf{W}_{:,q_k}^{rx},$$

$$\tilde{\mathbf{W}}_{U,j,r}^{a(k)} = \mathbf{\Lambda}_{\lambda,j,:}^{zn(k)}\mathbf{W}_{:,r}^{za} + \mathbf{\Lambda}_{\lambda,j,:}^{za(k)}\mathbf{W}_{:,r}^{za} + \mathbf{\Lambda}_{\Delta,j,r}^{za(k)} + \mathbf{\Lambda}_{\lambda,j,:}^{ra(k)}\mathbf{W}_{:,r}^{ra} + \mathbf{\Lambda}_{\Delta,j,:}^{ra(k)}\mathbf{W}_{:,r}^{na},$$

$$\tilde{\mathbf{b}}_{U,j}^{(k)} = \mathbf{\Lambda}_{\lambda,j,:}^{zn(k)}\mathbf{b}^z + \mathbf{\Lambda}_{\lambda,j,:}^{za(k)}\mathbf{b}^z + \mathbf{\Lambda}_{\Delta,j,:}^{zn(k)}\mathbf{b}^{nx} + \mathbf{\Lambda}_{\lambda,j,:}^{ra(k)}\mathbf{b}^r + \mathbf{\Lambda}_{\Delta,j,:}^{ra(k)}\mathbf{b}^{na} + \sum_{i=1}^{s}(\mathbf{\Lambda}_{\varphi,j,i}^{zn(k)} + \mathbf{\Lambda}_{\varphi,j,i}^{za(k)} + \mathbf{\Lambda}_{\varphi,j,i}^{ra(k)}),$$

*and (*$\odot$ *is the Hadamard product)*

$$\mathbf{\Lambda}_{\lambda,j,:}^{zn(k)} = \begin{cases} \mathbf{W}_{j,:}^{Fa} \odot \lambda_{j,:}^{zn(k)} & \text{if } k = m; \\ \tilde{\mathbf{W}}_{U,j,:}^{a(k+1)} \odot \lambda_{j,:}^{zn(k)} & \text{if } k \in [m-1]; \end{cases} \quad \mathbf{\Lambda}_{\lambda,j,:}^{za(k)} = \begin{cases} \mathbf{W}_{j,:}^{Fa} \odot \lambda_{j,:}^{za(k)} & \text{if } k = m; \\ \tilde{\mathbf{W}}_{U,j,:}^{a(k+1)} \odot \lambda_{j,:}^{za(k)} & \text{if } k \in [m-1]; \end{cases}$$

$$\mathbf{\Lambda}_{\Delta,j,:}^{zn(k)} = \begin{cases} \mathbf{W}_{j,:}^{Fa} \odot \mathbf{\Delta}_{j,:}^{zn(k)} & \text{if } k = m; \\ \tilde{\mathbf{W}}_{U,j,:}^{a(k+1)} \odot \mathbf{\Delta}_{j,:}^{zn(k)} & \text{if } k \in [m-1]; \end{cases} \quad \mathbf{\Lambda}_{\Delta,j,:}^{za(k)} = \begin{cases} \mathbf{W}_{j,:}^{Fa} \odot \mathbf{\Delta}_{j,:}^{za(k)} & \text{if } k = m; \\ \tilde{\mathbf{W}}_{U,j,:}^{a(k+1)} \odot \mathbf{\Delta}_{j,:}^{za(k)} & \text{if } k \in [m-1]; \end{cases}$$

$$\mathbf{\Lambda}_{\varphi,j,:}^{zn(k)} = \begin{cases} \mathbf{W}_{j,:}^{Fa} \odot \varphi_{j,:}^{zn(k)} & \text{if } k = m; \\ \tilde{\mathbf{W}}_{U,j,:}^{a(k+1)} \odot \varphi_{j,:}^{zn(k)} & \text{if } k \in [m-1]; \end{cases} \quad \mathbf{\Lambda}_{\varphi,j,:}^{za(k)} = \begin{cases} \mathbf{W}_{j,:}^{Fa} \odot \varphi_{j,:}^{za(k)} & \text{if } k = m; \\ \tilde{\mathbf{W}}_{U,j,:}^{a(k+1)} \odot \varphi_{j,:}^{za(k)} & \text{if } k \in [m-1]; \end{cases}$$

$$\begin{aligned}
\mathbf{\Lambda}^{ra(k)}_{\lambda,j,:} &= \mathbf{\Lambda}^{zn(k)}_{\Delta,j,:} \odot \lambda^{ra(k)}_{j,:} \qquad && \textit{if} \quad k \in [m];\\
\mathbf{\Lambda}^{ra(k)}_{\Delta,j,:} &= \mathbf{\Lambda}^{zn(k)}_{\Delta,j,:} \odot \mathbf{\Delta}^{ra(k)}_{j,:} && \textit{if} \quad k \in [m];\\
\mathbf{\Lambda}^{ra(k)}_{\varphi,j,:} &= \mathbf{\Lambda}^{zn(k)}_{\Delta,j,:} \odot \varphi^{ra(k)}_{j,:} && \textit{if} \quad k \in [m];
\end{aligned}$$

*and* $\forall r \in s$,

$$\lambda^{zn(m)}_{j,r} = \begin{cases} \alpha^{zn(m)}_{U,r} & \textit{if } \mathbf{W}^{Fa}_{j,r} \geq 0; \\ \alpha^{zn(m)}_{L,r} & \textit{if } \mathbf{W}^{Fa}_{j,r} < 0; \end{cases} \quad \mathbf{\Delta}^{zn(m)}_{j,r} = \begin{cases} \beta^{zn(m)}_{U,r} & \textit{if } \mathbf{W}^{Fa}_{j,r} \geq 0; \\ \beta^{zn(m)}_{L,r} & \textit{if } \mathbf{W}^{Fa}_{j,r} < 0; \end{cases} \quad \varphi^{zn(m)}_{j,r} = \begin{cases} \gamma^{zn(m)}_{U,r} & \textit{if } \mathbf{W}^{Fa}_{j,r} \geq 0; \\ \gamma^{zn(m)}_{L,r} & \textit{if } \mathbf{W}^{Fa}_{j,r} < 0; \end{cases}$$

$$\lambda^{za(m)}_{j,r} = \begin{cases} \alpha^{za(m)}_{U,r} & \textit{if } \mathbf{W}^{Fa}_{j,r} \geq 0; \\ \alpha^{za(m)}_{L,r} & \textit{if } \mathbf{W}^{Fa}_{j,r} < 0; \end{cases} \quad \mathbf{\Delta}^{za(m)}_{j,r} = \begin{cases} \beta^{za(m)}_{U,r} & \textit{if } \mathbf{W}^{Fa}_{j,r} \geq 0; \\ \beta^{za(m)}_{L,r} & \textit{if } \mathbf{W}^{Fa}_{j,r} < 0; \end{cases} \quad \varphi^{za(m)}_{j,r} = \begin{cases} \gamma^{za(m)}_{U,r} & \textit{if } \mathbf{W}^{Fa}_{j,r} \geq 0; \\ \gamma^{za(m)}_{L,r} & \textit{if } \mathbf{W}^{Fa}_{j,r} < 0; \end{cases}$$

*and* $\forall r \in s, k \in [m-1]$,

$$\lambda^{zn(k)}_{j,r} = \begin{cases} \alpha^{zn(k)}_{U,r} & \textit{if} \quad \tilde{\mathbf{W}}^{a(k+1)}_{U,j,r} \geq 0; \\ \alpha^{zn(k)}_{L,r} & \textit{if} \quad \tilde{\mathbf{W}}^{a(k+1)}_{U,j,r} < 0; \end{cases} \quad \lambda^{za(k)}_{j,r} = \begin{cases} \alpha^{za(k)}_{U,r} & \textit{if} \quad \tilde{\mathbf{W}}^{a(k+1)}_{U,j,r} \geq 0; \\ \alpha^{za(k)}_{L,r} & \textit{if} \quad \tilde{\mathbf{W}}^{a(k+1)}_{U,j,r} < 0; \end{cases}$$

$$\mathbf{\Delta}^{zn(k)}_{j,r} = \begin{cases} \beta^{zn(k)}_{U,r} & \textit{if} \quad \tilde{\mathbf{W}}^{a(k+1)}_{U,j,r} \geq 0; \\ \beta^{zn(k)}_{L,r} & \textit{if} \quad \tilde{\mathbf{W}}^{a(k+1)}_{U,j,r} < 0; \end{cases} \quad \mathbf{\Delta}^{za(k)}_{j,r} = \begin{cases} \beta^{za(k)}_{U,r} & \textit{if} \quad \tilde{\mathbf{W}}^{a(k+1)}_{U,j,r} \geq 0; \\ \beta^{za(k)}_{L,r} & \textit{if} \quad \tilde{\mathbf{W}}^{a(k+1)}_{U,j,r} < 0; \end{cases}$$

$$\varphi^{zn(k)}_{j,r} = \begin{cases} \gamma^{zn(k)}_{U,r} & \textit{if} \quad \tilde{\mathbf{W}}^{a(k+1)}_{U,j,r} \geq 0; \\ \gamma^{zn(k)}_{L,r} & \textit{if} \quad \tilde{\mathbf{W}}^{a(k+1)}_{U,j,r} < 0; \end{cases} \quad \varphi^{za(k)}_{j,r} = \begin{cases} \gamma^{za(k)}_{U,r} & \textit{if} \quad \tilde{\mathbf{W}}^{a(k+1)}_{U,j,r} \geq 0; \\ \gamma^{za(k)}_{L,r} & \textit{if} \quad \tilde{\mathbf{W}}^{a(k+1)}_{U,j,r} < 0; \end{cases}$$

*and* $\forall r \in s, k \in [m]$,

$$\lambda^{ra(k)}_{j,r} = \begin{cases} \alpha^{ra(k)}_{U,r} & \textit{if} \quad \mathbf{\Lambda}^{zn(k)}_{\Delta,j,r} \geq 0; \\ \alpha^{ra(k)}_{L,r} & \textit{if} \quad \mathbf{\Lambda}^{zn(k)}_{\Delta,j,r} < 0; \end{cases}$$

$$\mathbf{\Delta}^{ra(k)}_{j,r} = \begin{cases} \beta^{ra(k)}_{U,r} & \textit{if} \quad \mathbf{\Lambda}^{zn(k)}_{\Delta,j,r} \geq 0; \\ \beta^{ra(k)}_{L,r} & \textit{if} \quad \mathbf{\Lambda}^{zn(k)}_{\Delta,j,r} < 0; \end{cases}$$

$$\varphi^{ra(k)}_{j,r} = \begin{cases} \gamma^{ra(k)}_{U,r} & \textit{if} \quad \mathbf{\Lambda}^{zn(k)}_{\Delta,j,r} \geq 0; \\ \gamma^{ra(k)}_{L,r} & \textit{if} \quad \mathbf{\Lambda}^{zn(k)}_{\Delta,j,r} < 0. \end{cases}$$

***Lower bound.*** *The above derivations of upper bound can be applied similarly to derive lower bounds of* $F_j(\mathbf{X})$*, and the only difference is now we need to use the left-hand side of inequities (rather than right-hand side when deriving upper bound) to bound the activated terms. Thus, following the same procedure in deriving the upper bounds, we can iteratively unwrap the activation functions and obtain a final lower bound* $F^{L,1}_j(\mathbf{X})$*, where* $F_j(\mathbf{X}) \geq F^{L,m}_j(\mathbf{X}) \geq \cdots \geq F^{L,1}_j(\mathbf{X})$*. We let* $F^{L}_j(\mathbf{X})$ *denote the final lower bound* $F^{L,1}_j(\mathbf{X})$*, and we have*

$$F^{L}_j(\mathbf{X}) = \tilde{\mathbf{W}}^{a(1)}_{L,j,:}\mathbf{a}^{(0)} + \sum_{k=1}^{m} \tilde{\mathbf{W}}^{x(k)}_{L,j,:}\mathbf{x}^{(k)} + \sum_{k=1}^{m} \tilde{\mathbf{b}}^{(k)}_{L,j} + \mathbf{b}^{F}_{j},$$

*where*

$$\begin{aligned}
\tilde{\mathbf{W}}^{x(k)}_{L,j,q_k} &= \mathbf{\Omega}^{zn(k)}_{\omega,j,:}\mathbf{W}^{zx}_{:,q_k} + \mathbf{\Omega}^{za(k)}_{\omega,j,:}\mathbf{W}^{zx}_{:,q_k} + \mathbf{\Omega}^{zn(k)}_{\Theta,j,:}\mathbf{W}^{nx}_{:,q_k} + \mathbf{\Omega}^{ra(k)}_{\omega,j,:}\mathbf{W}^{rx}_{:,q_k},\\
\tilde{\mathbf{W}}^{a(k)}_{L,j,r} &= \mathbf{\Omega}^{zn(k)}_{\omega,j,:}\mathbf{W}^{za}_{:,r} + \mathbf{\Omega}^{za(k)}_{\omega,j,:}\mathbf{W}^{za}_{:,r} + \mathbf{\Omega}^{za(k)}_{\Theta,j,r} + \mathbf{\Omega}^{ra(k)}_{\omega,j,:}\mathbf{W}^{ra}_{:,r} + \mathbf{\Omega}^{ra(k)}_{\Theta,j,:}\mathbf{W}^{na}_{:,r},\\
\tilde{\mathbf{b}}^{(k)}_{L,j} &= \mathbf{\Omega}^{zn(k)}_{\omega,j,:}\mathbf{b}^{z} + \mathbf{\Omega}^{za(k)}_{\omega,j,:}\mathbf{b}^{z} + \mathbf{\Omega}^{zn(k)}_{\Theta,j,:}\mathbf{b}^{nx} + \mathbf{\Omega}^{ra(k)}_{\omega,j,:}\mathbf{b}^{r} + \mathbf{\Omega}^{ra(k)}_{\Theta,j,:}\mathbf{b}^{na} + \sum_{i=1}^{s}(\mathbf{\Omega}^{zn(k)}_{\psi,j,i} + \mathbf{\Omega}^{za(k)}_{\psi,j,i} + \mathbf{\Omega}^{ra(k)}_{\psi,j,i}),
\end{aligned}$$

*and ($\odot$ is the Hadamard product)*

$$\mathbf{\Omega}^{zn(k)}_{\omega,j,:} = \begin{cases} \mathbf{W}^{Fa}_{j,:} \odot \omega^{zn(k)}_{j,:} & \textit{if} \quad k = m; \\ \tilde{\mathbf{W}}^{a(k+1)}_{L,j,:} \odot \omega^{zn(k)}_{j,:} & \textit{if} \quad k \in [m-1]; \end{cases} \quad \mathbf{\Omega}^{za(k)}_{\omega,j,:} = \begin{cases} \mathbf{W}^{Fa}_{j,:} \odot \omega^{za(k)}_{j,:} & \textit{if} \quad k = m; \\ \tilde{\mathbf{W}}^{a(k+1)}_{L,j,:} \odot \omega^{za(k)}_{j,:} & \textit{if} \quad k \in [m-1]; \end{cases}$$

$$\mathbf{\Omega}^{zn(k)}_{\Theta,j,:} = \begin{cases} \mathbf{W}^{Fa}_{j,:} \odot \mathbf{\Theta}^{zn(k)}_{j,:} & \textit{if} \quad k = m; \\ \tilde{\mathbf{W}}^{a(k+1)}_{L,j,:} \odot \mathbf{\Theta}^{zn(k)}_{j,:} & \textit{if} \quad k \in [m-1]; \end{cases} \quad \mathbf{\Omega}^{za(k)}_{\Theta,j,:} = \begin{cases} \mathbf{W}^{Fa}_{j,:} \odot \mathbf{\Theta}^{za(k)}_{j,:} & \textit{if} \quad k = m; \\ \tilde{\mathbf{W}}^{a(k+1)}_{L,j,:} \odot \mathbf{\Theta}^{za(k)}_{j,:} & \textit{if} \quad k \in [m-1]; \end{cases}$$

$$\mathbf{\Omega}^{zn(k)}_{\psi,j,:} = \begin{cases} \mathbf{W}^{Fa}_{j,:} \odot \psi^{zn(k)}_{j,:} & \textit{if} \quad k = m; \\ \tilde{\mathbf{W}}^{a(k+1)}_{L,j,:} \odot \psi^{zn(k)}_{j,:} & \textit{if} \quad k \in [m-1]; \end{cases} \quad \mathbf{\Omega}^{za(k)}_{\psi,j,:} = \begin{cases} \mathbf{W}^{Fa}_{j,:} \odot \psi^{za(k)}_{j,:} & \textit{if} \quad k = m; \\ \tilde{\mathbf{W}}^{a(k+1)}_{L,j,:} \odot \psi^{za(k)}_{j,:} & \textit{if} \quad k \in [m-1]; \end{cases}$$

$$\begin{aligned} \mathbf{\Omega}^{ra(k)}_{\omega,j,:} &= \mathbf{\Omega}^{zn(k)}_{\Theta,j,:} \odot \omega^{ra(k)}_{j,:} & \textit{if} \quad k \in [m]; \\ \mathbf{\Omega}^{ra(k)}_{\Theta,j,:} &= \mathbf{\Omega}^{zn(k)}_{\Theta,j,:} \odot \mathbf{\Theta}^{ra(k)}_{j,:} & \textit{if} \quad k \in [m]; \\ \mathbf{\Omega}^{ra(k)}_{\psi,j,:} &= \mathbf{\Omega}^{zn(k)}_{\Theta,j,:} \odot \psi^{ra(k)}_{j,:} & \textit{if} \quad k \in [m]; \end{aligned}$$

*and* $\forall r \in s$,

$$\omega^{zn(m)}_{j,r} = \begin{cases} \alpha^{zn(m)}_{L,r} & \textit{if} \ \mathbf{W}^{Fa}_{j,r} \geq 0; \\ \alpha^{zn(m)}_{U,r} & \textit{if} \ \mathbf{W}^{Fa}_{j,r} < 0; \end{cases} \quad \mathbf{\Theta}^{zn(m)}_{j,r} = \begin{cases} \beta^{zn(m)}_{L,r} & \textit{if} \ \mathbf{W}^{Fa}_{j,r} \geq 0; \\ \beta^{zn(m)}_{U,r} & \textit{if} \ \mathbf{W}^{Fa}_{j,r} < 0; \end{cases} \quad \psi^{zn(m)}_{j,r} = \begin{cases} \gamma^{zn(m)}_{L,r} & \textit{if} \ \mathbf{W}^{Fa}_{j,r} \geq 0; \\ \gamma^{zn(m)}_{U,r} & \textit{if} \ \mathbf{W}^{Fa}_{j,r} < 0; \end{cases}$$

$$\omega^{za(m)}_{j,r} = \begin{cases} \alpha^{za(m)}_{L,r} & \textit{if} \ \mathbf{W}^{Fa}_{j,r} \geq 0; \\ \alpha^{za(m)}_{U,r} & \textit{if} \ \mathbf{W}^{Fa}_{j,r} < 0; \end{cases} \quad \mathbf{\Theta}^{za(m)}_{j,r} = \begin{cases} \beta^{za(m)}_{L,r} & \textit{if} \ \mathbf{W}^{Fa}_{j,r} \geq 0; \\ \beta^{za(m)}_{U,r} & \textit{if} \ \mathbf{W}^{Fa}_{j,r} < 0; \end{cases} \quad \psi^{za(m)}_{j,r} = \begin{cases} \gamma^{za(m)}_{L,r} & \textit{if} \ \mathbf{W}^{Fa}_{j,r} \geq 0; \\ \gamma^{za(m)}_{U,r} & \textit{if} \ \mathbf{W}^{Fa}_{j,r} < 0; \end{cases}$$

*and* $\forall r \in s, k \in [m-1]$,

$$\omega^{zn(k)}_{j,r} = \begin{cases} \alpha^{zn(k)}_{L,r} & \textit{if} \quad \tilde{\mathbf{W}}^{a(k+1)}_{L,j,r} \geq 0; \\ \alpha^{zn(k)}_{U,r} & \textit{if} \quad \tilde{\mathbf{W}}^{a(k+1)}_{L,j,r} < 0; \end{cases} \quad \omega^{za(k)}_{j,r} = \begin{cases} \alpha^{za(k)}_{L,r} & \textit{if} \quad \tilde{\mathbf{W}}^{a(k+1)}_{L,j,r} \geq 0; \\ \alpha^{za(k)}_{U,r} & \textit{if} \quad \tilde{\mathbf{W}}^{a(k+1)}_{L,j,r} < 0; \end{cases}$$

$$\mathbf{\Theta}^{zn(k)}_{j,r} = \begin{cases} \beta^{zn(k)}_{L,r} & \textit{if} \quad \tilde{\mathbf{W}}^{a(k+1)}_{L,j,r} \geq 0; \\ \beta^{zn(k)}_{U,r} & \textit{if} \quad \tilde{\mathbf{W}}^{a(k+1)}_{L,j,r} < 0; \end{cases} \quad \mathbf{\Theta}^{zn(k)}_{j,r} = \begin{cases} \beta^{zn(k)}_{L,r} & \textit{if} \quad \tilde{\mathbf{W}}^{a(k+1)}_{L,j,r} \geq 0; \\ \beta^{zn(k)}_{U,r} & \textit{if} \quad \tilde{\mathbf{W}}^{a(k+1)}_{L,j,r} < 0; \end{cases}$$

$$\psi^{zn(k)}_{j,r} = \begin{cases} \gamma^{zn(k)}_{L,r} & \textit{if} \quad \tilde{\mathbf{W}}^{a(k+1)}_{L,j,r} \geq 0; \\ \gamma^{zn(k)}_{U,r} & \textit{if} \quad \tilde{\mathbf{W}}^{a(k+1)}_{L,j,r} < 0; \end{cases} \quad \psi^{za(k)}_{j,r} = \begin{cases} \gamma^{za(k)}_{L,r} & \textit{if} \quad \tilde{\mathbf{W}}^{a(k+1)}_{L,j,r} \geq 0; \\ \gamma^{za(k)}_{U,r} & \textit{if} \quad \tilde{\mathbf{W}}^{a(k+1)}_{L,j,r} < 0; \end{cases}$$

*and* $\forall r \in s, k \in [m]$,

$$\omega^{ra(k)}_{j,r} = \begin{cases} \alpha^{ra(k)}_{L,r} & \textit{if} \quad \mathbf{\Omega}^{zn(k)}_{\Theta,j,r} \geq 0; \\ \alpha^{ra(k)}_{U,r} & \textit{if} \quad \mathbf{\Omega}^{zn(k)}_{\Theta,j,r} < 0; \end{cases}$$

$$\mathbf{\Theta}^{ra(k)}_{j,r} = \begin{cases} \beta^{ra(k)}_{L,r} & \textit{if} \quad \mathbf{\Omega}^{zn(k)}_{\Theta,j,r} \geq 0; \\ \beta^{ra(k)}_{U,r} & \textit{if} \quad \mathbf{\Omega}^{zn(k)}_{\Theta,j,r} < 0; \end{cases}$$

$$\psi^{ra(k)}_{j,r} = \begin{cases} \gamma^{ra(k)}_{L,r} & \textit{if} \quad \mathbf{\Omega}^{zn(k)}_{\Theta,j,r} \geq 0; \\ \gamma^{ra(k)}_{U,r} & \textit{if} \quad \mathbf{\Omega}^{zn(k)}_{\Theta,j,r} < 0. \end{cases}$$

**Corollary A. 5 (Closed-form global bounds)** *Given data $\mathbf{X} \in \mathbb{R}^{n \times m}$, $l_p$ ball parameters $p \geq 1$ and $\epsilon \geq 0$. For an $m$-layer gated recurrent unit network $F : \mathbb{R}^{n \times m} \to \mathbb{R}^t$, there exists two fixed values $\gamma^L_j$ and $\gamma^U_j$ such that $\forall \mathbf{X} \in \mathbb{R}^{n \times m}$ where $\mathbf{x}^{(k)} \in \mathbb{B}_p(\mathbf{x}^{(k)}_0, \epsilon)$, and $\forall j \in [t]$, $1/q = 1 - 1/p$, the inequity $\gamma^L_j \leq F_j(\mathbf{X}) \leq \gamma^U_j$ holds true, where*

$$\begin{aligned} \gamma^U_j &= \tilde{\mathbf{W}}^{a(1)}_{U,j,:}\mathbf{a}^{(0)} + \sum_{k=1}^{m} \epsilon \|\tilde{\mathbf{W}}^{x(k)}_{U,j,:}\|_q + \sum_{k=1}^{m} \tilde{\mathbf{W}}^{x(k)}_{U,j,:}\mathbf{x}^{(k)}_0 + \sum_{k=1}^{m} \tilde{\mathbf{b}}^{(k)}_{U,j} + \mathbf{b}^F_j, \\ \gamma^L_j &= \tilde{\mathbf{W}}^{a(1)}_{L,j,:}\mathbf{a}^{(0)} - \sum_{k=1}^{m} \epsilon \|\tilde{\mathbf{W}}^{x(k)}_{L,j,:}\|_q + \sum_{k=1}^{m} \tilde{\mathbf{W}}^{x(k)}_{L,j,:}\mathbf{x}^{(k)}_0 + \sum_{k=1}^{m} \tilde{\mathbf{b}}^{(k)}_{L,j} + \mathbf{b}^F_j. \end{aligned}$$

**Corollary A. 6 (Pre-activation bounds in GRUs)** *The pre-activation bounds of different gates can be obtained via simple modifications from Theorem A.6. Specifically, we recall the definitions of pre-activations in different gates:*

$$\begin{aligned}
\textit{Reset gate:}\quad & \mathbf{y}^{r(k)} = \underline{\mathbf{W}^{rx}\mathbf{x}^{(k)}} + \mathbf{W}^{ra}\mathbf{a}^{(k-1)} + \mathbf{b}^{r}; \\
\textit{Update gate:}\quad & \mathbf{y}^{z(k)} = \underline{\mathbf{W}^{zx}\mathbf{x}^{(k)}} + \mathbf{W}^{za}\mathbf{a}^{(k-1)} + \mathbf{b}^{z}; \\
\textit{New gate:}\quad & \mathbf{y}^{n(k)} = \underline{\mathbf{W}^{nx}\mathbf{x}^{(k)}} + \mathbf{b}^{nx} + \mathbf{r}^{(k)} \odot (\mathbf{W}^{na}\mathbf{a}^{(k-1)} + \mathbf{b}^{na}).
\end{aligned}$$

*For a given GRU and input $\mathbf{X}_0$, the underlined part of the equations are bounded by*

$$\mathbf{W}^{gate}\mathbf{x}_0^{(k)} - \epsilon\|\mathbf{W}^{gate}\|_q \leq \mathbf{W}^{gate}\mathbf{x}^{(k)} \leq \mathbf{W}^{gate}\mathbf{x}_0^{(k)} + \epsilon\|\mathbf{W}^{gate}\|_q,$$

*where gate = $\{rx, zx, nx\}$. Thus to derive pre-activation bounds, we only need to know the ranges of remaining parts in the equations above. These can be computed by replacing the output mapping $\mathbf{W}^{Fa}$ in Theorem A.6 by $\mathbf{W}^{ra}, \mathbf{W}^{za}, \mathbf{W}^{na}$, respectively. The output bias $\mathbf{b}^{F}$ is correspondingly substituted with $\mathbf{b}^{r}, \mathbf{b}^{z}, \mathbf{b}^{na}$. For example, to derive the bounds for pre-activation bounds of reset gates, we replace the output mapping matrix and bias from $\mathbf{W}^{Fa}$ and $\mathbf{b}^{F}$ by $\mathbf{W}^{ra}$and $\mathbf{b}^{r}$. For the pre-activation bound of new gate, we need to first derive the bound of reset gate. Considering that there is a cross-nonlinear term of reset gate and the previous hidden state, therefore we need to further use 2D bounding planes as introduced in Section 3.2 to bound the term. Lastly, the pre-activation bound is found by combining the linear bounds with $\mathbf{W}^{nx}\mathbf{x}_0^{(k)} \pm \epsilon\|\mathbf{W}^{nx}\|_q + \mathbf{b}^{nx}$.*

## B. Experiments

### B.1 Significance of plane (2D)-bounding POPQORN certificates

Recalling that when analyzing the bounds for an LSTM, we extend the ideas of bounding lines to bounding planes. In what follows, as proofs and formulas for POPQORN certificates with both 2D bounding planes (A.3) and 1D bounding lines (A.6) are provided, we justify our proposals of using 2D bounding planes instead of 1D or even constant bounding[2] alternatives from two angles:

1. In Experiment (I) - MNIST handwritten digit classification task, constant and 1D bounding approaches give much smaller (3-6 times smaller for 4-slice) certificates than those obtained by 2D bounding, and they become even looser as the LSTM goes deeper (400-3000 times smaller for 14-slice). Specifically,

   - LSTM 4-slice: average bound for (2D, 1D, constant) bound = (0.232, 0.071, 0.041)
   - LSTM 7-slice: average bound for (2D, 1D, constant) bound = (0.140, 0.015, 0.012)
   - LSTM 14-slice: average bound for (2D, 1D, constant) bound = (0.059, 1.5e-4, 2e-5)

2. In Experiment (III) - question classification task, robustness bounds obtained are only meaningful when the bounds are large enough to cover word pairs in the word embedding space. Here, we show that the robustness certificates obtained via constant and 1D bounding contain significantly fewer word embeddings compared with the proposed 2D bounding. Specifically, we use 2 different groups of word embeddings in a length-10K vocabulary and show that our 2D bounding technique indeed contains non-trivial numbers (19, 535635) of word embedding pairs for the 1st LSTM and the 2nd LSTM. Meanwhile, 1D and constant bounding have issues of robustness certificates being smaller than the minimum distance of word embeddings (MDWE), where their certificates contain (9, 0) and (0, 0) word embedding pairs.

   - LSTM 1: MDWE = 0.120, average bound for (2D, 1D, constant) bound = (0.138,0.067,0.039)
   - LSTM 2: MDWE = 0.012, average bound for (2D, 1D, constant) bound = (0.027,0.013,0.008)

The above results demonstrate the necessity and significance of the proposed 2D gate-bounding planes, in order to obtain *non-trivial* robustness certificates.

[2]Modifying the results of 2D and 1D bounding to constant bounding means that pre-activation bounds are directly combined and considered when evaluating ranges of activated states. This is rather a trivial implementation, whose details are therefore omitted herein.

### B.2 CLEVER-RNN Score

Assume for a given data sequence $\mathbf{X}$, $j$ is the true label, and $i$ is the target label. Let $g(\mathbf{X}) = F_j(\mathbf{X}) - F_i(\mathbf{X})$, is a Lipshiz function that has the property below:

$$
\begin{aligned}
|g(\mathbf{X}) - g(\mathbf{Y})| &= |g(\mathbf{x}^{(1)}, \mathbf{x}^{(2)}, \ldots, \mathbf{x}^{(m)}) - g(\mathbf{y}^{(1)}, \mathbf{y}^{(2)}, \ldots, \mathbf{y}^{(m)})| \\
&\leq \sum_{t=1}^{m} L_q^t \|\mathbf{x}^{(t)} - \mathbf{y}^t\|_p,
\end{aligned}
$$

where $L_q^t = \max\{\|\nabla_t g(\mathbf{X})\|_q : \mathbf{x}^{(k)} \in \mathbb{B}_p(\mathbf{x}_0^{(k)}, \epsilon_0), \forall k \in [m]\}$ and $\nabla_t g(\mathbf{X}) = (\frac{\partial g(\mathbf{X})}{\partial \mathbf{x}_1^{(t)}}, \ldots, \frac{\partial g(\mathbf{X})}{\partial \mathbf{x}_n^{(t)}})^T$. We then have

$$
|g(\mathbf{X}) - g(\mathbf{X}_0)| \leq \sum_{t=1}^{m} L_q^t \|\mathbf{x}^{(t)} - \mathbf{x}_0^t\|_p,
$$

which can be rearranged into the following form

$$
g(\mathbf{X}_0) - \sum_{t=1}^{m} L_q^t \|\mathbf{x}^{(t)} - \mathbf{x}_0^t\|_p \leq g(\mathbf{X}) \leq g(\mathbf{X}_0) + \sum_{t=1}^{m} L_q^t \|\mathbf{x}^{(t)} - \mathbf{x}_0^t\|_p.
$$

Recalling that $g(\mathbf{X}) = 0$ when $F_j(\mathbf{X}) = F_i(\mathbf{X})$, which indicates an adversarial example is found. That is to say, we want to ensure $g(\mathbf{X}) \geq 0$. This is assured by utilizing its lower bound:

$$
g(\mathbf{X}_0) - \sum_{t=1}^{m} L_q^t \|\mathbf{x}^{(t)} - \mathbf{x}_0^t\|_p \geq 0 \Rightarrow \epsilon = \|\mathbf{x}^{(t)} - \mathbf{x}_0^t\|_p \leq \frac{g(\mathbf{X}_0)}{\sum_{t=1}^{m} L_q^t}.
$$

In summary, CLEVER-Ada score is given as $\epsilon = \min\{\frac{g(\mathbf{X}_0)}{\sum_{t=1}^{m} L_q^t}, \epsilon_0\}$.

### B.3 Adapted C&W Attack

In the original C&W attack, the loss function is designed with a loss function as *loss* $= c * q + \|\mathbf{X} - \mathbf{X}_0\|_p$, where $q = \max(\max_{j \neq i}(F_j(\mathbf{X}) - F_i(\mathbf{X})), 0)$ and $c$ is a positive constant. In practice, we use binary search procedure to find a $c$ such that an attack is obtained with a small magnitude. In essence, this corresponds to finding a targeted attack for class $i$, and the perturbation is measured by computing the norm of difference between $\mathbf{X}$ and $\mathbf{X}_0$. Here, we adapt the loss function to be *loss* $= q + (v + c) * \max_k \|\mathbf{x}^{(k)} - \mathbf{x}_0^{(k)}\|_p$, where $q = \max(F_j(\mathbf{X}) - F_i(\mathbf{X}), 0)$ and $v$ is defined by indicator function $\mathbb{1}_{q \leq 0}(q)$. In our formulation, the $c$ is a pre-defined small constant, which does not update during the process. More concretely, C&W-Ada puts higher weights on minimizing the $q$ until an attack is found, and prioritizes the minimization of distortion magnitude when an attack has been found ($q = 0$, $v = 1$). We use the maximum perturbation of all frames as the C&W score.

### B.4 Experimental Details

We evaluate POPQORN and other baselines on vanilla RNNs and LSTMs trained on MNIST dataset, MNIST sequence dataset, and Classifier for the question classification (UIUC's CogComp QC) Dataset. We train vanilla RNN and LSTM models on MNIST dataset, and evaluate by randomly selecting 1000 test images as samples. For these 1000 test images, we randomly generate a set of adversarial target labels, and compute their average targeted POPQORN bounds (the true label output is only guaranteed to be bigger than the target label output) and standard deviation, CLEVER-RNN scores, and compare them with the magnitude of attacks found by C&W-Ada. Different from MNIST dataset, MNIST sequence dataset records handwritten numbers as sequential data of line segment sequences. Due to the poor performance of vanilla RNNs on MNIST sequence dataset, only LSTM classifiers are trained for robustness evaluations. In this example, we compute the untargeted POPQORN bound on only one single stroke of a digit sequence. After calculating bounds of all strokes, we can identify the strokes with minimal bounds in a digit sequence. We call the strokes *sensitive strokes*. Question classification task is to classify a question into several pre-defined categories. For example, *"What is a mirror made out of?"* corresponds to *"ENTY"* (entity), *"What is the temperature at the center of the earth?"* corresponds to *"NUM"* (number), *"What is the abbreviation for Texas?"* corresponds to *"ABBR"* (abbreviation), *"Who discovered x-rays?"* corresponds to *"HUM"* (human), *"What is the capital of Yugoslavia?"* corresponds to *"LOC"* (location), and *"What is caffeine?"* corresponds to *"DESC"* (description). In this example, we also compute the untargeted POPQORN bound on one single input frame, and call the words with minimal bounds *sensitive words*.

**Word embedding is used in question classifications.** In the task of certifying bounds for question classification networks, we study how much we can perturb a single frame in a sequence while not causing any misclassification. However, different from the former tasks, the space of words is discrete. Thus instead of dealing with words in a discrete space, we evaluate their word embedding. Specifically, we use pretrained word embedding from "glove.6B.100d"[3].

**Additional NLP Experiment: News Title Classification.** We further exemplify the usefulness of POPQORN by identifying key words (quantifying robustness) for TagMyNews [1] LSTMs. TagMyNews is a dataset consisting of 32,567 English news items grouped into 7 categories: Sport, Business, U.S., Health, Sci&Tech, World, and Entertainment. Each news item has a news title and a short description. We train an LSTM to classify the news items into the 7 categories according to their news titles. Then we use POPQORN to identify keywords in the news titles by selecting the words with the smallest POPQORN robustness quantification. Three examples are given in Figure 3, where we can see that the keywords (underlined) identified by POPQORN are indeed more closely tied to the category of each news.

| Example | Samsung | to | launch | galaxy | s | sequel | In | south | korea | in | late | april |
|---|---|---|---|---|---|---|---|---|---|---|---|---|
| Sci&Tech | 0.4219 | 0.7344 | 0.5469 | 0.4648 | 0.5234 | 0.5664 | 0.8047 | 0.6641 | 0.6680 | 0.8516 | 0.7188 | 0.8125 |

| Example | 3 | journalists | kidnapped | in | afghanistan | are | set | free |
|---|---|---|---|---|---|---|---|---|
| World | 0.4492 | 0.4258 | 0.4219 | 0.7305 | 0.3945 | 0.6484 | 0.5977 | 0.5547 |

| Example | actress | evan | rachel | wood | dates | both | men | and | women |
|---|---|---|---|---|---|---|---|---|---|
| Entertain ment | 0.4062 | 0.3906 | 0.4609 | 0.4805 | 0.6211 | 0.6875 | 0.9688 | 1.0625 | 0.8672 |

Figure 3: Three examples in the news title classification task. The upper row gives the sample sentence; the lower row shows the POPQORN (2-norm) lower bounds of individual words. "Sci&Tech", "World", and "Entertainment" are the corresponding categories these news belong to.

[3]https://nlp.stanford.edu/projects/glove/

# References

[1] D. Vitale, P. Ferragina, and U. Scaiella. Classification of short texts by deploying topical annotations. In *Advances in Information Retrieval*, pages 376–387, 2012.
